# Supplementary material for: The sign problem in full configuration interaction quantum Monte Carlo: Linear and sub-linear representation regimes for the exact wave function
Source: arXiv:1407.4800 ancillary file (2014-07-17)
Supplement: Supplementary file 1 [file sm1.pdf]

# Supplementary material for "The sign problem in full configuration interaction quantum Monte Carlo: Linear and sub-linear representation regimes for the exact wave function"

James J. Shepherd[(a)], Gustavo E. Scuseria[(a)], and James S. Spencer[(b)]
[(a)] *Department of Chemistry and Department of Physics and Astronomy, Rice University, Houston, TX 77005-1892*
[(b)] *Department of Materials, Imperial College London, Exhibition Road, London, SW7 2AZ, U.K. and Department of Physics, Imperial College London, Exhibition Road, London, SW7 2AZ, U.K.*

We consider a set of 1D one-band Hubbard models for $U = 0.5,\ 0.75,\ 1.0,\ 2.0,\ 4.0,\ 8.0$ with $N_s = 12,\ 14,\ 16,\ 18,\ 20,\ 22$ sites per simulation cell and with an even number of electrons, $N_{\text{elec}}$, in the range $[4, 2N_s - 4]$. Not all combinations are presented here; in particular we do not include results at $U > 2.0$ and large $N_s$ close to half-filling; such systems have large Hilbert spaces and we estimate these plateaus to be larger than the maximum walker count we used ($10^7$). Further, the trend of the plateau with Hilbert space is well established for these values of $U$. We consider only spin-unpolarized systems and use momentum symmetry to reduce the size of the accessible Hilbert space; only determinants with total momentum of 0 ($\pi/2$) are considered for $N_{\text{elec}} = 4i + 2$ ($N_{\text{elec}} = 4i$), where $i = 0, 1, \ldots$. Preliminary calculations indicate that the plateau in the Hubbard models considered here are somewhat insensitive to the symmetry of the underlying wavefunction. The remaining calculation parameters are identical for all calculations: a time step of $\tau = 0.001$ and the shift was set to the energy of the restricted Hartree–Fock determinant. All calculations were run using the HANDE QMC code. Raw input and output files are available from Ref. 1. We encourage the community to use this data set as a starting point for comparing FCIQMC and related methods. By way of a starting point and as an example, we have, using a 'clean room' approach, verified our results by running a new set of calculations and processing the data with a different set of analysis tools [2].

Finding the plateau by taking the histogram of the population is complicated by the exponential population growth either side of the plateau. Hence if the simulation reaches a population substantially above the plateau, the histogram would be weighted to the large population limit and the plateau signal would be hard to detect. We largely overcome this by considering the histogram of the logarithm of the population. The plateau is then taken to be the bin of the histogram in which the most samples in imaginary time occur. This was used by one of us (JJS), although not described, in a prior study [3].

Here we plot the population dynamics from multiple trajectories for each system for which we found a plateau, thus providing visual validation. This was very important to our methodology, in particular in detecting systematic defects in the histogramming algorithm. We note in passing that we do not intend to mention that this is a black box method for plateau height determination. However, it is semi-automatic and has aided us in contracting the data set here. Plots below are ordered (small to large) by U and then by the size of the (accessible) Hilbert space, which is calculated by a Monte Carlo method.

In each plot below:

- blue lines show the total population of individual trajectories (i.e. individual simulations started using different random number seeds and hence following different Markov chains);
- green lines show the Hartree–Fock population;
- the dashed black line shows the first point at which the walker population contains 100 walkers on the restricted Hartree–Fock determinant;
- the horitzonal red line shows the plateau height as determined by histogramming;
- the shaded red region indicates the error on the estimate of the plateau height, determined by averaging over seeds;
- The plateau population, $N_{\text{plat}}$, is quoted with a estimate of the error as a fraction of $N_{\text{plat}}$;
- Unless detailed below, a bin width of $12500/N_{\text{data}}^2$, where $N_{\text{data}}$ is the number of data points, was used to histogram the logarithm of the walker population.

Various data files required alteration of the algorithmic determination of the plateau. In particular, the bin width was difficult to optimize. This was typically reflected in the standard deviations, and those where the plateau was smaller than two standard deviations were unreliably estimated. We manually measured the plateaus where the error exceeded 30% of the plateau height; we estimate the error due to measurement by hand to be around 10% where the histogram estimate still remains useful to guide the eye.

[1] http://dx.doi.org/10.6084/m9.figshare.1101537 (2014), in preparation; http://dx.doi.org/10.6084/m9.figshare.1096136 (2014), in preparation.

[2] http://dx.doi.org/10.6084/m9.figshare.1106864 (2014), in preparation.

[3] J. J. Shepherd, L. R. Schwarz, R. E. Thomas, G. H. Booth, D. Frenkel, and A. Alavi, *Emergence of Critical Phenomena in Full Configuration Interaction Quantum Monte Carlo*, arXiv e-print 1209.4023 (2012).

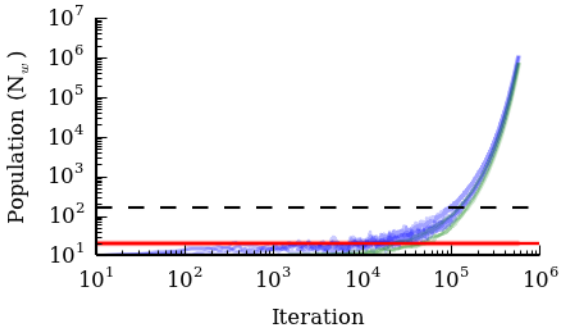


FIG. 1. $U = 0.5$, $N_{\rm dets} = 3.7e{+}02$ (12 sites, 4 electrons), $N_{\rm plat} = 20.3 \pm 9.2$ %

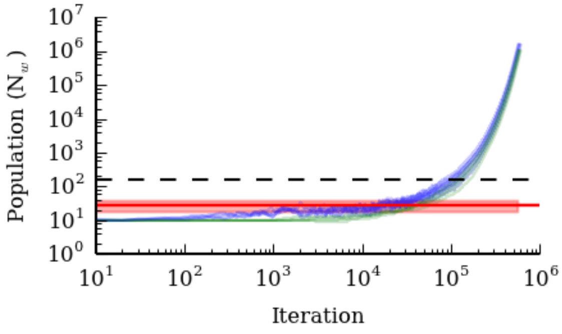


FIG. 2. $U = 0.5$, $N_{\rm dets} = 3.7e{+}02$ (12 sites, 20 electrons), $N_{\rm plat} = 27.6 \pm 36$ % (manual correction: 20)

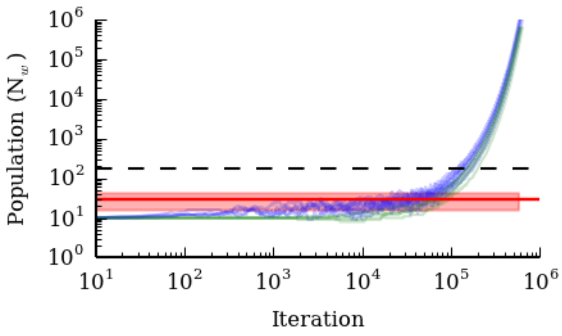


FIG. 3. $U = 0.5$, $N_{\rm dets} = 6e{+}02$ (14 sites, 4 electrons), $N_{\rm plat} = 28.6 \pm 45$ % (manual correction: 20)

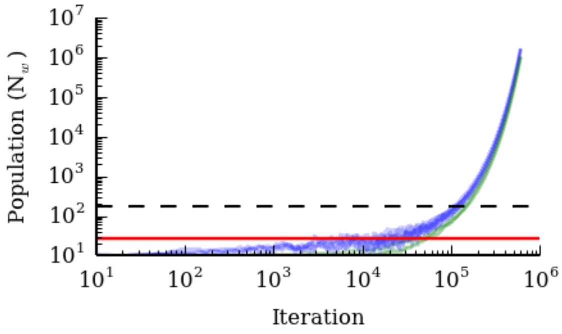


FIG. 4. $U = 0.5$, $N_{\rm dets} = 6e{+}02$ (14 sites, 24 electrons), $N_{\rm plat} = 27.1 \pm 0.23$ %

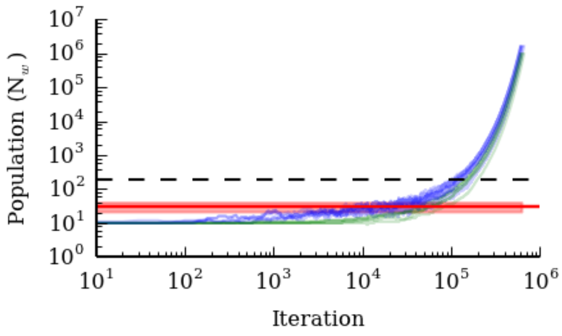


FIG. 5. $U = 0.5$, $N_{\rm dets} = 9e{+}02$ (16 sites, 28 electrons), $N_{\rm plat} = 30.2 \pm 31$ % (manual correction: 20)

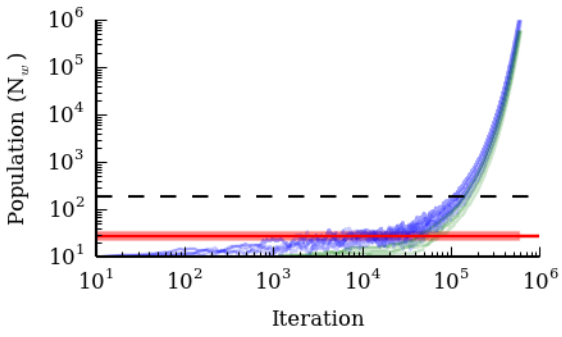


FIG. 6. $U = 0.5$, $N_{\rm dets} = 9e{+}02$ (16 sites, 4 electrons), $N_{\rm plat} = 28.3 \pm 18$ %

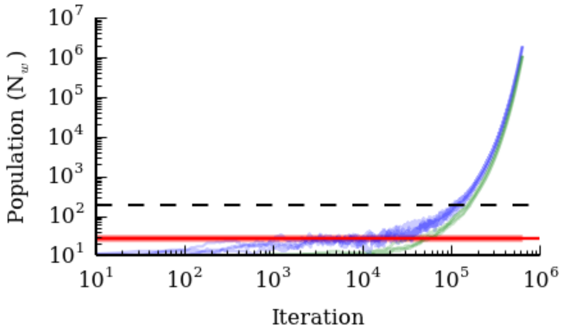


FIG. 7. $U$ = 0.5, $N_{\mathrm{dets}}$ = 1.3e+03 (18 sites, 32 electrons), $N_{\mathrm{plat}}$ = 27.2 ± 15 %

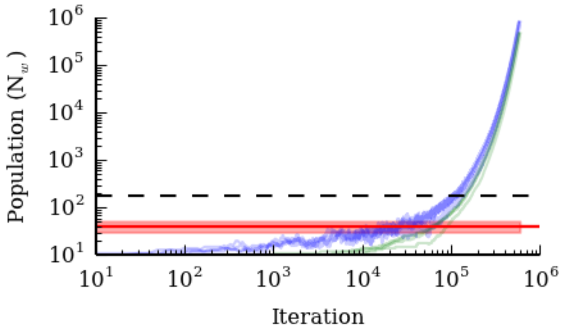


FIG. 8. $U = 0.5$, $N_{\mathrm{dets}} = 1.3\mathrm{e}{+}03$ (18 sites, 4 electrons), $N_{\mathrm{plat}}$ = 39.9 ± 26 %

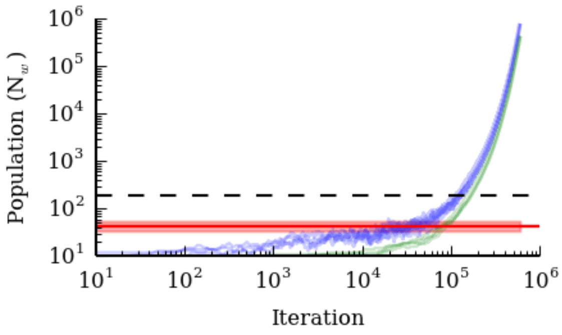


FIG. 9. $U = 0.5$, $N_{\mathrm{dets}} = 1.8\mathrm{e}{+}03$ (20 sites, 4 electrons), $N_{\mathrm{plat}}$ = 42.8 ± 23 %

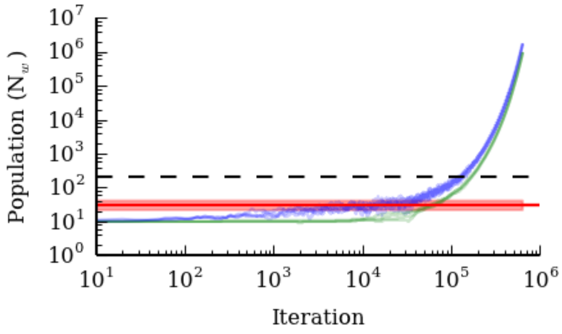


FIG. 10. $U$ = 0.5, $N_{\mathrm{dets}}$ = 1.8e+03 (20 sites, 36 electrons), $N_{\mathrm{plat}}$ = 31.6 ± 30 % (manual correction: 30)

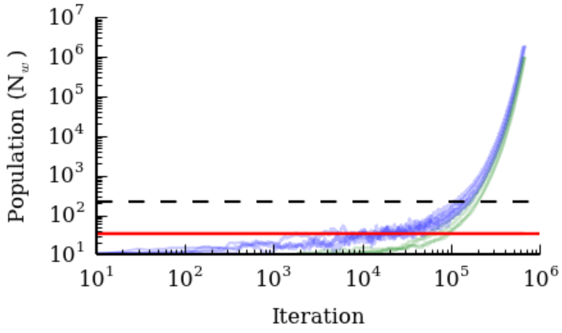


FIG. 11. $U$ = 0.5, $N_{\mathrm{dets}}$ = 2.4e+03 (22 sites, 40 electrons), $N_{\mathrm{plat}}$ = 34.4 ± 1.9 %

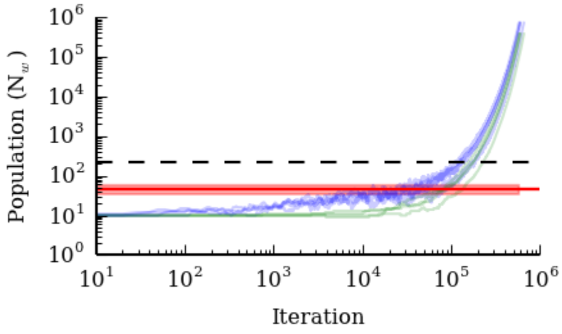


FIG. 12. $U$ = 0.5, $N_{\mathrm{dets}}$ = 2.4e+03 (22 sites, 4 electrons), $N_{\mathrm{plat}}$ = 46.2 ± 26 %

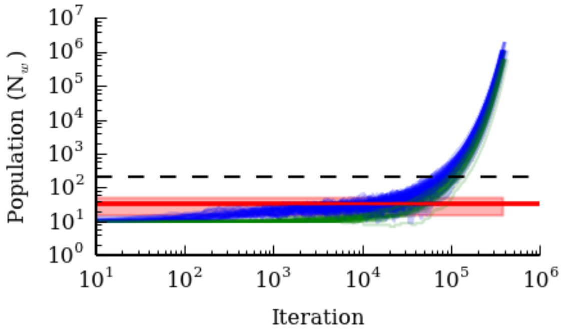


FIG. 13. $U = 0.5$, $N_{\text{dets}} = 4\text{e}{+}03$ (12 sites, 6 electrons), $N_{\text{plat}} = 32.5 \pm 53$ % (manual correction: 30)

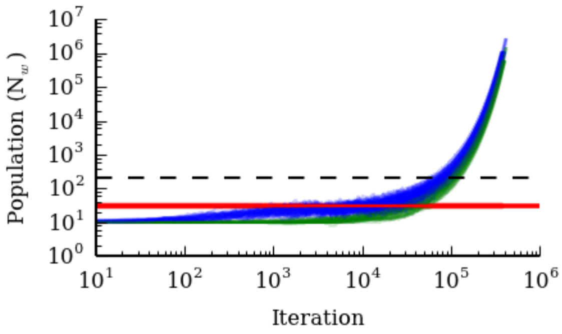


FIG. 14. $U = 0.5$, $N_{\text{dets}} = 4\text{e}{+}03$ (12 sites, 18 electrons), $N_{\text{plat}} = 31.4 \pm 15$ %

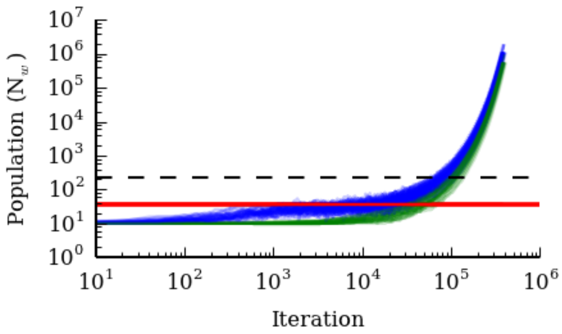


FIG. 15. $U = 0.5$, $N_{\text{dets}} = 9.5\text{e}{+}03$ (14 sites, 6 electrons), $N_{\text{plat}} = 38.2 \pm 0.56$ %

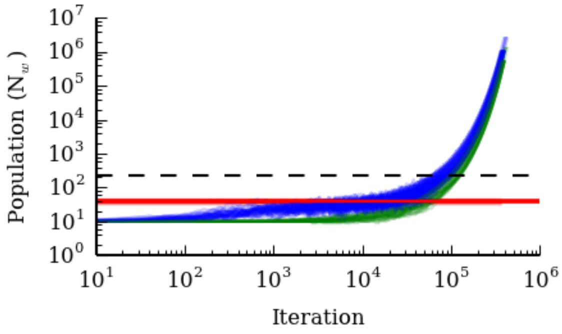


FIG. 16. $U = 0.5$, $N_{\text{dets}} = 9.5\text{e}{+}03$ (14 sites, 22 electrons), $N_{\text{plat}} = 38.5 \pm 16$ %

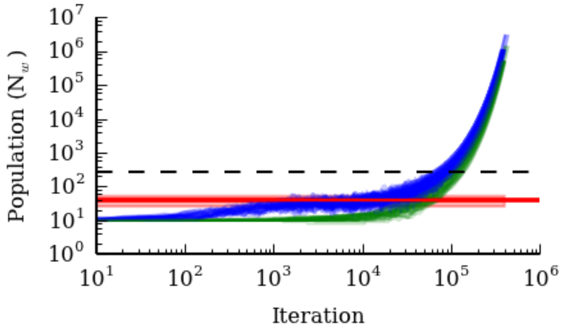


FIG. 17. $U = 0.5$, $N_{\text{dets}} = 2\text{e}{+}04$ (16 sites, 26 electrons), $N_{\text{plat}} = 39.3 \pm 34$ % (manual correction: 40)

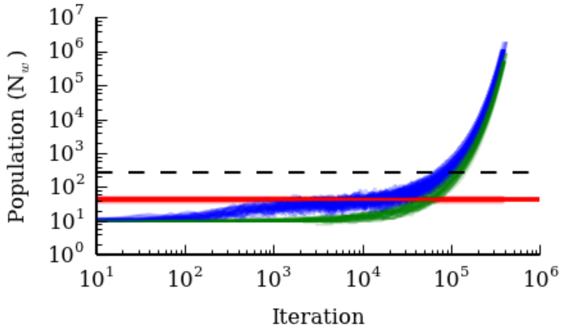


FIG. 18. $U = 0.5$, $N_{\text{dets}} = 2\text{e}{+}04$ (16 sites, 6 electrons), $N_{\text{plat}} = 43.3 \pm 19$ %

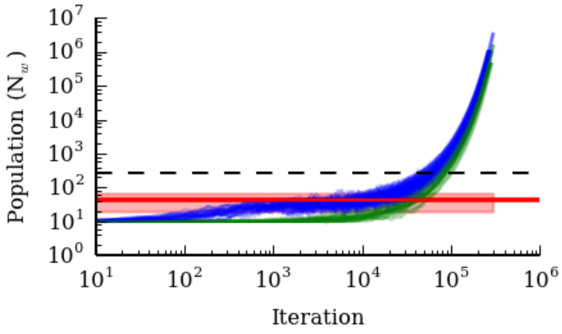


FIG. 19. $U = 0.5$, $N_{\rm dets} = 2e+04$ (12 sites, 8 electrons), $N_{\rm plat} = 42 \pm 55$ % (manual correction: 30)

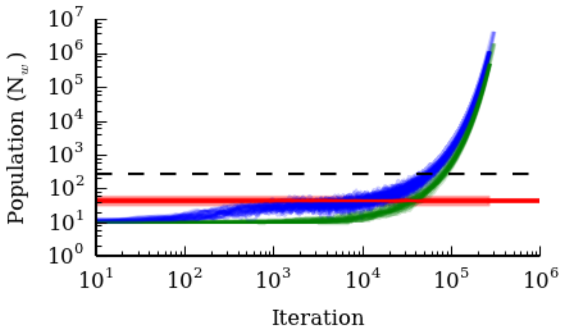


FIG. 20. $U = 0.5$, $N_{\rm dets} = 2e+04$ (12 sites, 16 electrons), $N_{\rm plat} = 44.7 \pm 28$ %

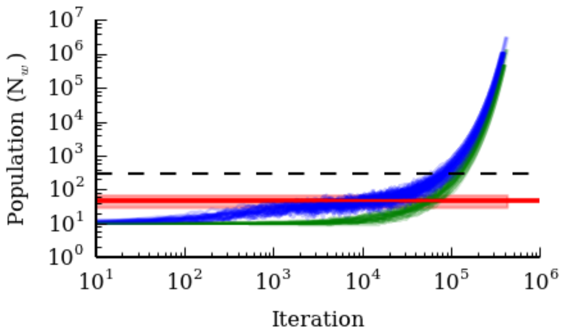


FIG. 21. $U = 0.5$, $N_{\rm dets} = 3.7e+04$ (18 sites, 30 electrons), $N_{\rm plat} = 47.8 \pm 39$ % (manual correction: 40)

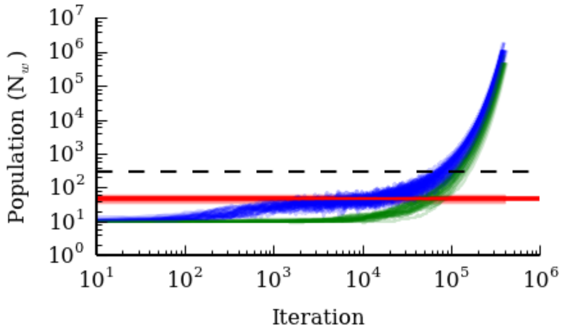


FIG. 22. $U = 0.5$, $N_{\rm dets} = 3.7e+04$ (18 sites, 6 electrons), $N_{\rm plat} = 46.7 \pm 24$ %

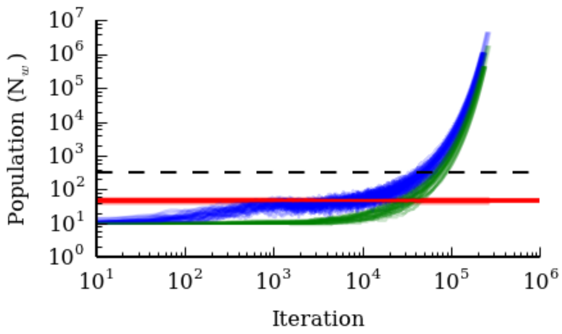


FIG. 23. $U = 0.5$, $N_{\rm dets} = 5.2e+04$ (12 sites, 10 electrons), $N_{\rm plat} = 46.6 \pm 18$ %

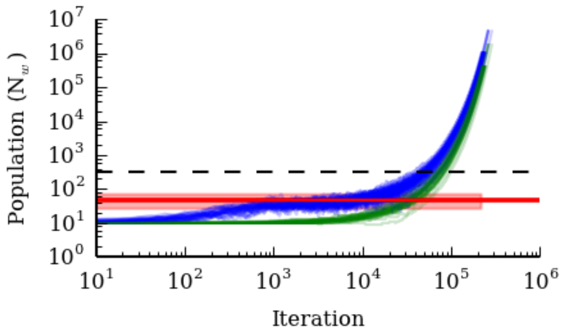


FIG. 24. $U = 0.5$, $N_{\rm dets} = 5.2e+04$ (12 sites, 14 electrons), $N_{\rm plat} = 48.3 \pm 45$ % (manual correction: 35)

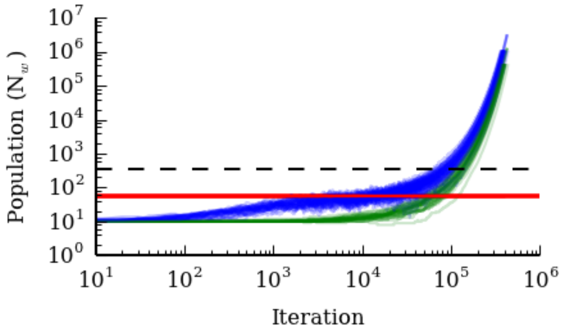


FIG. 25. $U$ = 0.5, $N_{\rm dets}$ = 6.5e+04 (20 sites, 34 electrons), $N_{\rm plat}$ = 54.2 ± 0.35 %

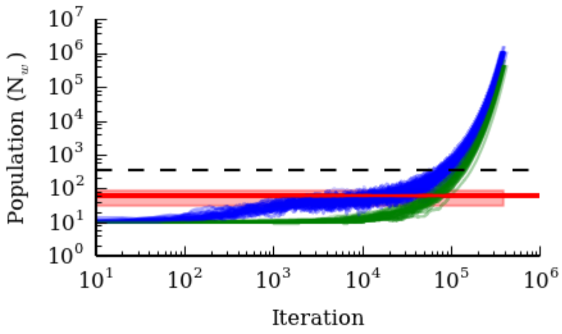


FIG. 26. $U$ = 0.5, $N_{\rm dets}$ = 6.5e+04 (20 sites, 6 electrons), $N_{\rm plat}$ = 59.3 ± 48 % (manual correction: 30)

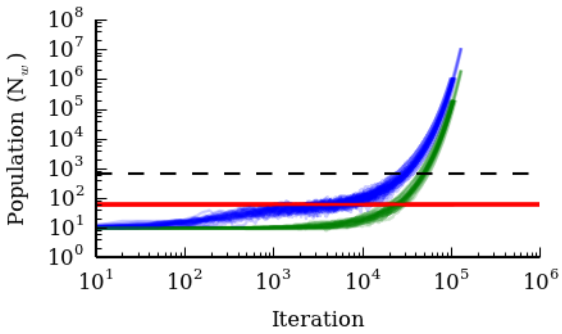


FIG. 27. $U$ = 0.5, $N_{\rm dets}$ = 7.1e+04 (12 sites, 12 electrons), $N_{\rm plat}$ = 58.3 ± 2.3 %

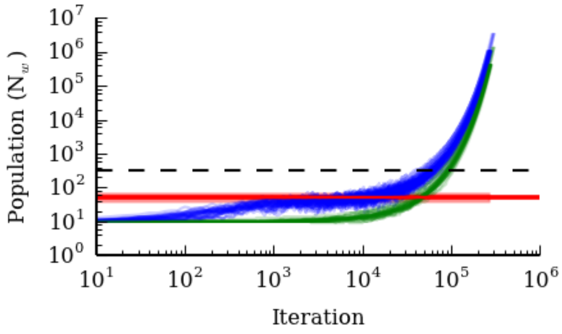


FIG. 28. $U$ = 0.5, $N_{\rm dets}$ = 7.2e+04 (14 sites, 8 electrons), $N_{\rm plat}$ = 52 ± 27 %

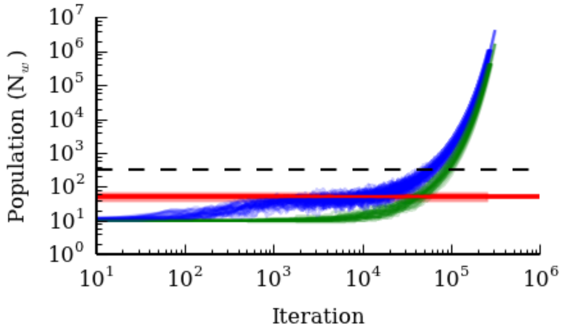


FIG. 29. $U$ = 0.5, $N_{\rm dets}$ = 7.2e+04 (14 sites, 20 electrons), $N_{\rm plat}$ = 51.3 ± 25 %

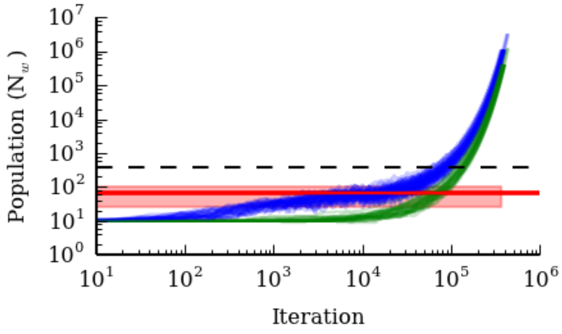


FIG. 30. $U$ = 0.5, $N_{\rm dets}$ = 1.1e+05 (22 sites, 38 electrons), $N_{\rm plat}$ = 64.8 ± 60 % (manual correction: 80)

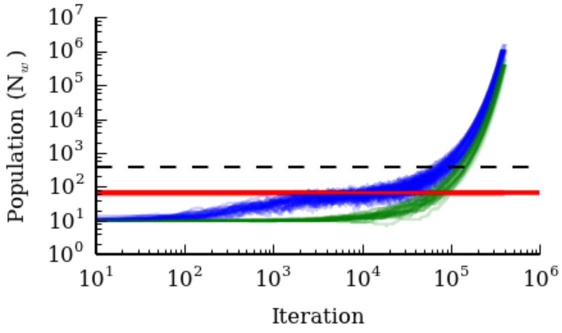


FIG. 31. $U = 0.5$, $N_{\rm dets} = 1.1e{+}05$ (22 sites, 6 electrons), $N_{\rm plat} = 65.8 \pm 15$ %

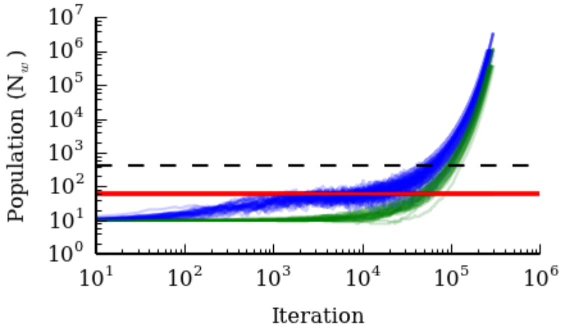


FIG. 32. $U = 0.5$, $N_{\rm dets} = 2.1e{+}05$ (16 sites, 8 electrons), $N_{\rm plat} = 61.3 \pm 5.6$ %

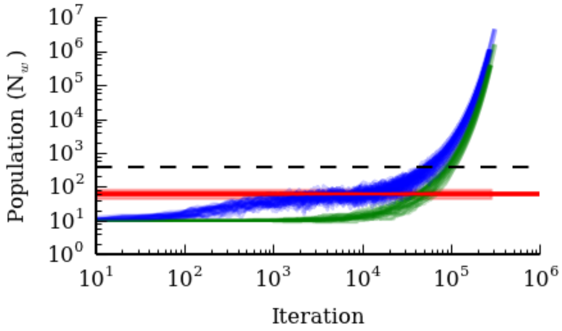


FIG. 33. $U = 0.5$, $N_{\rm dets} = 2.1e{+}05$ (16 sites, 24 electrons), $N_{\rm plat} = 62.7 \pm 29$ %

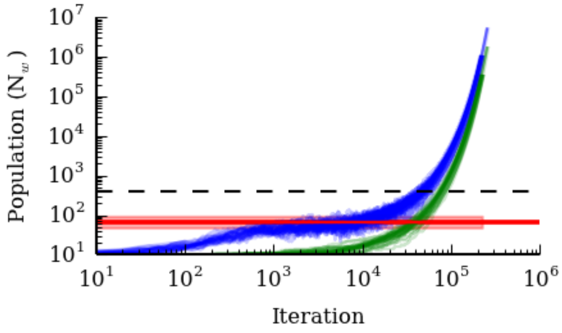


FIG. 34. $U = 0.5$, $N_{\rm dets} = 2.9e{+}05$ (14 sites, 18 electrons), $N_{\rm plat} = 68.3 \pm 32$ % (manual correction: 50)

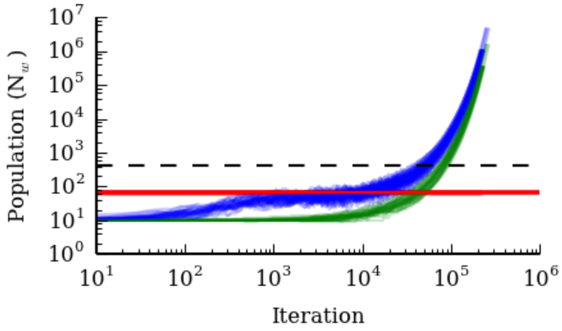


FIG. 35. $U = 0.5$, $N_{\rm dets} = 2.9e{+}05$ (14 sites, 10 electrons), $N_{\rm plat} = 64.9 \pm 13$ %

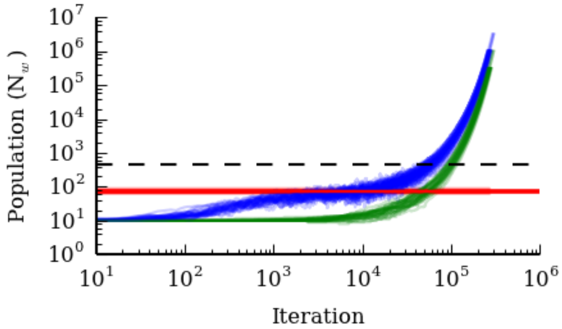


FIG. 36. $U = 0.5$, $N_{\rm dets} = 5.2e{+}05$ (18 sites, 8 electrons), $N_{\rm plat} = 75.9 \pm 18$ %

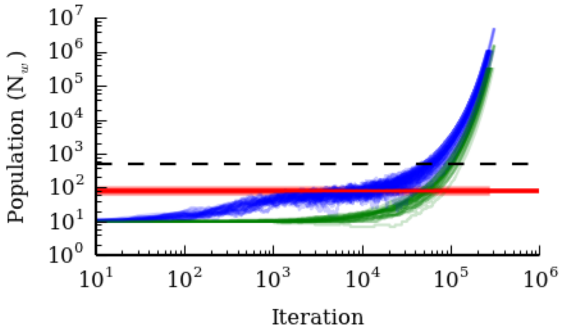


FIG. 37. $U$ = 0.5, $N_{\rm dets}$ = 5.2e+05 (18 sites, 28 electrons), $N_{\rm plat}$ = 81.4 ± 24 %

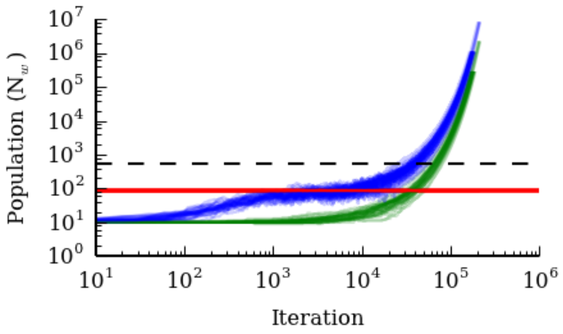


FIG. 38. $U$ = 0.5, $N_{\rm dets}$ = 6.4e+05 (14 sites, 16 electrons), $N_{\rm plat}$ = 84.1 ± 3.4 %

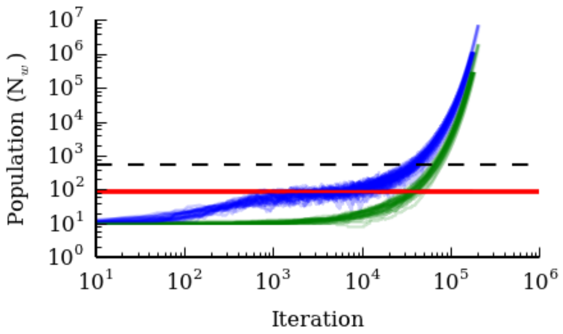


FIG. 39. $U$ = 0.5, $N_{\rm dets}$ = 6.4e+05 (14 sites, 12 electrons), $N_{\rm plat}$ = 90 ± 3.4 %

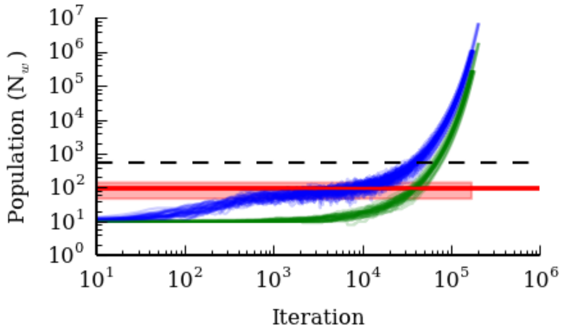


FIG. 40. $U$ = 0.5, $N_{\rm dets}$ = 8.4e+05 (14 sites, 14 electrons), $N_{\rm plat}$ = 93.7 ± 50 % (manual correction: 60)

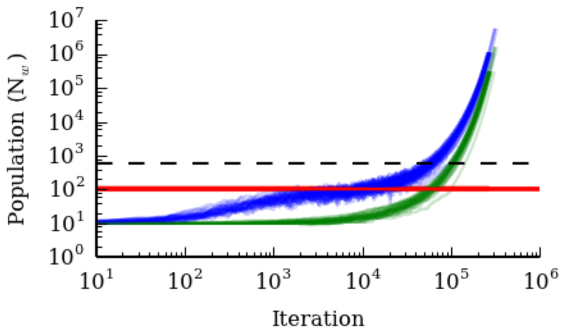


FIG. 41. $U$ = 0.5, $N_{\rm dets}$ = 1.2e+06 (20 sites, 32 electrons), $N_{\rm plat}$ = 108 ± 13 %

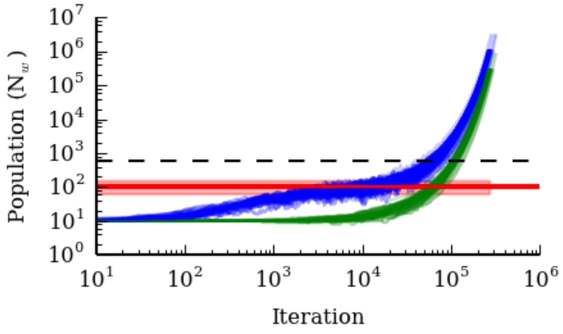


FIG. 42. $U$ = 0.5, $N_{\rm dets}$ = 1.2e+06 (20 sites, 8 electrons), $N_{\rm plat}$ = 106 ± 42 % (manual correction: 80)

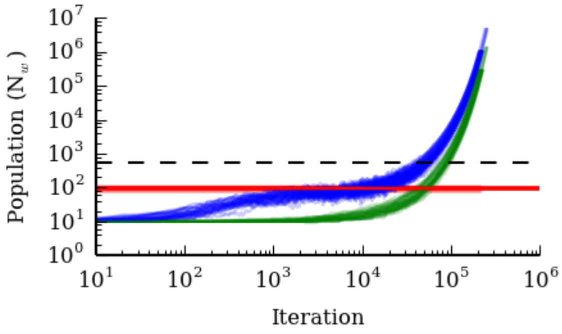


FIG. 43. $U = 0.5$, $N_{\text{dets}} = 1.2\text{e}{+}06$ (16 sites, 10 electrons), $N_{\text{plat}} = 91.8 \pm 19$ %

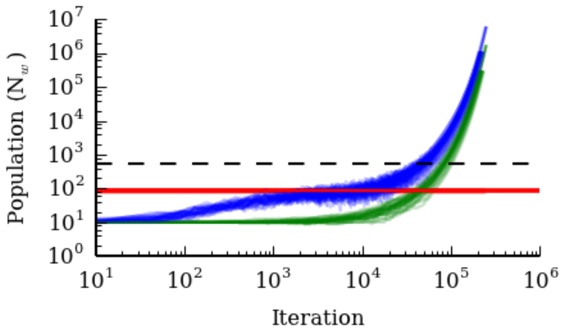


FIG. 44. $U = 0.5$, $N_{\text{dets}} = 1.2\text{e}{+}06$ (16 sites, 22 electrons), $N_{\text{plat}} = 84.4 \pm 12$ %

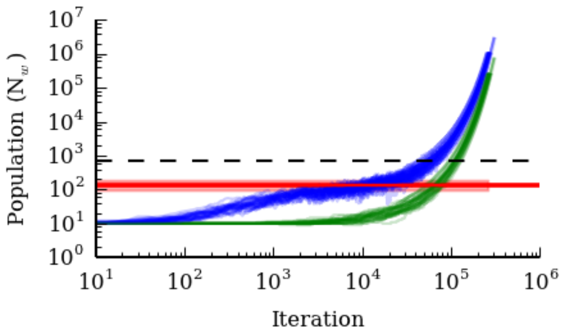


FIG. 45. $U = 0.5$, $N_{\text{dets}} = 2.4\text{e}{+}06$ (22 sites, 8 electrons), $N_{\text{plat}} = 136 \pm 32$ % (manual correction: 80)

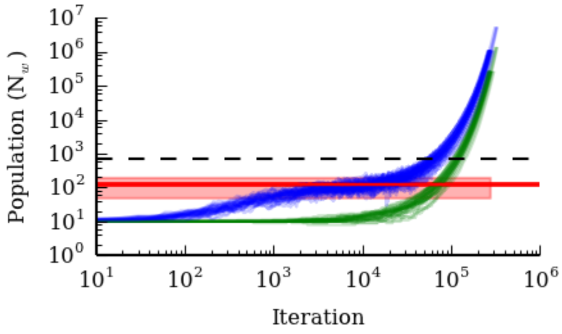


FIG. 46. $U = 0.5$, $N_{\text{dets}} = 2.4\text{e}{+}06$ (22 sites, 36 electrons), $N_{\text{plat}} = 120 \pm 60$ % (manual correction: 100)

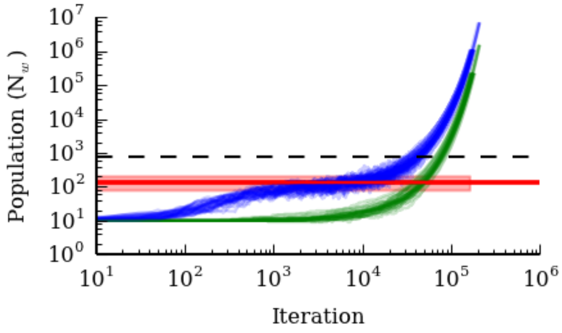


FIG. 47. $U = 0.5$, $N_{\text{dets}} = 4\text{e}{+}06$ (16 sites, 12 electrons), $N_{\text{plat}} = 139 \pm 45$ % (manual correction: 100)

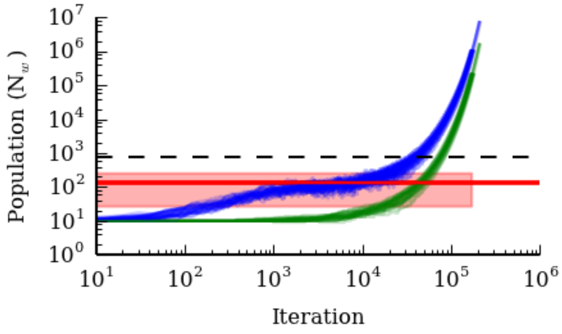


FIG. 48. $U = 0.5$, $N_{\text{dets}} = 4\text{e}{+}06$ (16 sites, 20 electrons), $N_{\text{plat}} = 140 \pm 81$ % (manual correction: 100)

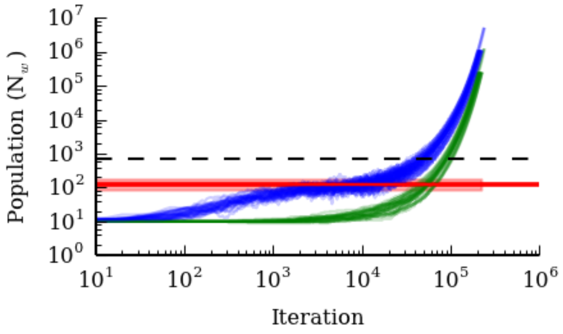


FIG. 49. $U = 0.5$, $N_{\rm dets} = 4.1e{+}06$ (18 sites, 10 electrons), $N_{\rm plat} = 127 \pm 35$ % (manual correction: 100)

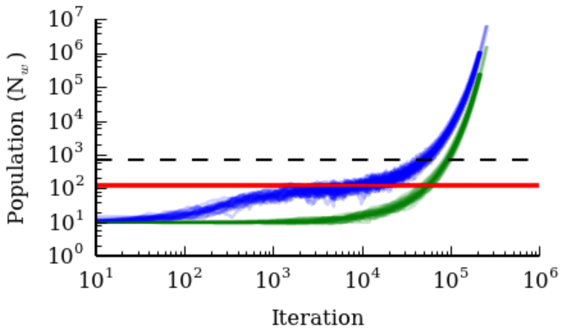


FIG. 50. $U = 0.5$, $N_{\rm dets} = 4.1e{+}06$ (18 sites, 26 electrons), $N_{\rm plat} = 125 \pm 2.2$ %

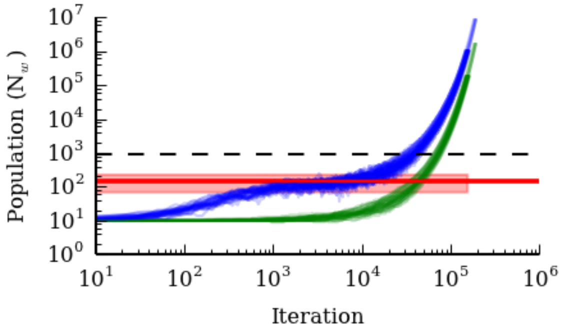


FIG. 51. $U = 0.5$, $N_{\rm dets} = 8.2e{+}06$ (16 sites, 18 electrons), $N_{\rm plat} = 149 \pm 54$ % (manual correction: 200)

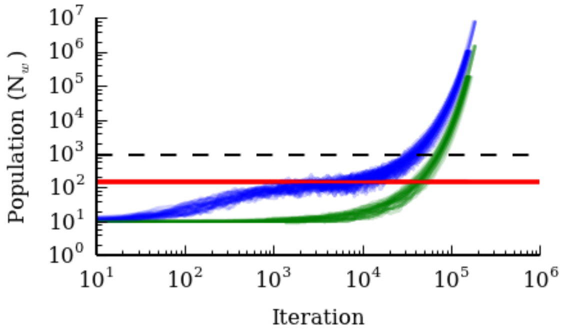


FIG. 52. $U = 0.5$, $N_{\rm dets} = 8.2e{+}06$ (16 sites, 14 electrons), $N_{\rm plat} = 154 \pm 5.2$ %

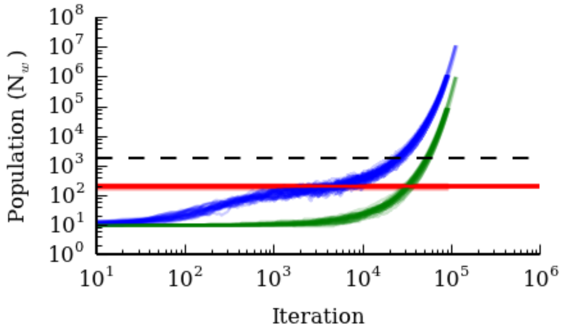


FIG. 53. $U = 0.5$, $N_{\rm dets} = 1e{+}07$ (16 sites, 16 electrons), $N_{\rm plat} = 194 \pm 20$ %

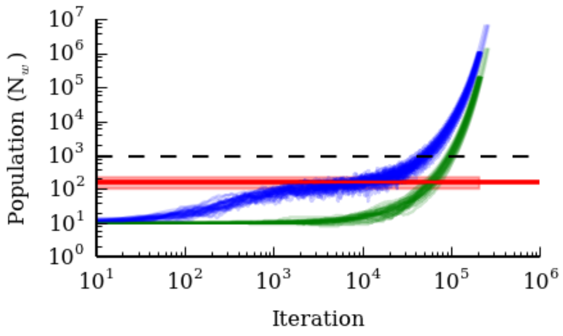


FIG. 54. $U = 0.5$, $N_{\rm dets} = 1.2e{+}07$ (20 sites, 30 electrons), $N_{\rm plat} = 163 \pm 37$ % (manual correction: 150)

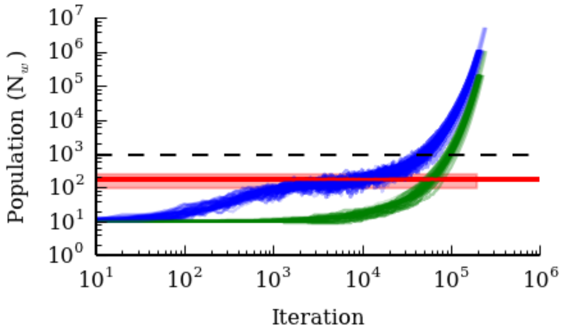


FIG. 55. $U = 0.5$, $N_{\rm dets} = 1.2\text{e}{+}07$ (20 sites, 10 electrons), $N_{\rm plat} = 171 \pm 43$ % (manual correction: 150)

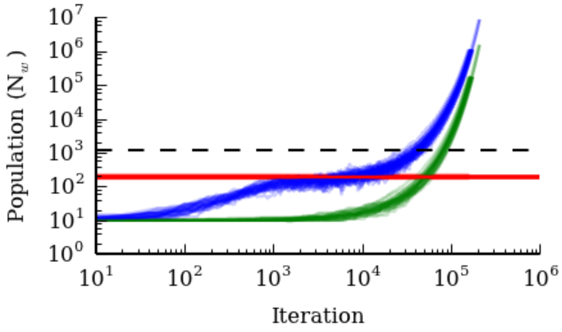


FIG. 56. $U = 0.5$, $N_{\rm dets} = 1.9\text{e}{+}07$ (18 sites, 24 electrons), $N_{\rm plat} = 199 \pm 15$ %

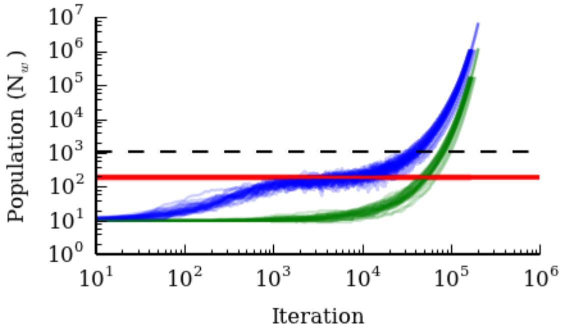


FIG. 57. $U = 0.5$, $N_{\rm dets} = 1.9\text{e}{+}07$ (18 sites, 12 electrons), $N_{\rm plat} = 189 \pm 14$ %

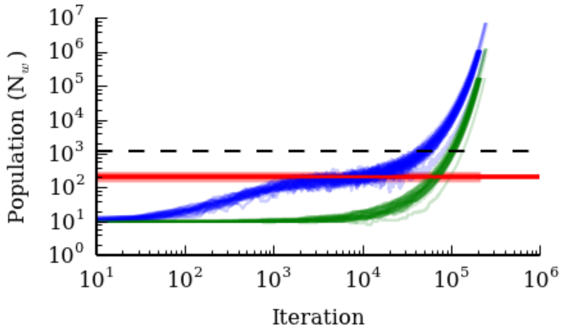


FIG. 58. $U = 0.5$, $N_{\rm dets} = 3.2\text{e}{+}07$ (22 sites, 34 electrons), $N_{\rm plat} = 212 \pm 27$ %

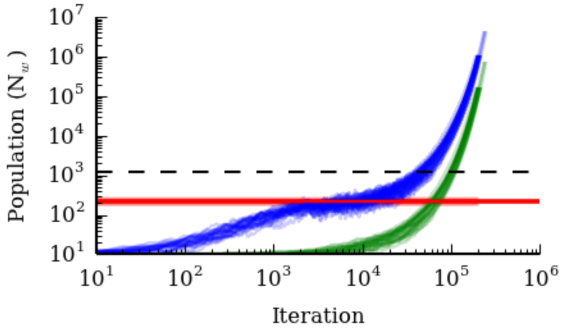


FIG. 59. $U = 0.5$, $N_{\rm dets} = 3.2\text{e}{+}07$ (22 sites, 10 electrons), $N_{\rm plat} = 219 \pm 19$ %

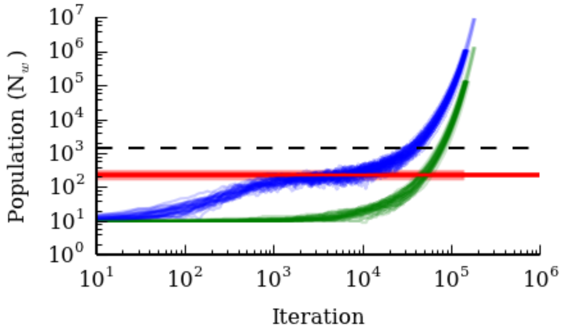


FIG. 60. $U = 0.5$, $N_{\rm dets} = 5.6\text{e}{+}07$ (18 sites, 22 electrons), $N_{\rm plat} = 233 \pm 27$ %

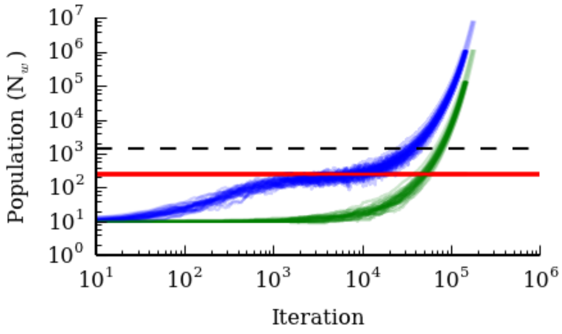


FIG. 61. $U = 0.5$, $N_{\rm dets} = 5.6\text{e}{+}07$ (18 sites, 14 electrons), $N_{\rm plat} = 253 \pm 3.7$ %

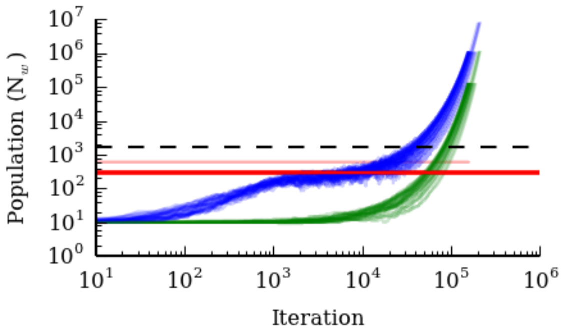


FIG. 62. $U = 0.5$, $N_{\rm dets} = 7.5\text{e}{+}07$ (20 sites, 28 electrons), $N_{\rm plat} = 299 \pm 1\text{e}{+}02$ % (manual correction: 400)

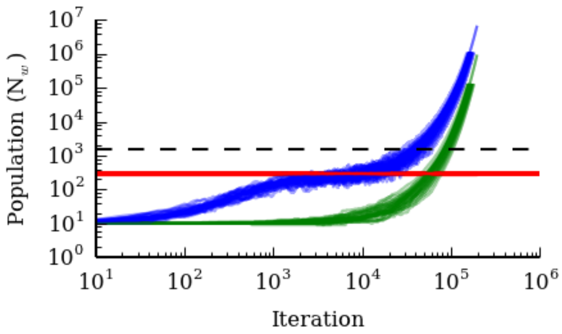


FIG. 63. $U = 0.5$, $N_{\rm dets} = 7.5\text{e}{+}07$ (20 sites, 12 electrons), $N_{\rm plat} = 288 \pm 9.4$ %

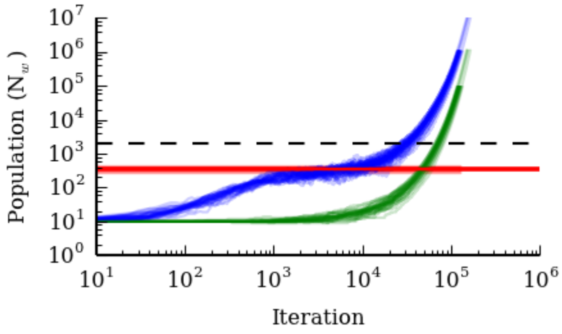


FIG. 64. $U = 0.5$, $N_{\rm dets} = 1.1\text{e}{+}08$ (18 sites, 20 electrons), $N_{\rm plat} = 345 \pm 22$ %

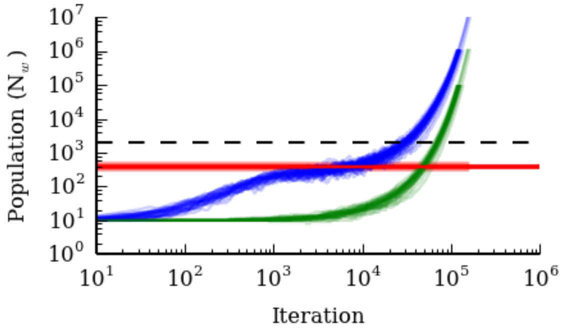


FIG. 65. $U = 0.5$, $N_{\rm dets} = 1.1\text{e}{+}08$ (18 sites, 16 electrons), $N_{\rm plat} = 401 \pm 26$ %

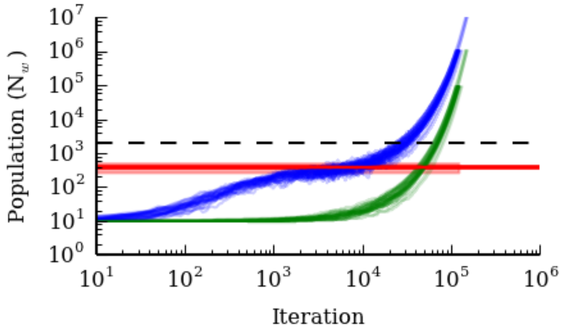


FIG. 66. $U = 0.5$, $N_{\rm dets} = 1.3\text{e}{+}08$ (18 sites, 18 electrons), $N_{\rm plat} = 376 \pm 31$ % (manual correction: 300)

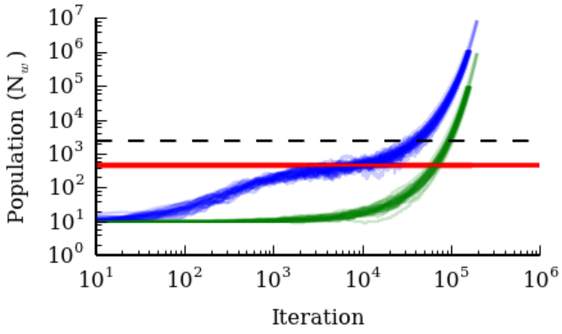


FIG. 67. $U = 0.5$, $N_{\rm dets} = 2.5e{+}08$ (22 sites, 32 electrons), $N_{\rm plat} = 451 \pm 14$ %

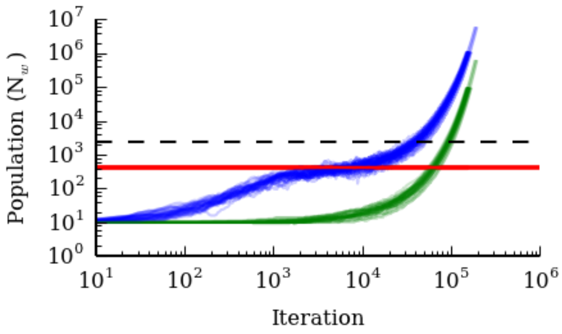


FIG. 68. $U = 0.5$, $N_{\rm dets} = 2.5e{+}08$ (22 sites, 12 electrons), $N_{\rm plat} = 412 \pm 8.4$ %

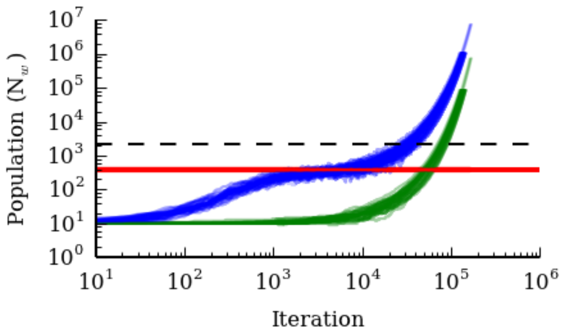


FIG. 69. $U = 0.5$, $N_{\rm dets} = 3e{+}08$ (20 sites, 14 electrons), $N_{\rm plat} = 391 \pm 13$ %

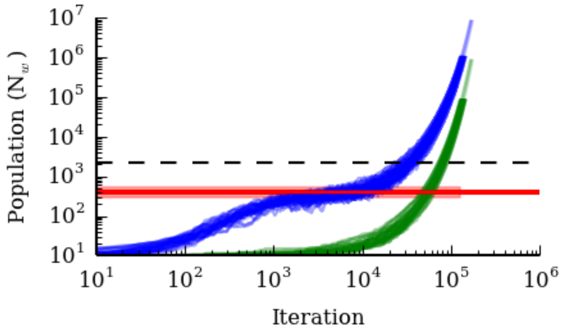


FIG. 70. $U = 0.5$, $N_{\rm dets} = 3e{+}08$ (20 sites, 26 electrons), $N_{\rm plat} = 409 \pm 28$ %

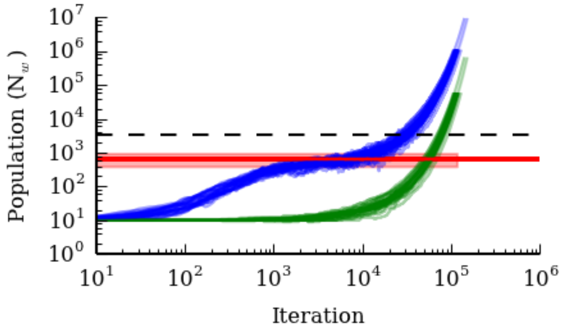


FIG. 71. $U = 0.5$, $N_{\rm dets} = 7.9e{+}08$ (20 sites, 16 electrons), $N_{\rm plat} = 645 \pm 42$ % (manual correction: 500)

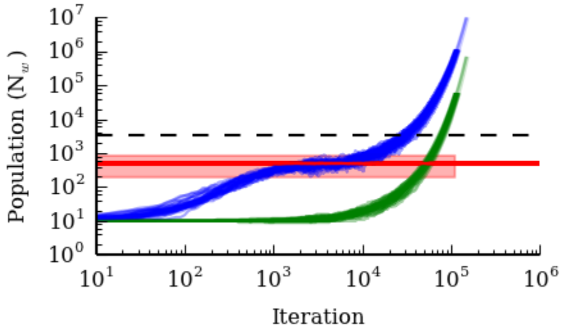


FIG. 72. $U = 0.5$, $N_{\rm dets} = 7.9e{+}08$ (20 sites, 24 electrons), $N_{\rm plat} = 518 \pm 62$ % (manual correction: 600)

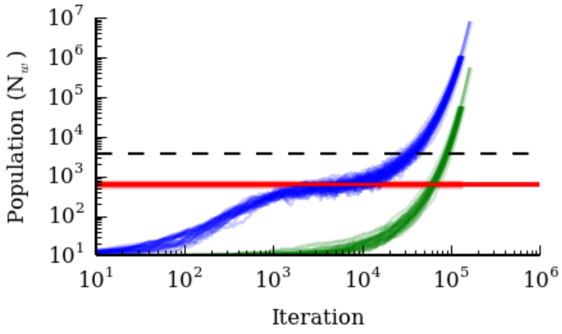


FIG. 73. $U = 0.5$, $N_{\text{dets}} = 1.3\text{e}{+}09$ (22 sites, 30 electrons), $N_{\text{plat}} = 619 \pm 17$ %

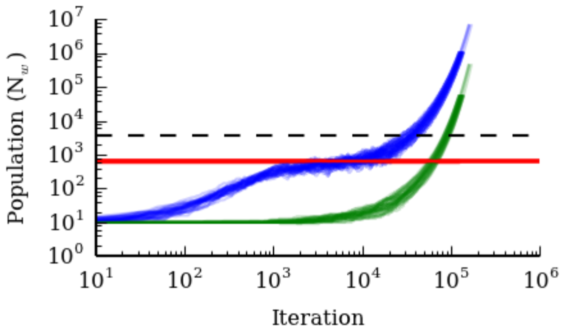


FIG. 74. $U = 0.5$, $N_{\text{dets}} = 1.3\text{e}{+}09$ (22 sites, 14 electrons), $N_{\text{plat}} = 620 \pm 9.8$ %

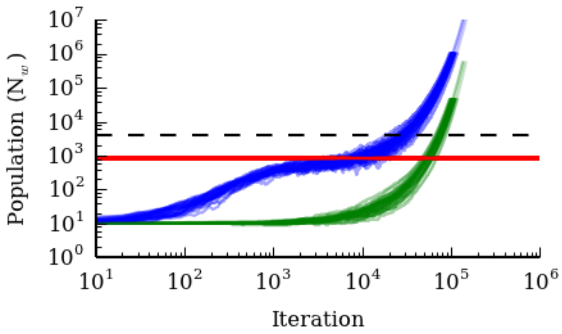


FIG. 75. $U = 0.5$, $N_{\text{dets}} = 1.4\text{e}{+}09$ (20 sites, 22 electrons), $N_{\text{plat}} = 831 \pm 0.16$ %

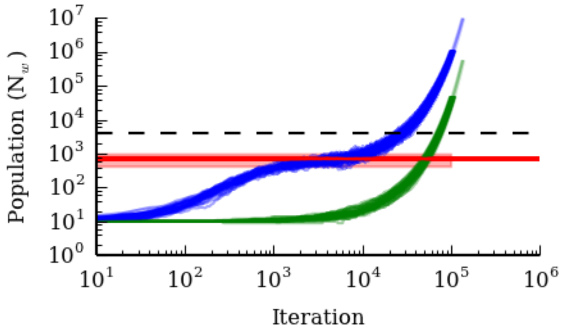


FIG. 76. $U = 0.5$, $N_{\text{dets}} = 1.4\text{e}{+}09$ (20 sites, 18 electrons), $N_{\text{plat}} = 675 \pm 39$ % (manual correction: 800)

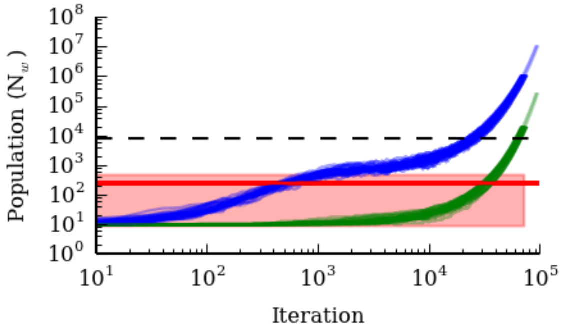


FIG. 77. $U = 0.5$, $N_{\text{dets}} = 1.7\text{e}{+}09$ (20 sites, 20 electrons), $N_{\text{plat}} = 238 \pm 96$ % (manual correction: 1e+03)

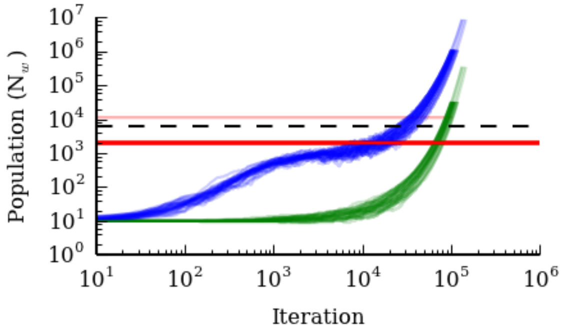


FIG. 78. $U = 0.5$, $N_{\text{dets}} = 4.7\text{e}{+}09$ (22 sites, 28 electrons), $N_{\text{plat}} = 1.99\text{e}{+}03 \pm 4.7\text{e}{+}02$ % (manual correction: 1e+03)

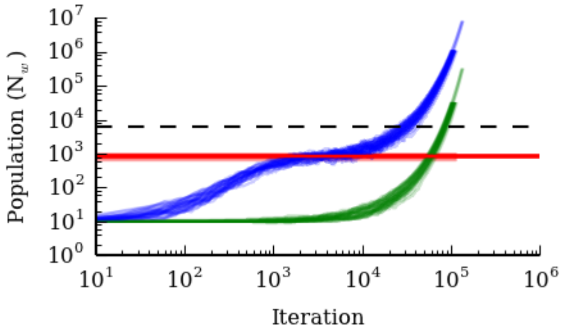


FIG. 79. $U = 0.5$, $N_{\text{dets}} = 4.7\text{e}{+}09$ (22 sites, 16 electrons), $N_{\text{plat}} = 814 \pm 22$ %

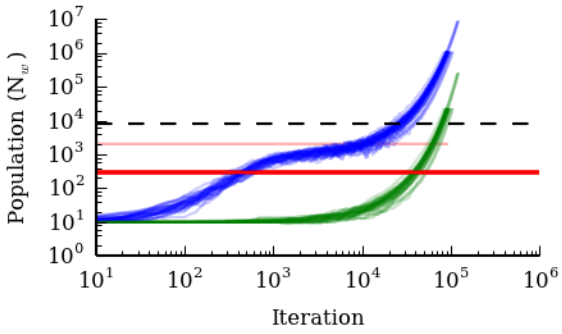


FIG. 80. $U = 0.5$, $N_{\text{dets}} = 1.1\text{e}{+}10$ (22 sites, 26 electrons), $N_{\text{plat}} = 299 \pm 5.8\text{e}{+}02$ % (manual correction: 1.5e+03)

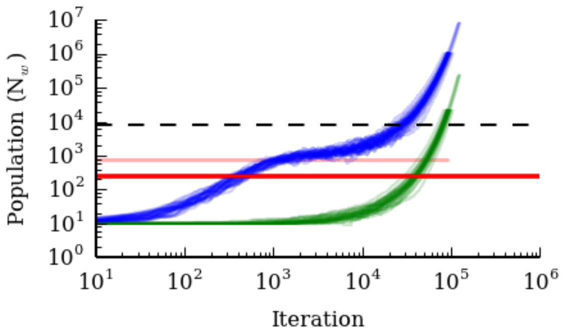


FIG. 81. $U = 0.5$, $N_{\text{dets}} = 1.1\text{e}{+}10$ (22 sites, 18 electrons), $N_{\text{plat}} = 248 \pm 2\text{e}{+}02$ % (manual correction: 1.5e+03)

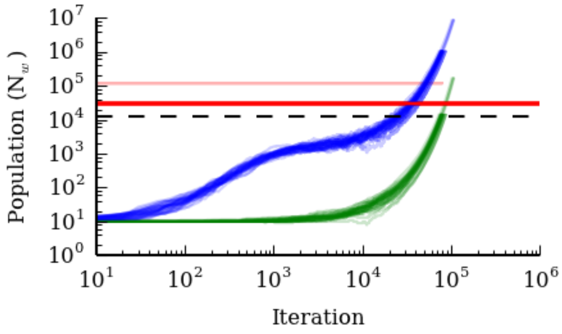


FIG. 82. $U = 0.5$, $N_{\text{dets}} = 1.9\text{e}{+}10$ (22 sites, 20 electrons), $N_{\text{plat}} = 2.89\text{e}{+}04 \pm 3.1\text{e}{+}02$ % (manual correction: 2e+03)

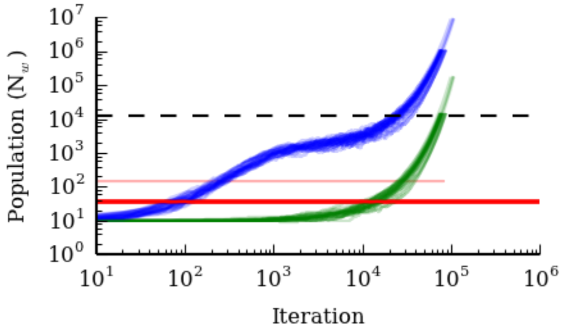


FIG. 83. $U = 0.5$, $N_{\text{dets}} = 1.9\text{e}{+}10$ (22 sites, 24 electrons), $N_{\text{plat}} = 35.1 \pm 3.2\text{e}{+}02$ % (manual correction: 3e+03)

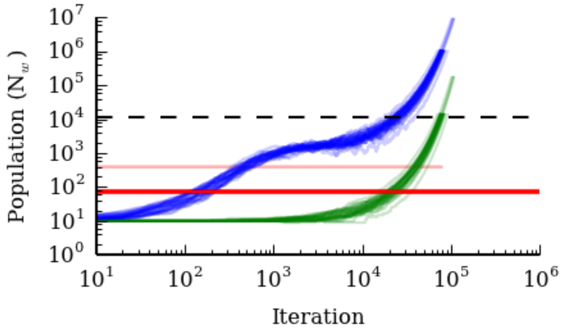


FIG. 84. $U = 0.5$, $N_{\text{dets}} = 2.3\text{e}{+}10$ (22 sites, 22 electrons), $N_{\text{plat}} = 72.5 \pm 4.4\text{e}{+}02$ % (manual correction: 2e+03)

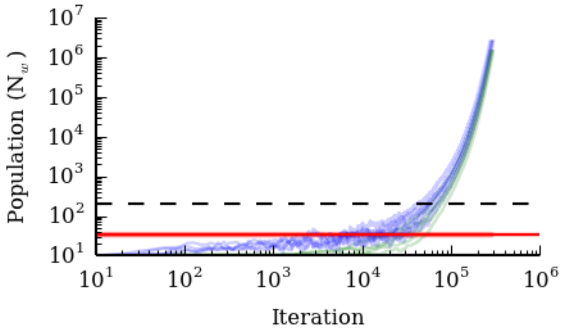


FIG. 85. $U$ = 0.75, $N_{\mathrm{dets}}$ = 3.7e+02 (12 sites, 4 electrons), $N_{\mathrm{plat}}$ = 33.7 ± 9.3 %

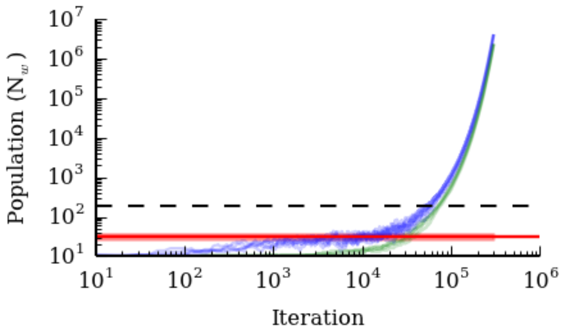


FIG. 86. $U$ = 0.75, $N_{\mathrm{dets}}$ = 3.7e+02 (12 sites, 20 electrons), $N_{\mathrm{plat}}$ = 31 ± 17 %

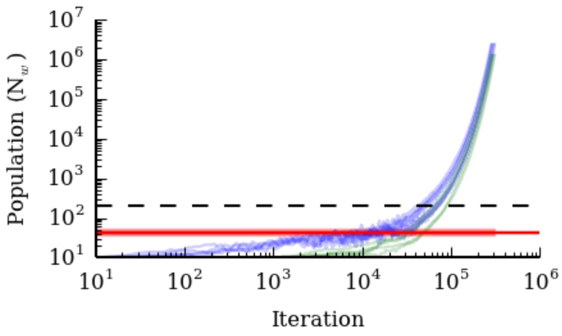


FIG. 87. $U$ = 0.75, $N_{\mathrm{dets}}$ = 6e+02 (14 sites, 4 electrons), $N_{\mathrm{plat}}$ = 43.2 ± 16 %

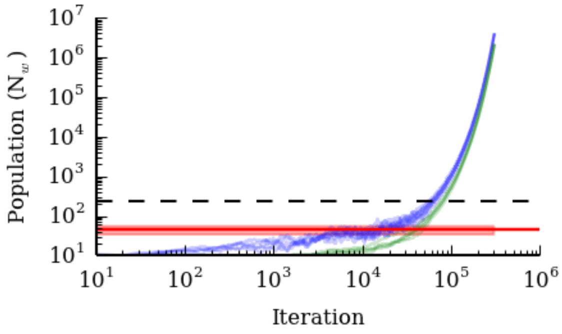


FIG. 88. $U$ = 0.75, $N_{\mathrm{dets}}$ = 6e+02 (14 sites, 24 electrons), $N_{\mathrm{plat}}$ = 44.4 ± 24 %

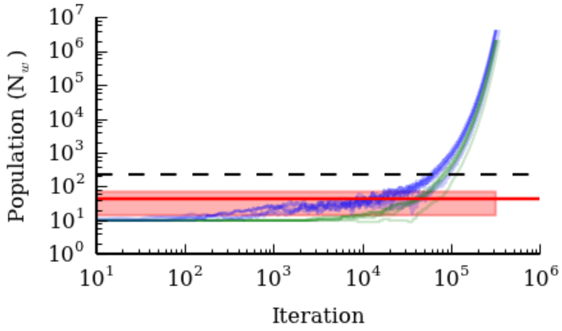


FIG. 89. $U$ = 0.75, $N_{\mathrm{dets}}$ = 9e+02 (16 sites, 28 electrons), $N_{\mathrm{plat}}$ = 42.5 ± 67 % (manual correction: 30)

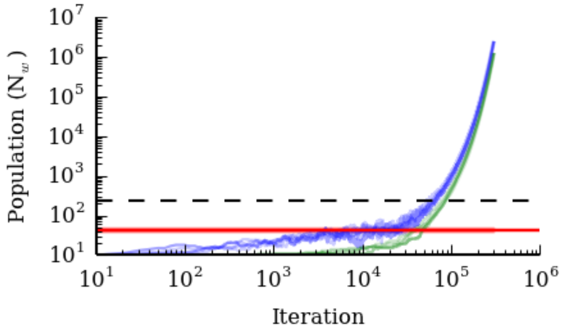


FIG. 90. $U$ = 0.75, $N_{\mathrm{dets}}$ = 9e+02 (16 sites, 4 electrons), $N_{\mathrm{plat}}$ = 42.5 ± 11 %

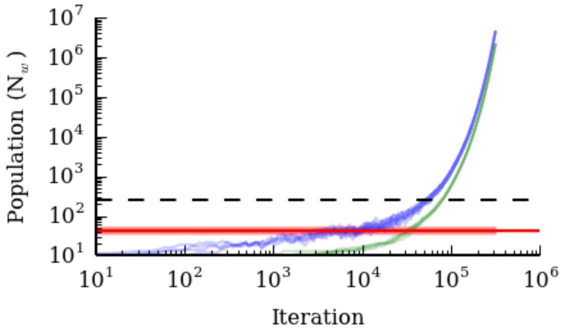


FIG. 91. $U$ = 0.75, $N_{\rm dets}$ = 1.3e+03 (18 sites, 32 electrons), $N_{\rm plat}$ = 43.1 ± 17 %

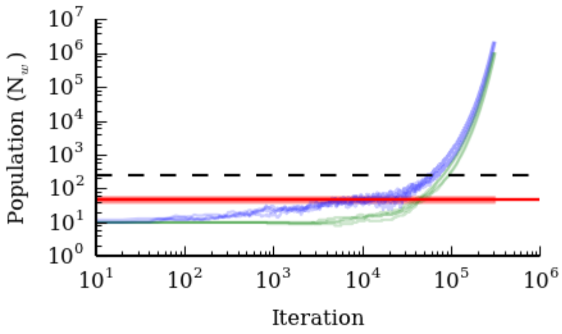


FIG. 92. $U$ = 0.75, $N_{\rm dets}$ = 1.3e+03 (18 sites, 4 electrons), $N_{\rm plat}$ = 47 ± 19 %

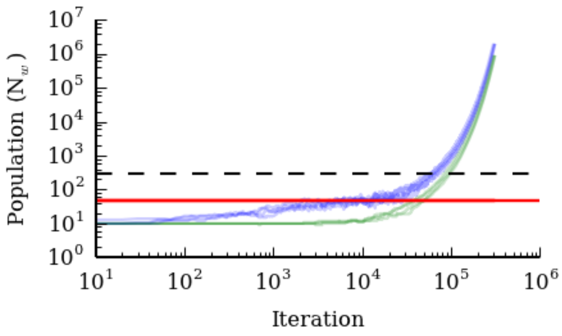


FIG. 93. $U$ = 0.75, $N_{\rm dets}$ = 1.8e+03 (20 sites, 4 electrons), $N_{\rm plat}$ = 48.1 ± 6.7 %

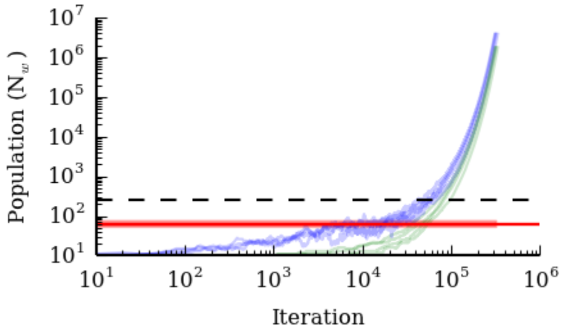


FIG. 94. $U$ = 0.75, $N_{\rm dets}$ = 1.8e+03 (20 sites, 36 electrons), $N_{\rm plat}$ = 63.3 ± 16 %

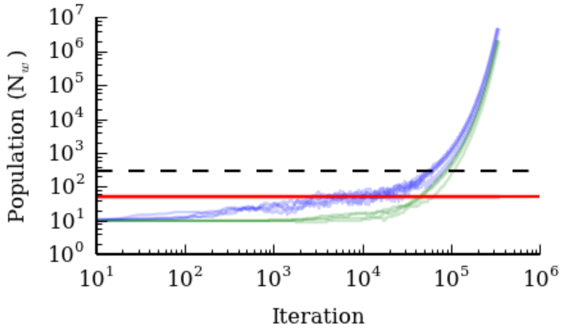


FIG. 95. $U$ = 0.75, $N_{\rm dets}$ = 2.4e+03 (22 sites, 40 electrons), $N_{\rm plat}$ = 50.3 ± 5.4 %

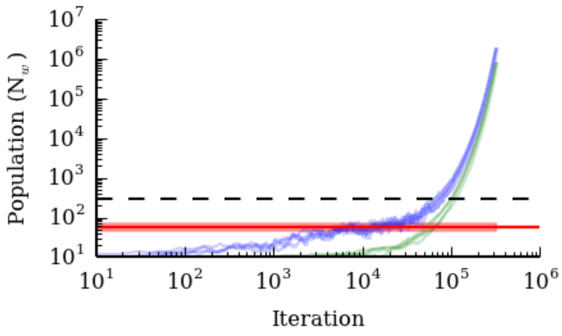


FIG. 96. $U$ = 0.75, $N_{\rm dets}$ = 2.4e+03 (22 sites, 4 electrons), $N_{\rm plat}$ = 57.8 ± 20 %

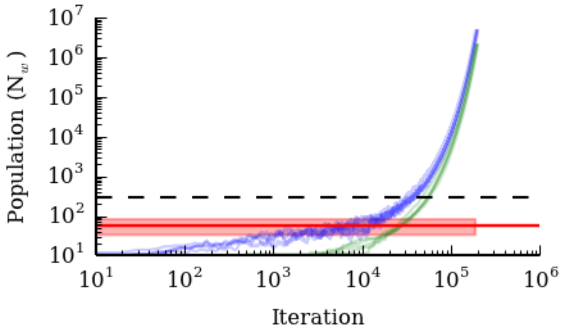


FIG. 97. $U = 0.75$, $N_{\mathrm{dets}} = 4\mathrm{e}{+}03$ (12 sites, 6 electrons), $N_{\mathrm{plat}} = 57.9 \pm 43$ % (manual correction: 50)

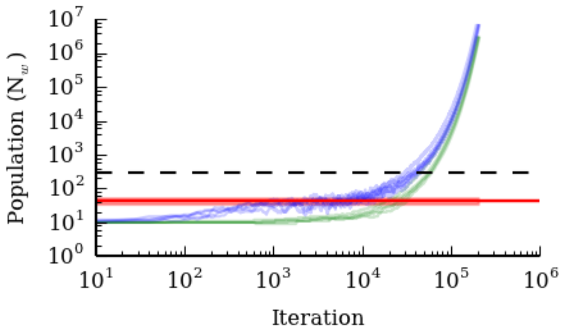


FIG. 98. $U = 0.75$, $N_{\mathrm{dets}} = 4\mathrm{e}{+}03$ (12 sites, 18 electrons), $N_{\mathrm{plat}} = 42.2 \pm 21$ %

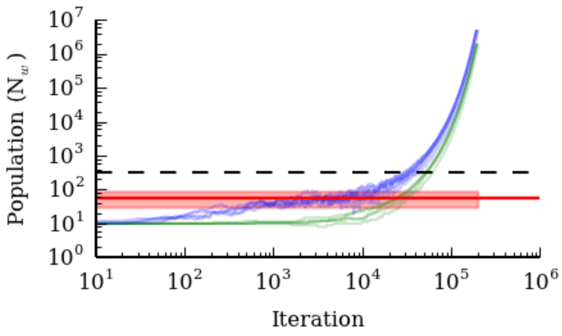


FIG. 99. $U = 0.75$, $N_{\mathrm{dets}} = 9.5\mathrm{e}{+}03$ (14 sites, 6 electrons), $N_{\mathrm{plat}} = 57.3 \pm 49$ % (manual correction: 40)

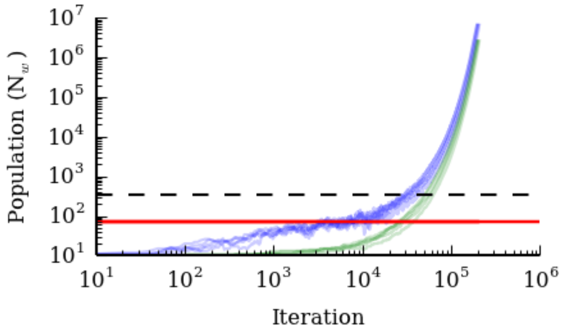


FIG. 100. $U = 0.75$, $N_{\mathrm{dets}} = 9.5\mathrm{e}{+}03$ (14 sites, 22 electrons), $N_{\mathrm{plat}} = 71.4 \pm 7$ %

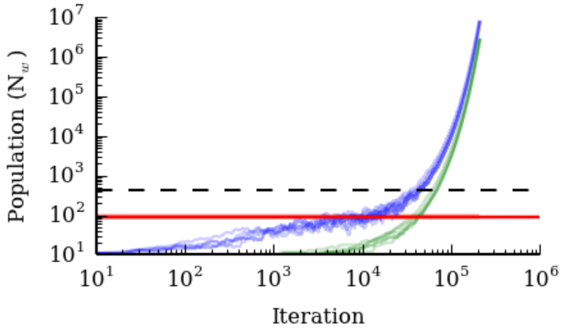


FIG. 101. $U = 0.75$, $N_{\mathrm{dets}} = 2\mathrm{e}{+}04$ (16 sites, 26 electrons), $N_{\mathrm{plat}} = 92.2 \pm 7.8$ %

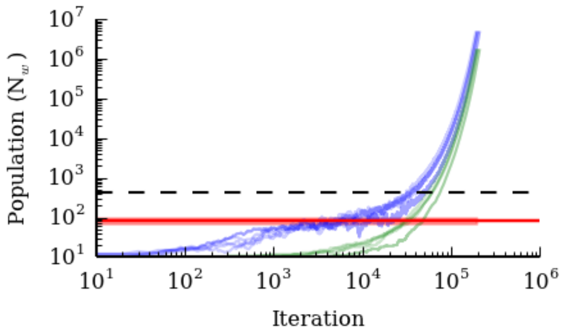


FIG. 102. $U = 0.75$, $N_{\mathrm{dets}} = 2\mathrm{e}{+}04$ (16 sites, 6 electrons), $N_{\mathrm{plat}} = 80.8 \pm 17$ %

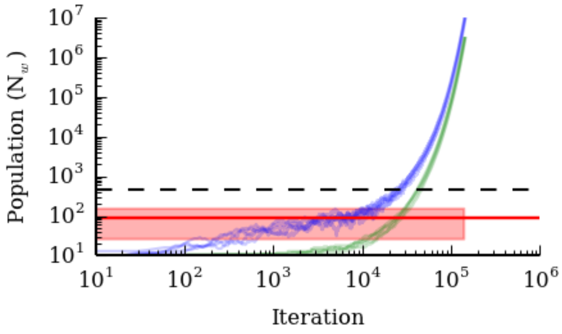


FIG. 103. $U$ = 0.75, $N_{\mathrm{dets}}$ = 2e+04 (12 sites, 8 electrons), $N_{\mathrm{plat}}$ = 89.1 ± 71 % (manual correction: 60)

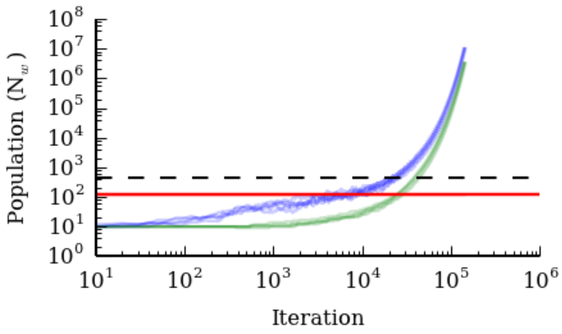


FIG. 104. $U$ = 0.75, $N_{\mathrm{dets}}$ = 2e+04 (12 sites, 16 electrons), $N_{\mathrm{plat}}$ = 121 ± 0.33 %

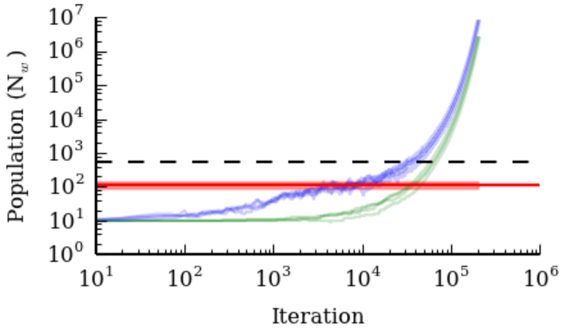


FIG. 105. $U$ = 0.75, $N_{\mathrm{dets}}$ = 3.7e+04 (18 sites, 30 electrons), $N_{\mathrm{plat}}$ = 111 ± 22 %

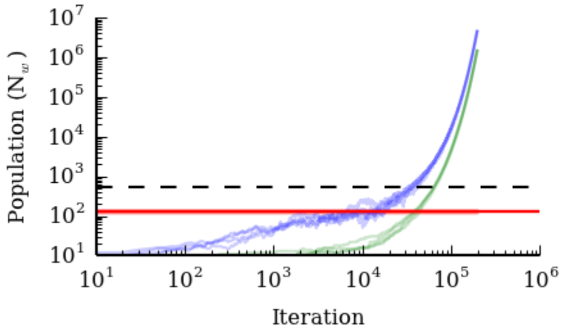


FIG. 106. $U$ = 0.75, $N_{\mathrm{dets}}$ = 3.7e+04 (18 sites, 6 electrons), $N_{\mathrm{plat}}$ = 128 ± 9 %

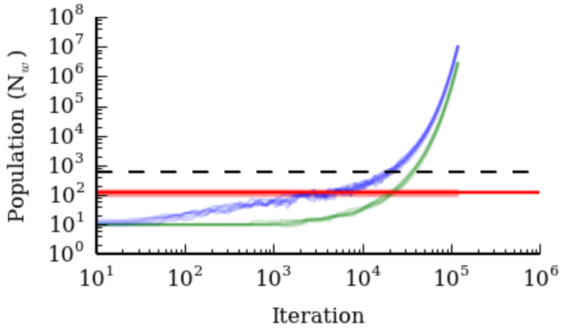


FIG. 107. $U$ = 0.75, $N_{\mathrm{dets}}$ = 5.2e+04 (12 sites, 10 electrons), $N_{\mathrm{plat}}$ = 118 ± 21 %

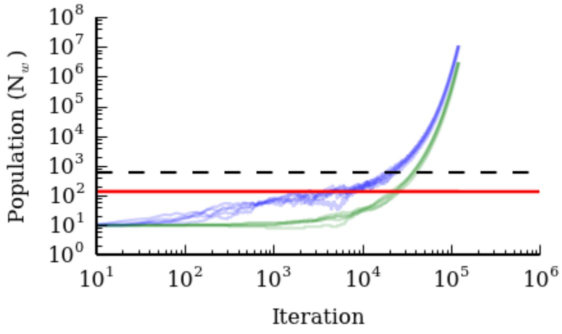


FIG. 108. $U$ = 0.75, $N_{\mathrm{dets}}$ = 5.2e+04 (12 sites, 14 electrons), $N_{\mathrm{plat}}$ = 140 ± 2.3 %

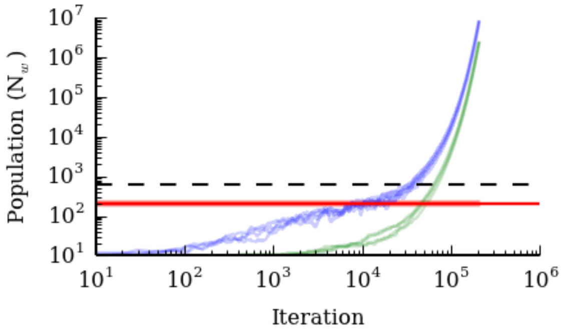


FIG. 109. $U = 0.75$, $N_{\mathrm{dets}} = 6.5\mathrm{e}{+}04$ (20 sites, 34 electrons), $N_{\mathrm{plat}} = 208 \pm 12$ %

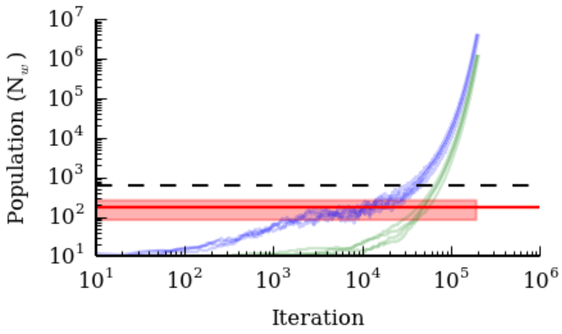


FIG. 110. $U = 0.75$, $N_{\mathrm{dets}} = 6.5\mathrm{e}{+}04$ (20 sites, 6 electrons), $N_{\mathrm{plat}} = 172 \pm 52$ % (manual correction: 150)

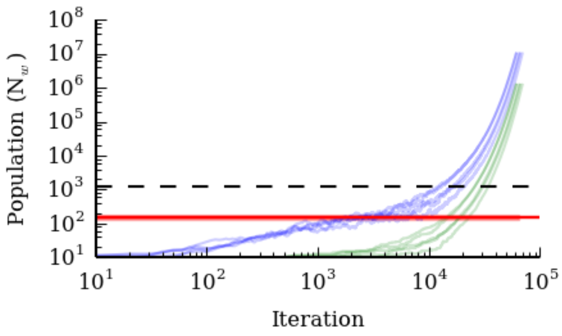


FIG. 111. $U = 0.75$, $N_{\mathrm{dets}} = 7.1\mathrm{e}{+}04$ (12 sites, 12 electrons), $N_{\mathrm{plat}} = 148 \pm 14$ %

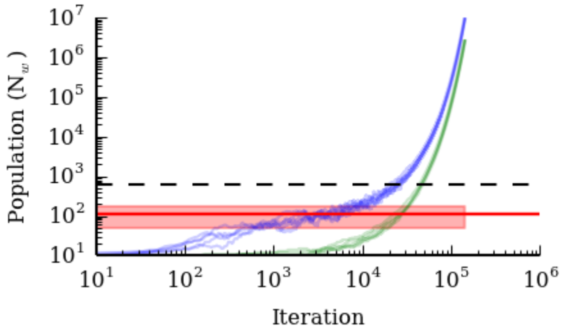


FIG. 112. $U = 0.75$, $N_{\mathrm{dets}} = 7.2\mathrm{e}{+}04$ (14 sites, 8 electrons), $N_{\mathrm{plat}} = 112 \pm 56$ % (manual correction: 100)

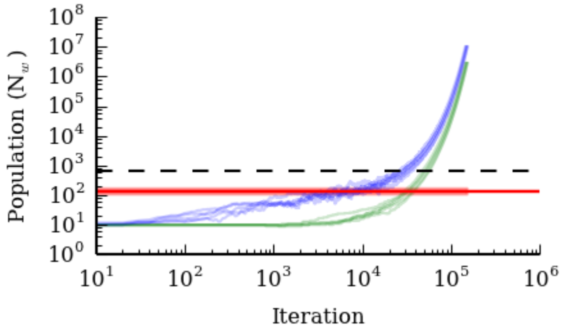


FIG. 113. $U = 0.75$, $N_{\mathrm{dets}} = 7.2\mathrm{e}{+}04$ (14 sites, 20 electrons), $N_{\mathrm{plat}} = 138 \pm 23$ %

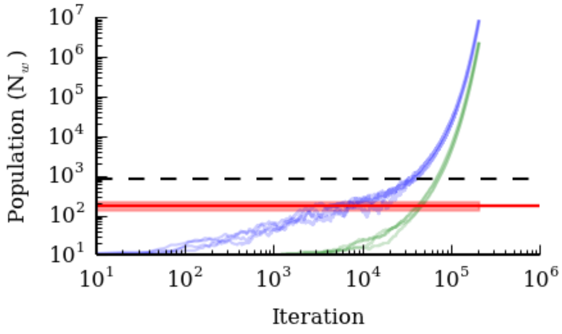


FIG. 114. $U = 0.75$, $N_{\mathrm{dets}} = 1.1\mathrm{e}{+}05$ (22 sites, 38 electrons), $N_{\mathrm{plat}} = 174 \pm 24$ %

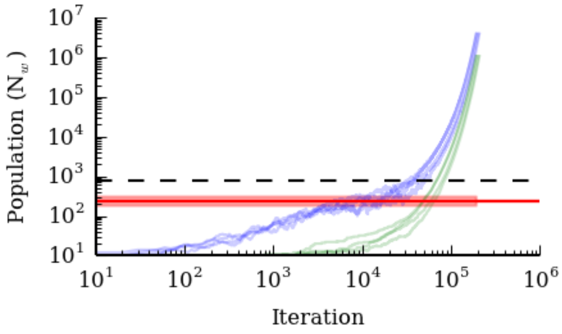


FIG. 115. $U = 0.75$, $N_{\mathrm{dets}} = 1.1\mathrm{e}{+}05$ (22 sites, 6 electrons), $N_{\mathrm{plat}} = 243 \pm 26$ %

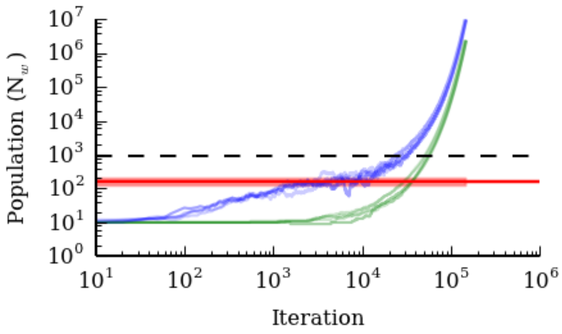


FIG. 116. $U = 0.75$, $N_{\mathrm{dets}} = 2.1\mathrm{e}{+}05$ (16 sites, 8 electrons), $N_{\mathrm{plat}} = 159 \pm 24$ %

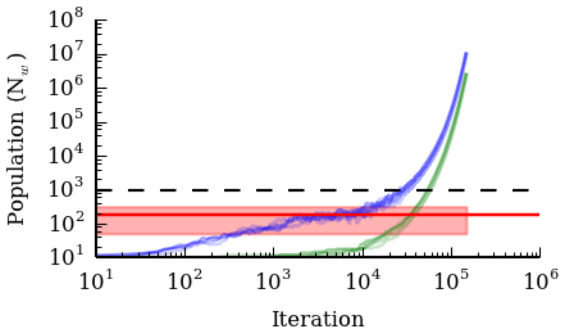


FIG. 117. $U = 0.75$, $N_{\mathrm{dets}} = 2.1\mathrm{e}{+}05$ (16 sites, 24 electrons), $N_{\mathrm{plat}} = 176 \pm 72$ % (manual correction: 200)

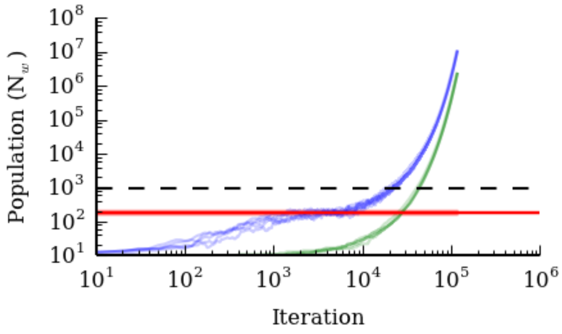


FIG. 118. $U = 0.75$, $N_{\mathrm{dets}} = 2.9\mathrm{e}{+}05$ (14 sites, 18 electrons), $N_{\mathrm{plat}} = 183 \pm 13$ %

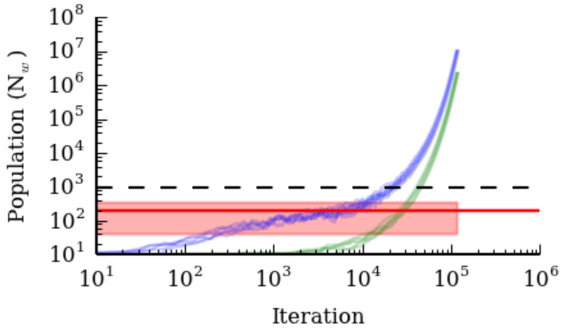


FIG. 119. $U = 0.75$, $N_{\mathrm{dets}} = 2.9\mathrm{e}{+}05$ (14 sites, 10 electrons), $N_{\mathrm{plat}} = 191 \pm 79$ % (manual correction: 150)

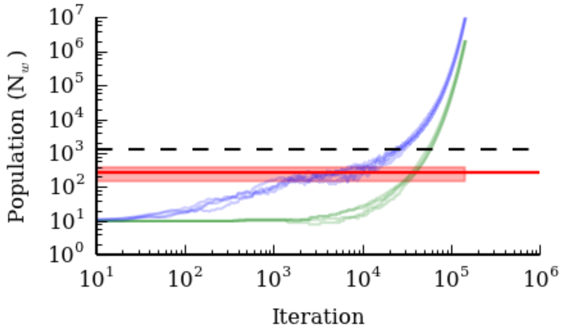


FIG. 120. $U = 0.75$, $N_{\mathrm{dets}} = 5.2\mathrm{e}{+}05$ (18 sites, 8 electrons), $N_{\mathrm{plat}} = 266 \pm 44$ % (manual correction: 200)

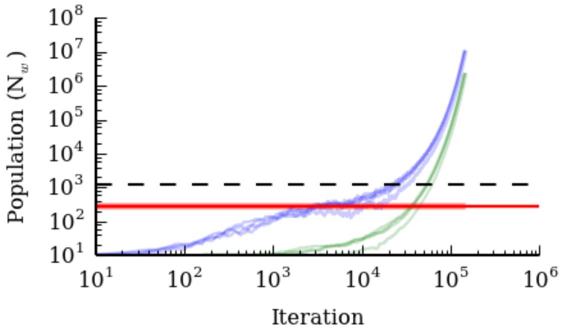


FIG. 121. $U = 0.75$, $N_{\rm dets} = 5.2\text{e+}05$ (18 sites, 28 electrons), $N_{\rm plat} = 285 \pm 14$ %

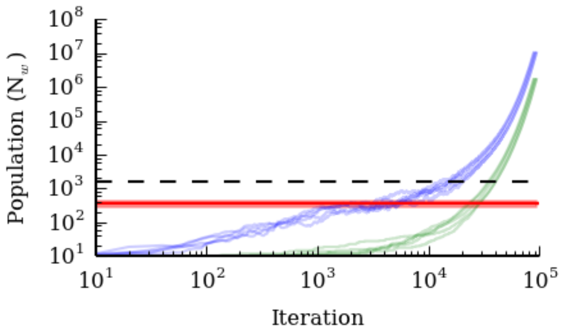


FIG. 122. $U = 0.75$, $N_{\rm dets} = 6.4\text{e+}05$ (14 sites, 16 electrons), $N_{\rm plat} = 356 \pm 20$ %

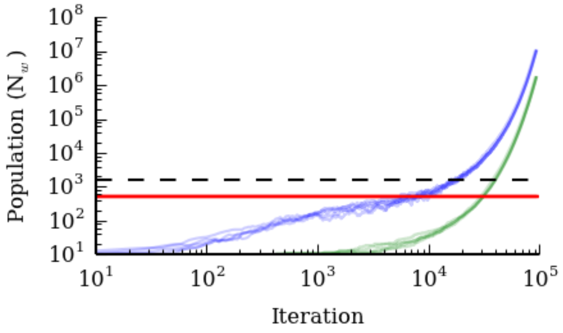


FIG. 123. $U = 0.75$, $N_{\rm dets} = 6.4\text{e+}05$ (14 sites, 12 electrons), $N_{\rm plat} = 526 \pm 5.9$ %

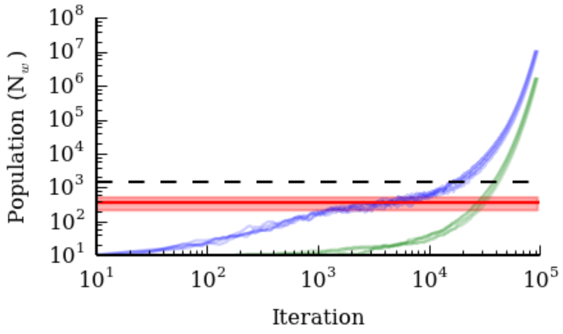


FIG. 124. $U = 0.75$, $N_{\rm dets} = 8.4\text{e+}05$ (14 sites, 14 electrons), $N_{\rm plat} = 365 \pm 41$ % (manual correction: 300)

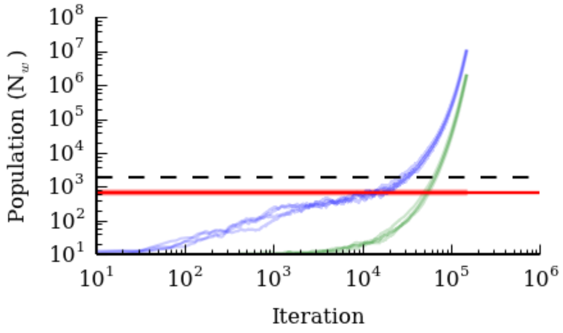


FIG. 125. $U = 0.75$, $N_{\rm dets} = 1.2\text{e+}06$ (20 sites, 32 electrons), $N_{\rm plat} = 687 \pm 13$ %

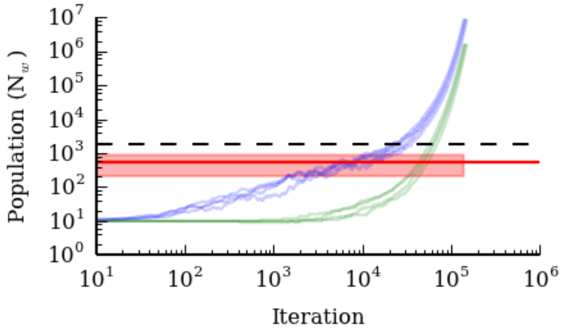


FIG. 126. $U = 0.75$, $N_{\rm dets} = 1.2\text{e+}06$ (20 sites, 8 electrons), $N_{\rm plat} = 545 \pm 61$ % (manual correction: 400)

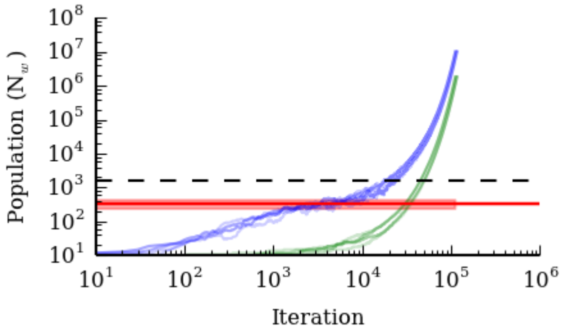


FIG. 127. $U = 0.75$, $N_{\mathrm{dets}} = 1.2\mathrm{e}{+}06$ (16 sites, 10 electrons), $N_{\mathrm{plat}} = 332 \pm 29$ %

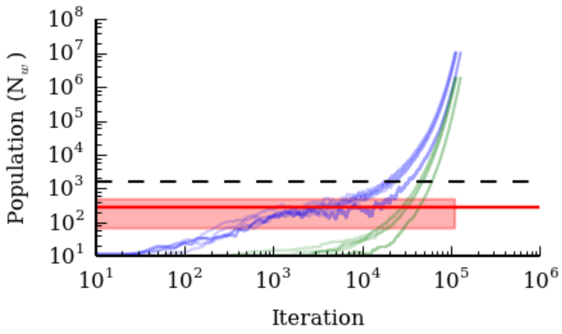


FIG. 128. $U = 0.75$, $N_{\mathrm{dets}} = 1.2\mathrm{e}{+}06$ (16 sites, 22 electrons), $N_{\mathrm{plat}} = 276 \pm 76$ % (manual correction: 400)

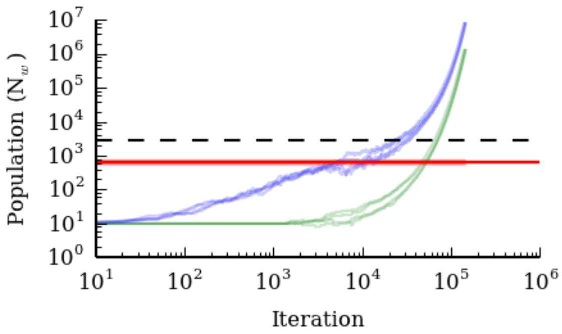


FIG. 129. $U = 0.75$, $N_{\mathrm{dets}} = 2.4\mathrm{e}{+}06$ (22 sites, 8 electrons), $N_{\mathrm{plat}} = 639 \pm 12$ %

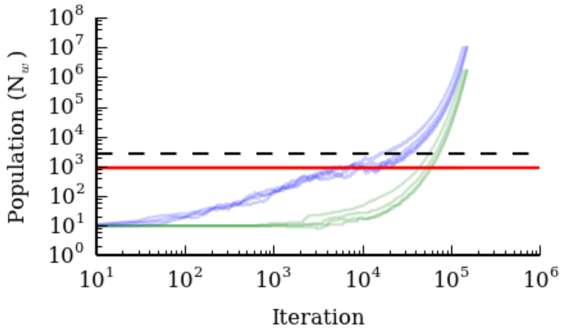


FIG. 130. $U = 0.75$, $N_{\mathrm{dets}} = 2.4\mathrm{e}{+}06$ (22 sites, 36 electrons), $N_{\mathrm{plat}} = 888 \pm 2.4$ %

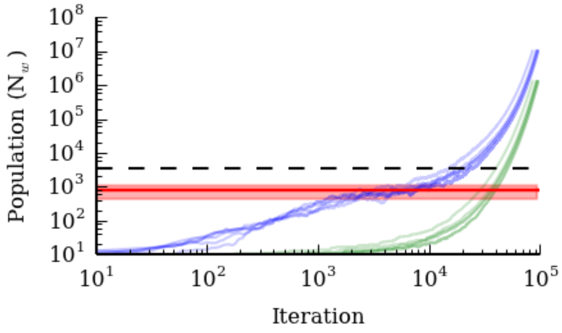


FIG. 131. $U = 0.75$, $N_{\mathrm{dets}} = 4\mathrm{e}{+}06$ (16 sites, 12 electrons), $N_{\mathrm{plat}} = 769 \pm 42$ % (manual correction: 1e+03)

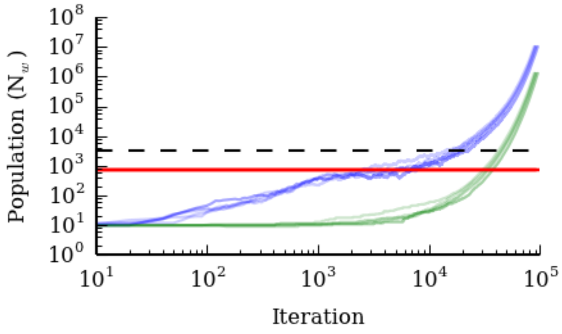


FIG. 132. $U = 0.75$, $N_{\mathrm{dets}} = 4\mathrm{e}{+}06$ (16 sites, 20 electrons), $N_{\mathrm{plat}} = 739 \pm 8.4$ %

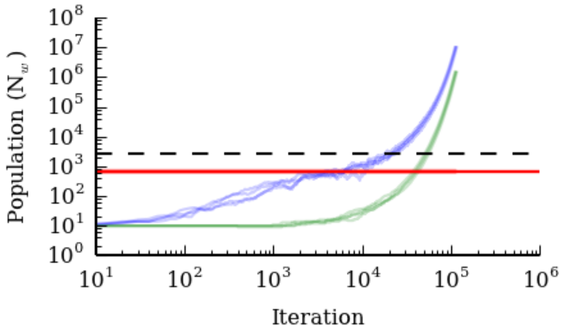


FIG. 133. $U = 0.75$, $N_{\rm dets} = 4.1e{+}06$ (18 sites, 10 electrons), $N_{\rm plat} = 679 \pm 10$ %

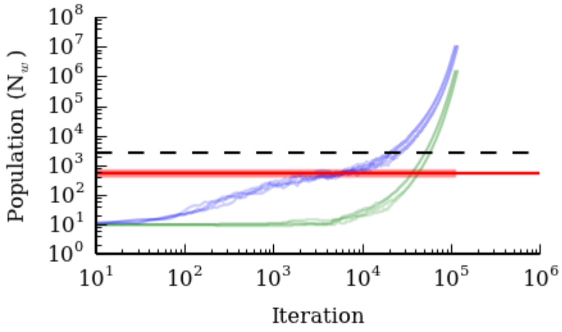


FIG. 134. $U = 0.75$, $N_{\rm dets} = 4.1e{+}06$ (18 sites, 26 electrons), $N_{\rm plat} = 551 \pm 24$ %

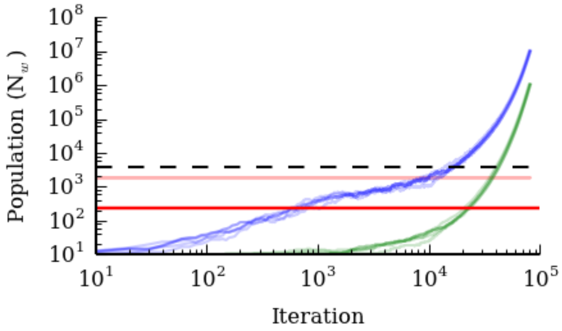


FIG. 135. $U = 0.75$, $N_{\rm dets} = 8.2e{+}06$ (16 sites, 18 electrons), $N_{\rm plat} = 240 \pm 6.7e{+}02$ % (manual correction: 800)

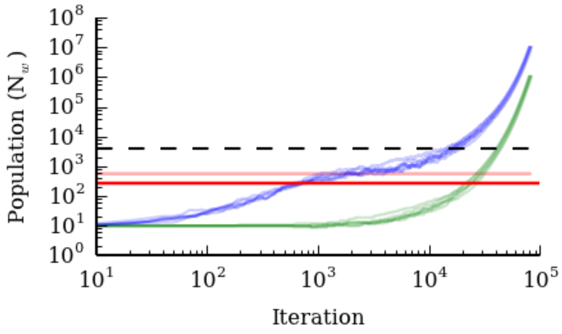


FIG. 136. $U = 0.75$, $N_{\rm dets} = 8.2e{+}06$ (16 sites, 14 electrons), $N_{\rm plat} = 268 \pm 1.1e{+}02$ % (manual correction: 800)

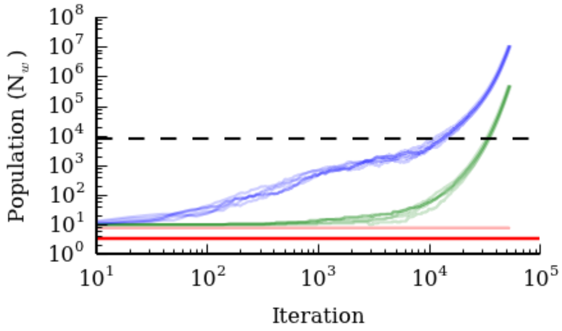


FIG. 137. $U = 0.75$, $N_{\rm dets} = 1e{+}07$ (16 sites, 16 electrons), $N_{\rm plat} = 3.34 \pm 1.3e{+}02$ % (manual correction: 2e+03)

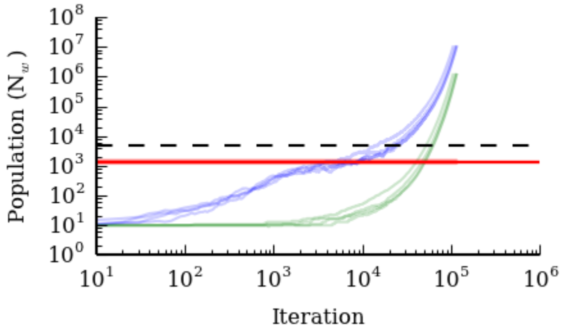


FIG. 138. $U = 0.75$, $N_{\rm dets} = 1.2e{+}07$ (20 sites, 30 electrons), $N_{\rm plat} = 1.38e{+}03 \pm 13$ %

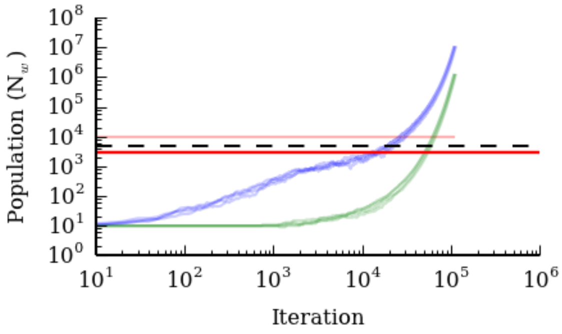


FIG. 139. $U = 0.75$, $N_{\text{dets}} = 1.2\text{e+}07$ (20 sites, 10 electrons), $N_{\text{plat}} = 2.91\text{e+}03 \pm 2.4\text{e+}02$ % (manual correction: 1.5e+03)

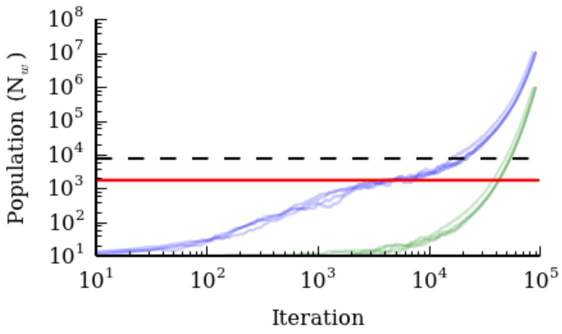


FIG. 140. $U = 0.75$, $N_{\text{dets}} = 1.9\text{e+}07$ (18 sites, 24 electrons), $N_{\text{plat}} = 1.78\text{e+}03 \pm 0$ %

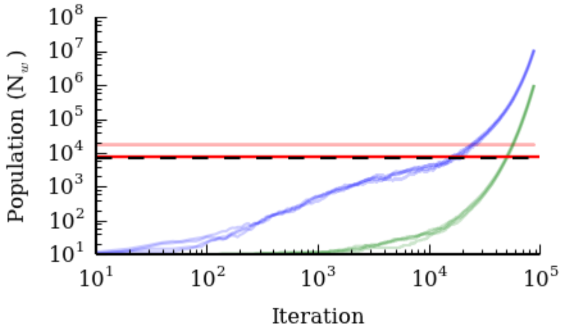


FIG. 141. $U = 0.75$, $N_{\text{dets}} = 1.9\text{e+}07$ (18 sites, 12 electrons), $N_{\text{plat}} = 7.87\text{e+}03 \pm 1.2\text{e+}02$ % (manual correction: 4e+03)

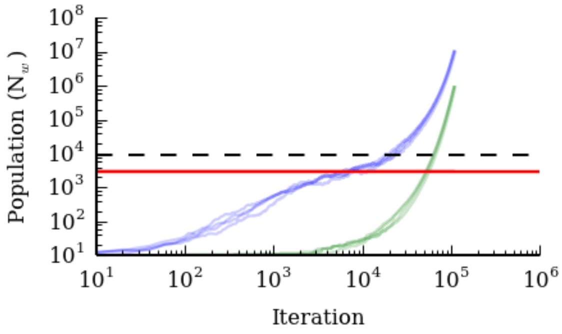


FIG. 142. $U = 0.75$, $N_{\text{dets}} = 3.2\text{e+}07$ (22 sites, 34 electrons), $N_{\text{plat}} = 3.03\text{e+}03 \pm 0$ %

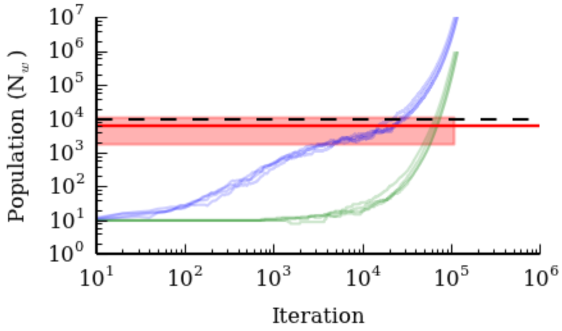


FIG. 143. $U = 0.75$, $N_{\text{dets}} = 3.2\text{e+}07$ (22 sites, 10 electrons), $N_{\text{plat}} = 6.29\text{e+}03 \pm 72$ % (manual correction: 3e+03)

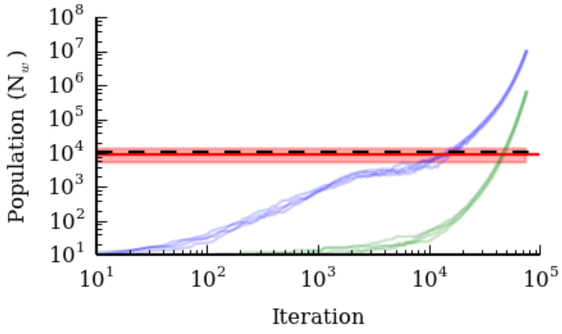


FIG. 144. $U = 0.75$, $N_{\text{dets}} = 5.6\text{e+}07$ (18 sites, 22 electrons), $N_{\text{plat}} = 9.44\text{e+}03 \pm 44$ % (manual correction: 4e+03)

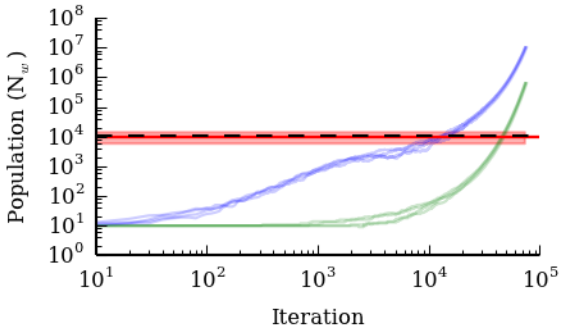


FIG. 145. $U = 0.75$, $N_{\rm dets} = 5.6\text{e+}07$ (18 sites, 14 electrons), $N_{\rm plat} = 9.96\text{e+}03 \pm 42$ % (manual correction: 3e+03)

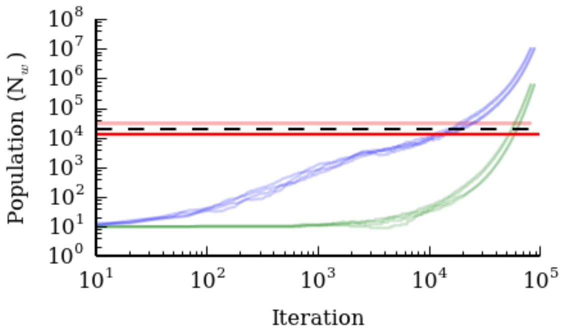


FIG. 146. $U = 0.75$, $N_{\rm dets} = 7.5\text{e+}07$ (20 sites, 28 electrons), $N_{\rm plat} = 1.28\text{e+}04 \pm 1.4\text{e+}02$ % (manual correction: 4e+03)

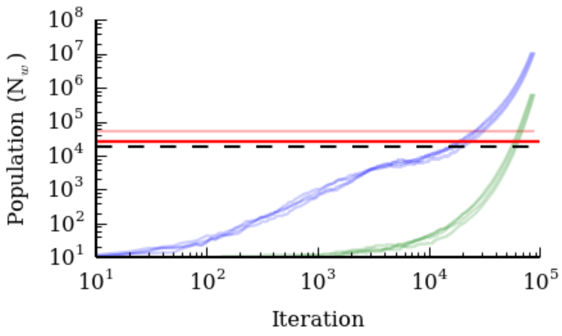


FIG. 147. $U = 0.75$, $N_{\rm dets} = 7.5\text{e+}07$ (20 sites, 12 electrons), $N_{\rm plat} = 2.5\text{e+}04 \pm 1.1\text{e+}02$ % (manual correction: 7e+03)

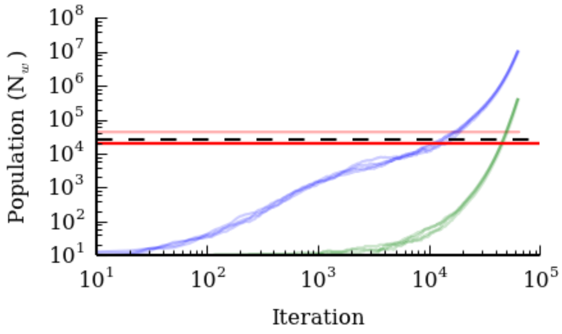


FIG. 148. $U = 0.75$, $N_{\rm dets} = 1.1\text{e+}08$ (18 sites, 20 electrons), $N_{\rm plat} = 2.04\text{e+}04 \pm 1.1\text{e+}02$ % (manual correction: 1e+04)

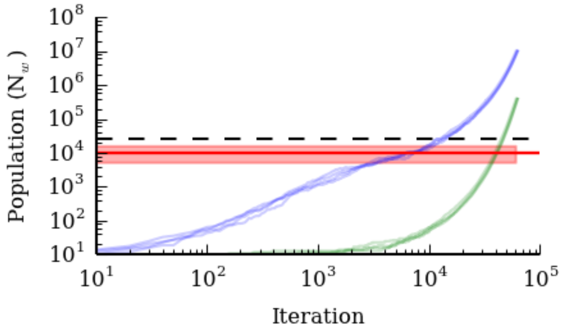


FIG. 149. $U = 0.75$, $N_{\rm dets} = 1.1\text{e+}08$ (18 sites, 16 electrons), $N_{\rm plat} = 1.04\text{e+}04 \pm 51$ % (manual correction: 8e+03)

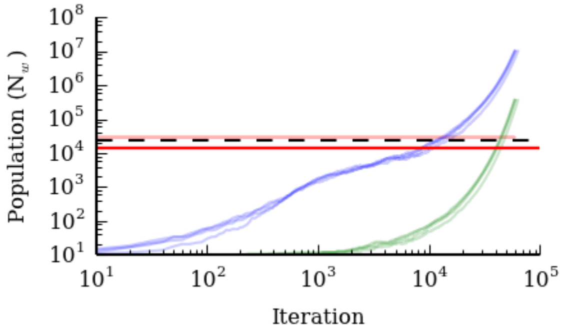


FIG. 150. $U = 0.75$, $N_{\rm dets} = 1.3\text{e+}08$ (18 sites, 18 electrons), $N_{\rm plat} = 1.41\text{e+}04 \pm 1.1\text{e+}02$ % (manual correction: 5e+03)

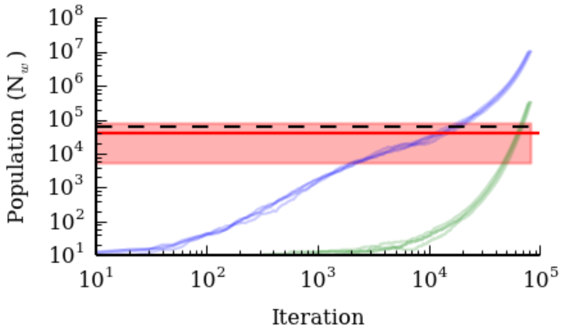


FIG. 151. $U = 0.75$, $N_{\rm dets} = 2.5\text{e}{+}08$ (22 sites, 32 electrons), $N_{\rm plat} = 4.08\text{e}{+}04 \pm 87$ % (manual correction: 2e+04)

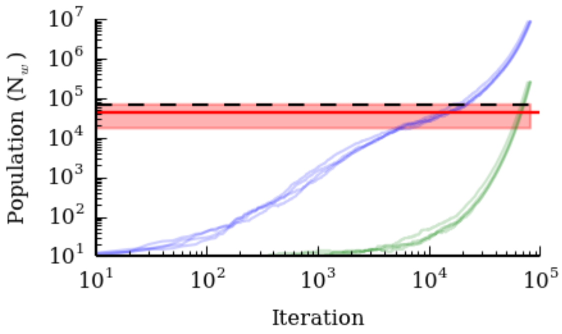


FIG. 152. $U = 0.75$, $N_{\rm dets} = 2.5\text{e}{+}08$ (22 sites, 12 electrons), $N_{\rm plat} = 4.34\text{e}{+}04 \pm 60$ % (manual correction: 2e+04)

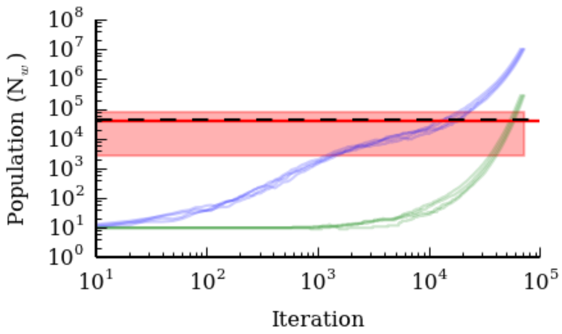


FIG. 153. $U = 0.75$, $N_{\rm dets} = 3\text{e}{+}08$ (20 sites, 14 electrons), $N_{\rm plat} = 4.04\text{e}{+}04 \pm 93$ % (manual correction: 1.5e+04)

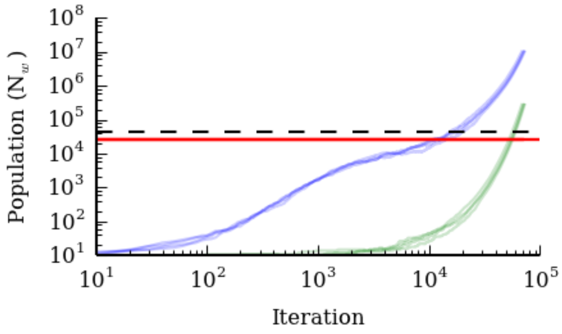


FIG. 154. $U = 0.75$, $N_{\rm dets} = 3\text{e}{+}08$ (20 sites, 26 electrons), $N_{\rm plat} = 2.6\text{e}{+}04 \pm 4.7$ %

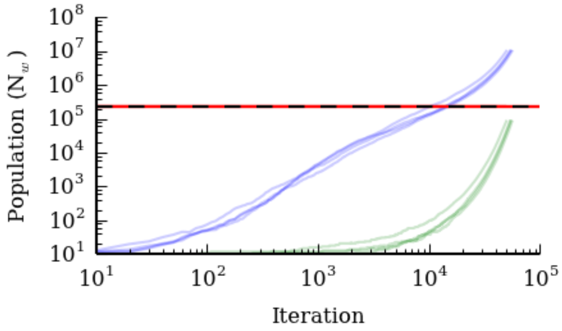


FIG. 155. $U = 0.75$, $N_{\rm dets} = 7.9\text{e}{+}08$ (20 sites, 16 electrons), $N_{\rm plat} = 2.32\text{e}{+}05 \pm 0.18$ %

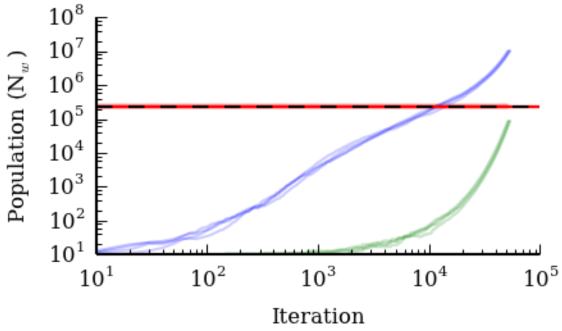


FIG. 156. $U = 0.75$, $N_{\rm dets} = 7.9\text{e}{+}08$ (20 sites, 24 electrons), $N_{\rm plat} = 2.38\text{e}{+}05 \pm 9.1$ %

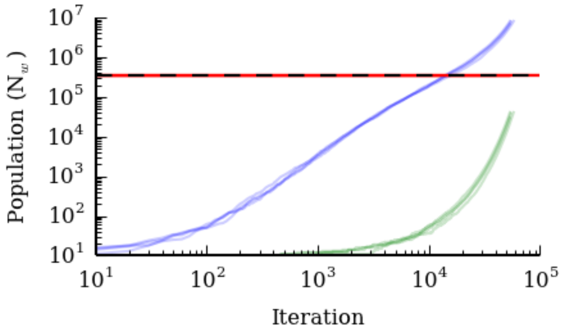


FIG. 157. $U$ = 0.75, $N_{\rm dets}$ = 1.3e+09 (22 sites, 30 electrons), $N_{\rm plat}$ = 3.4e+05 ± 2.4 %

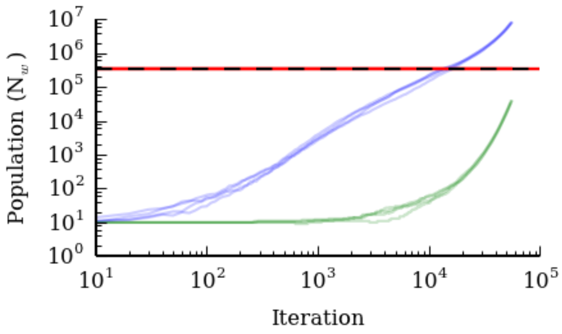


FIG. 158. $U$ = 0.75, $N_{\rm dets}$ = 1.3e+09 (22 sites, 14 electrons), $N_{\rm plat}$ = 3.5e+05 ± 5.1 %

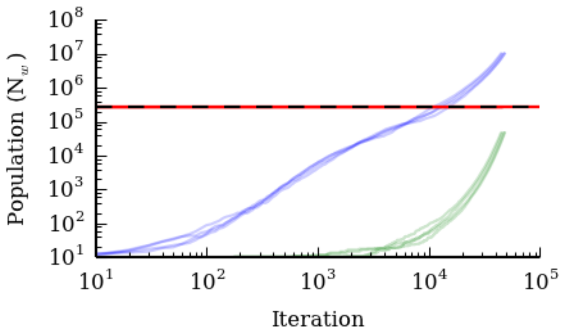


FIG. 159. $U$ = 0.75, $N_{\rm dets}$ = 1.4e+09 (20 sites, 22 electrons), $N_{\rm plat}$ = 2.63e+05 ± 2.5 %

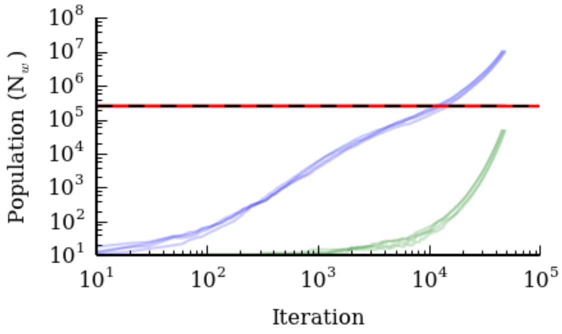


FIG. 160. $U$ = 0.75, $N_{\rm dets}$ = 1.4e+09 (20 sites, 18 electrons), $N_{\rm plat}$ = 2.58e+05 ± 2 %

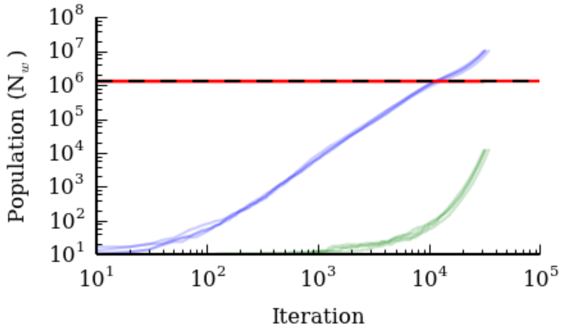


FIG. 161. $U$ = 0.75, $N_{\rm dets}$ = 1.7e+09 (20 sites, 20 electrons), $N_{\rm plat}$ = 1.26e+06 ± 0 %

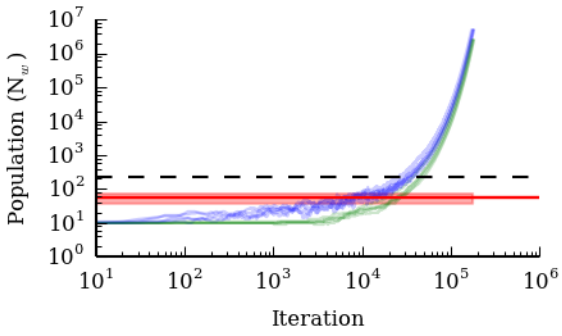


FIG. 162. $U$ = 1.0, $N_{\rm dets}$ = 3.7e+02 (12 sites, 4 electrons), $N_{\rm plat}$ = 55.3 ± 33 % (manual correction: 40)

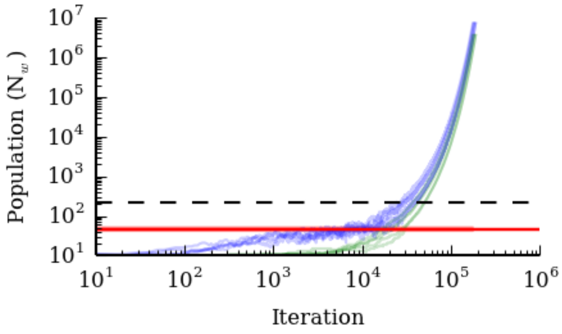


FIG. 163. $U$ = 1.0, $N_{\rm dets}$ = 3.7e+02 (12 sites, 20 electrons), $N_{\rm plat}$ = 46.8 ± 9.7 %

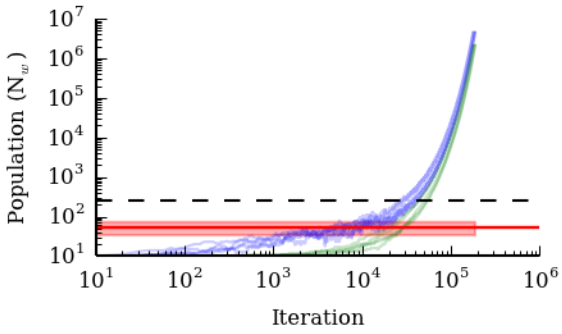


FIG. 164. $U$ = 1.0, $N_{\rm dets}$ = 6e+02 (14 sites, 4 electrons), $N_{\rm plat}$ = 53.3 ± 37 % (manual correction: 40)

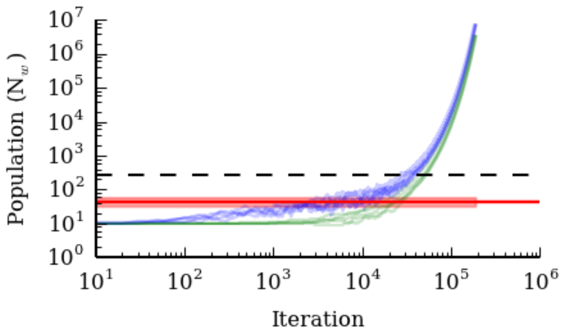


FIG. 165. $U$ = 1.0, $N_{\rm dets}$ = 6e+02 (14 sites, 24 electrons), $N_{\rm plat}$ = 44 ± 29 %

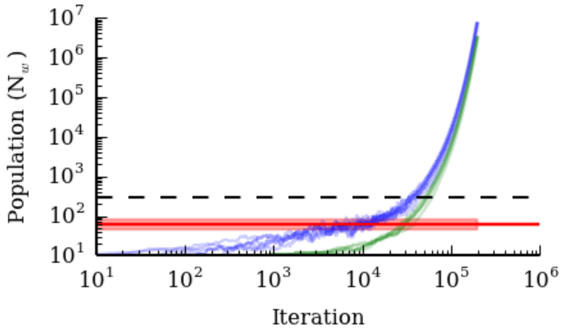


FIG. 166. $U$ = 1.0, $N_{\rm dets}$ = 9e+02 (16 sites, 28 electrons), $N_{\rm plat}$ = 63.5 ± 28 %

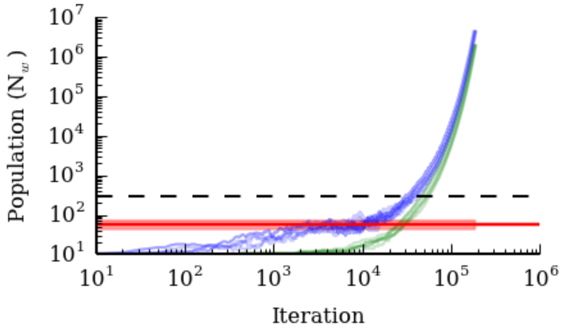


FIG. 167. $U$ = 1.0, $N_{\rm dets}$ = 9e+02 (16 sites, 4 electrons), $N_{\rm plat}$ = 57.5 ± 25 %

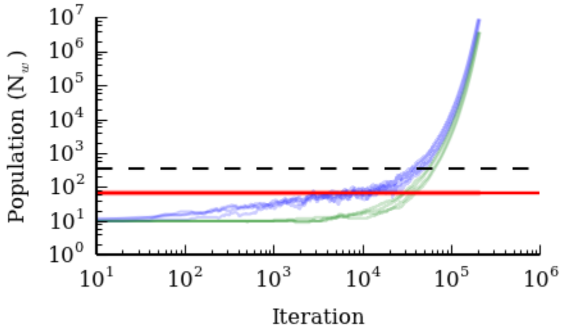


FIG. 168. $U$ = 1.0, $N_{\rm dets}$ = 1.3e+03 (18 sites, 32 electrons), $N_{\rm plat}$ = 67.8 ± 10 %

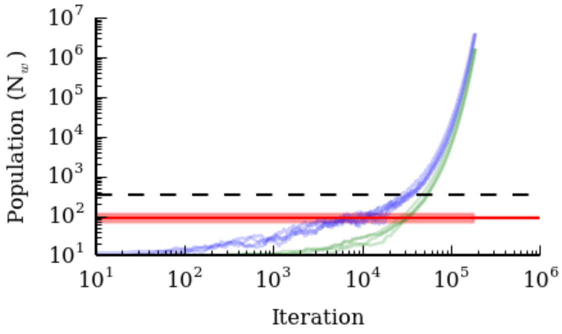


FIG. 169. $U = 1.0$, $N_{\text{dets}} = 1.3\text{e}{+}03$ (18 sites, 4 electrons), $N_{\text{plat}} = 90.9 \pm 24$ %

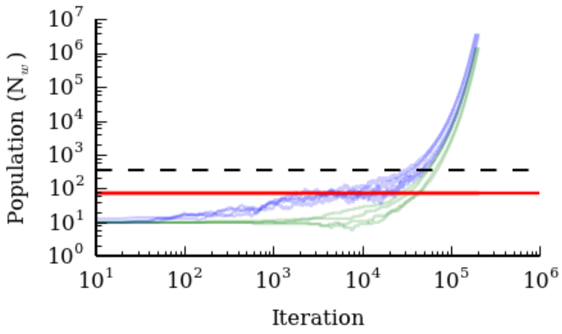


FIG. 170. $U = 1.0$, $N_{\text{dets}} = 1.8\text{e}{+}03$ (20 sites, 4 electrons), $N_{\text{plat}} = 72.6 \pm 7.5$ %

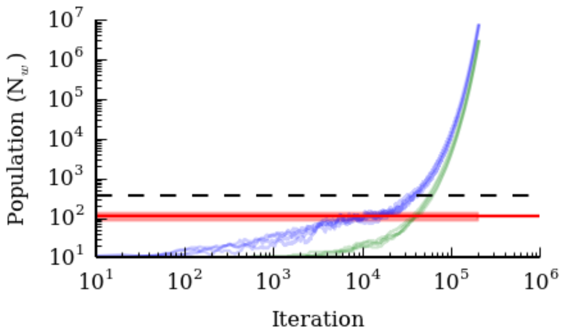


FIG. 171. $U = 1.0$, $N_{\text{dets}} = 1.8\text{e}{+}03$ (20 sites, 36 electrons), $N_{\text{plat}} = 110 \pm 21$ %

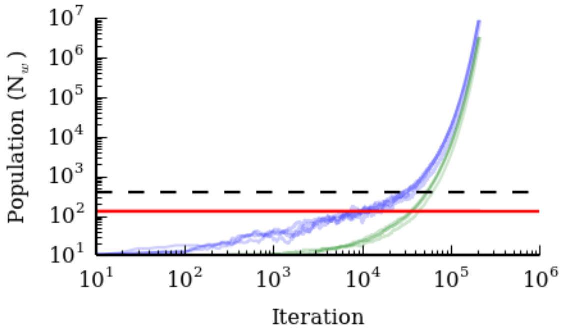


FIG. 172. $U = 1.0$, $N_{\text{dets}} = 2.4\text{e}{+}03$ (22 sites, 40 electrons), $N_{\text{plat}} = 133 \pm 0.31$ %

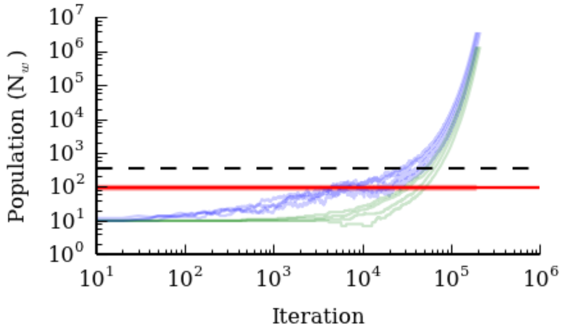


FIG. 173. $U = 1.0$, $N_{\text{dets}} = 2.4\text{e}{+}03$ (22 sites, 4 electrons), $N_{\text{plat}} = 94.3 \pm 12$ %

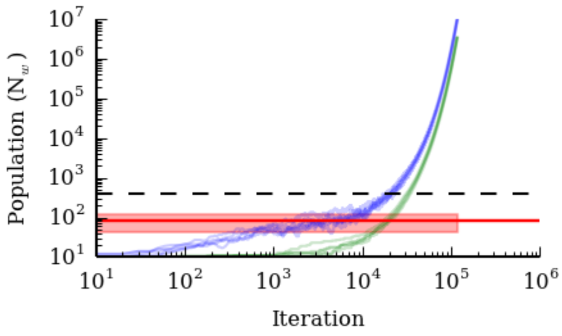


FIG. 174. $U = 1.0$, $N_{\text{dets}} = 4\text{e}{+}03$ (12 sites, 6 electrons), $N_{\text{plat}} = 81.1 \pm 48$ % (manual correction: 100)

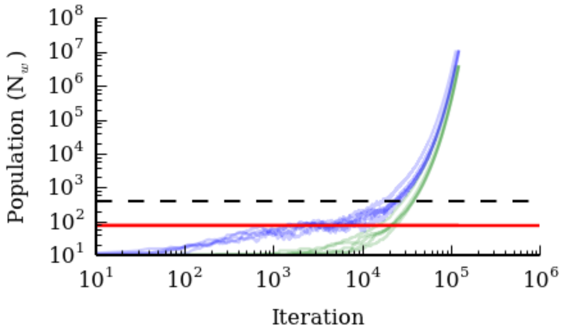


FIG. 175. $U$ = 1.0, $N_{\mathrm{dets}}$ = 4e+03 (12 sites, 18 electrons), $N_{\mathrm{plat}}$ = 79.8 ± 4.5 %

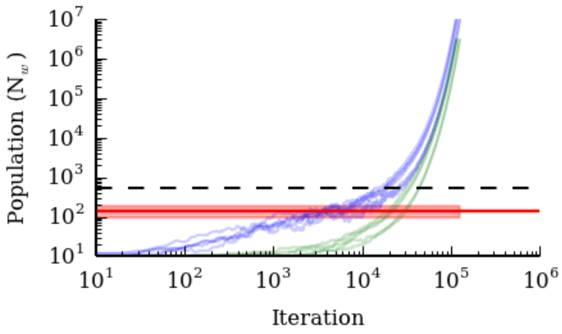


FIG. 176. $U$ = 1.0, $N_{\mathrm{dets}}$ = 9.5e+03 (14 sites, 6 electrons), $N_{\mathrm{plat}}$ = 141 ± 32 % (manual correction: 150)

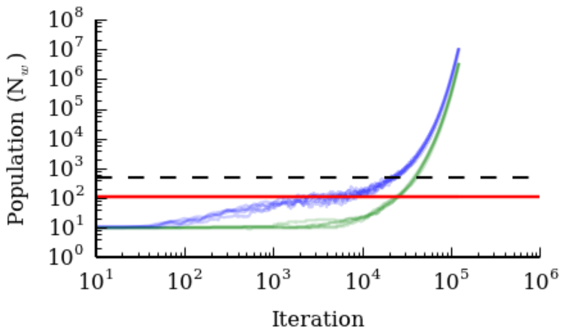


FIG. 177. $U$ = 1.0, $N_{\mathrm{dets}}$ = 9.5e+03 (14 sites, 22 electrons), $N_{\mathrm{plat}}$ = 111 ± 1.8 %

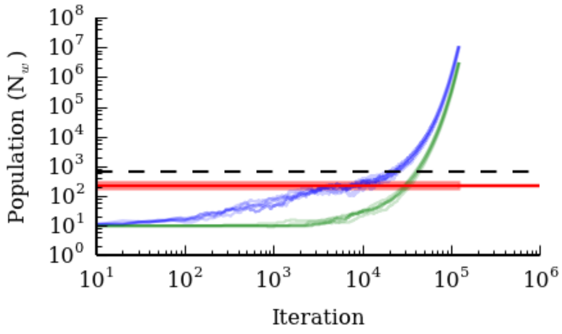


FIG. 178. $U$ = 1.0, $N_{\mathrm{dets}}$ = 2e+04 (16 sites, 26 electrons), $N_{\mathrm{plat}}$ = 233 ± 28 %

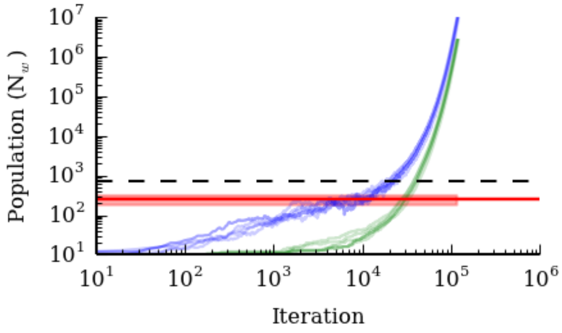


FIG. 179. $U$ = 1.0, $N_{\mathrm{dets}}$ = 2e+04 (16 sites, 6 electrons), $N_{\mathrm{plat}}$ = 246 ± 27 %

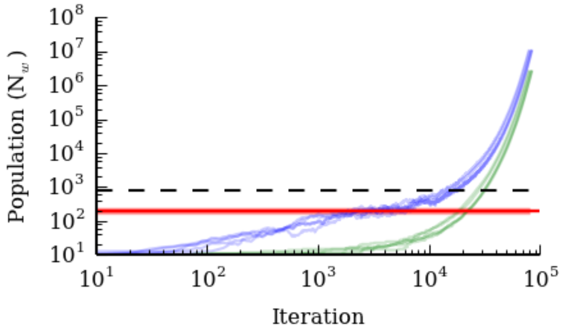


FIG. 180. $U$ = 1.0, $N_{\mathrm{dets}}$ = 2e+04 (12 sites, 8 electrons), $N_{\mathrm{plat}}$ = 195 ± 15 %

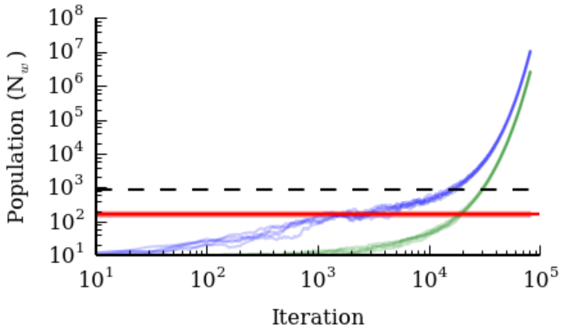


FIG. 181. $U$ = 1.0, $N_{\rm dets}$ = 2e+04 (12 sites, 16 electrons), $N_{\rm plat}$ = 164 ± 15 %

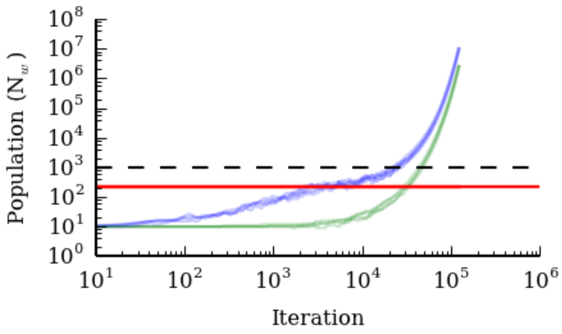


FIG. 182. $U$ = 1.0, $N_{\rm dets}$ = 3.7e+04 (18 sites, 30 electrons), $N_{\rm plat}$ = 220 ± 6.4 %

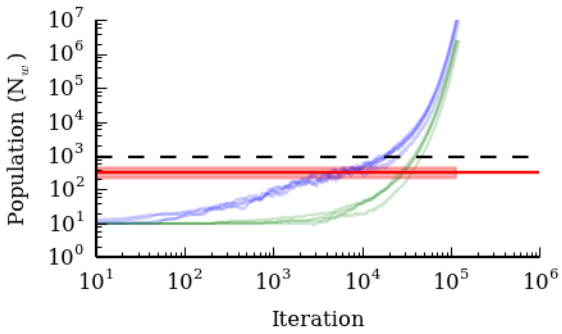


FIG. 183. $U$ = 1.0, $N_{\rm dets}$ = 3.7e+04 (18 sites, 6 electrons), $N_{\rm plat}$ = 329 ± 33 % (manual correction: 400)

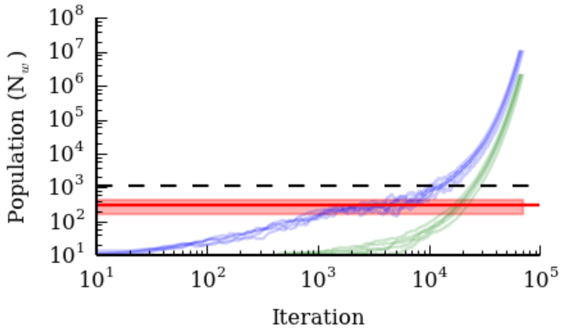


FIG. 184. $U$ = 1.0, $N_{\rm dets}$ = 5.2e+04 (12 sites, 10 electrons), $N_{\rm plat}$ = 301 ± 45 % (manual correction: 300)

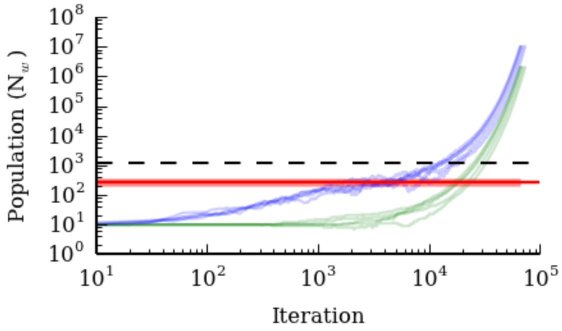


FIG. 185. $U$ = 1.0, $N_{\rm dets}$ = 5.2e+04 (12 sites, 14 electrons), $N_{\rm plat}$ = 267 ± 23 %

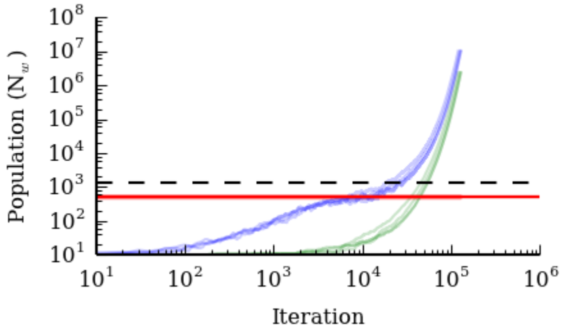


FIG. 186. $U$ = 1.0, $N_{\rm dets}$ = 6.5e+04 (20 sites, 34 electrons), $N_{\rm plat}$ = 511 ± 9.9 %

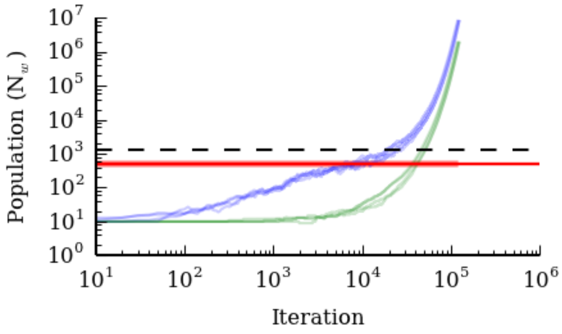


FIG. 187. $U = 1.0$, $N_{\text{dets}} = 6.5\text{e}{+}04$ (20 sites, 6 electrons), $N_{\text{plat}} = 505 \pm 15$ %

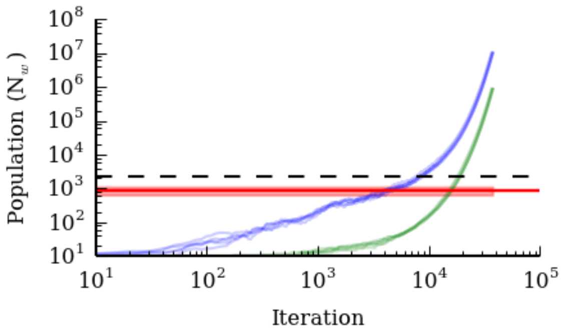


FIG. 188. $U = 1.0$, $N_{\text{dets}} = 7.1\text{e}{+}04$ (12 sites, 12 electrons), $N_{\text{plat}} = 846 \pm 27$ %

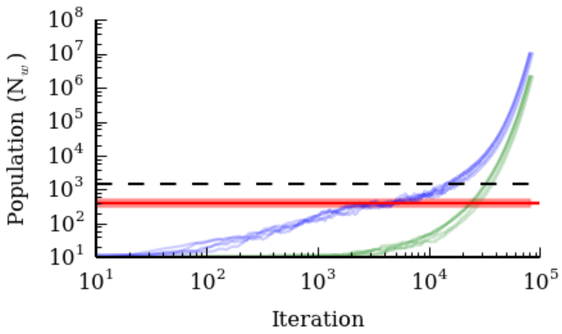


FIG. 189. $U = 1.0$, $N_{\text{dets}} = 7.2\text{e}{+}04$ (14 sites, 8 electrons), $N_{\text{plat}} = 411 \pm 24$ %

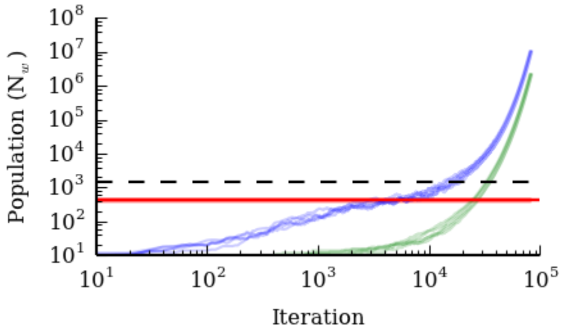


FIG. 190. $U = 1.0$, $N_{\text{dets}} = 7.2\text{e}{+}04$ (14 sites, 20 electrons), $N_{\text{plat}} = 428 \pm 11$ %

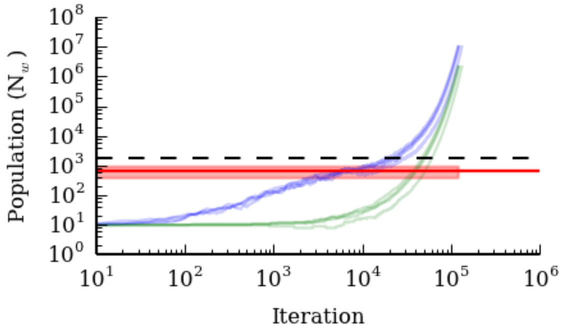


FIG. 191. $U = 1.0$, $N_{\text{dets}} = 1.1\text{e}{+}05$ (22 sites, 38 electrons), $N_{\text{plat}} = 652 \pm 42$ % (manual correction: 700)

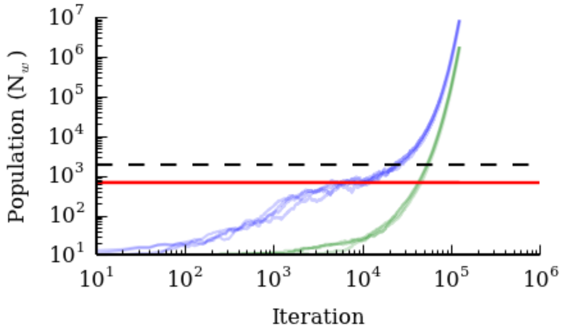


FIG. 192. $U = 1.0$, $N_{\text{dets}} = 1.1\text{e}{+}05$ (22 sites, 6 electrons), $N_{\text{plat}} = 688 \pm 2.3$ %

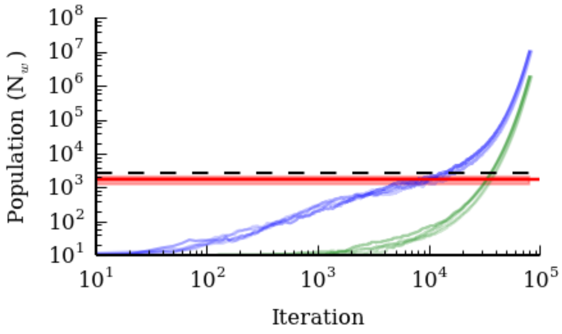


FIG. 193. $U = 1.0$, $N_{\rm dets} = 2.1\text{e+}05$ (16 sites, 8 electrons), $N_{\rm plat} = 1.68\text{e+}03 \pm 25$ %

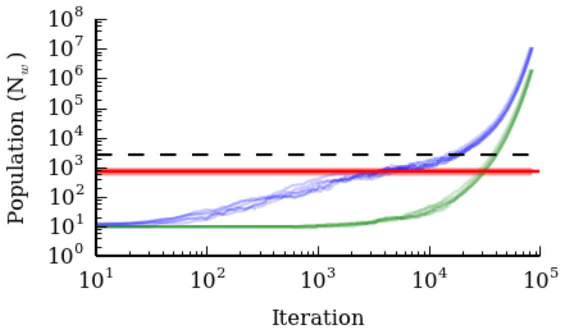


FIG. 194. $U = 1.0$, $N_{\rm dets} = 2.1\text{e+}05$ (16 sites, 24 electrons), $N_{\rm plat} = 731 \pm 22$ %

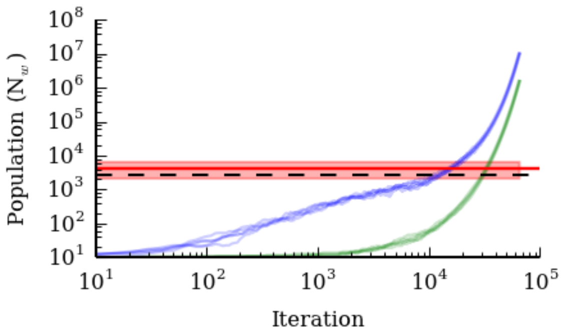


FIG. 195. $U = 1.0$, $N_{\rm dets} = 2.9\text{e+}05$ (14 sites, 18 electrons), $N_{\rm plat} = 4.29\text{e+}03 \pm 51$ % (manual correction: 1e+03)

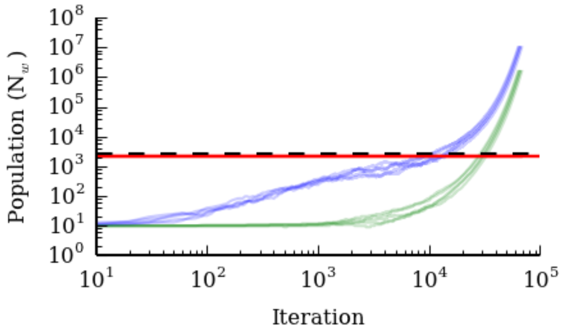


FIG. 196. $U = 1.0$, $N_{\rm dets} = 2.9\text{e+}05$ (14 sites, 10 electrons), $N_{\rm plat} = 2.18\text{e+}03 \pm 4.6$ %

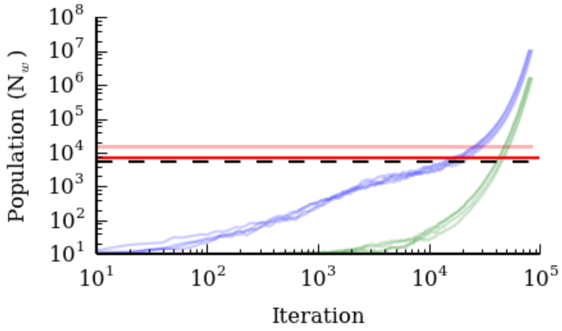


FIG. 197. $U = 1.0$, $N_{\rm dets} = 5.2\text{e+}05$ (18 sites, 8 electrons), $N_{\rm plat} = 7.15\text{e+}03 \pm 1.1\text{e+}02$ % (manual correction: 2e+03)

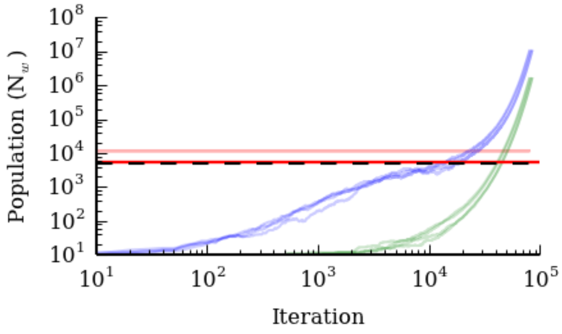


FIG. 198. $U = 1.0$, $N_{\rm dets} = 5.2\text{e+}05$ (18 sites, 28 electrons), $N_{\rm plat} = 5.31\text{e+}03 \pm 1.2\text{e+}02$ % (manual correction: 3e+03)

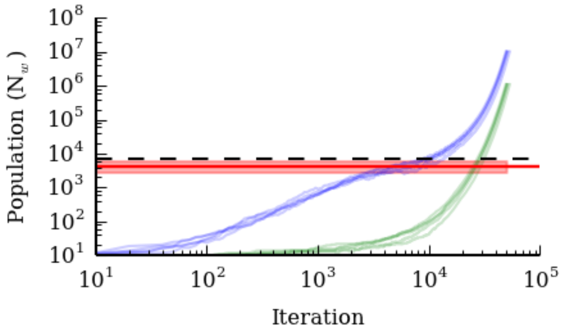


FIG. 199. $U$ = 1.0, $N_{\rm dets}$ = 6.4e+05 (14 sites, 16 electrons), $N_{\rm plat}$ = 4.3e+03 ± 37 % (manual correction: 4e+03)

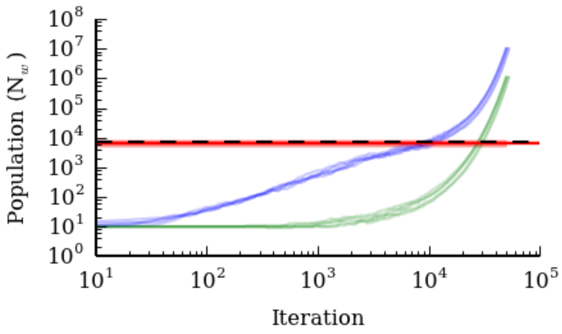


FIG. 200. $U$ = 1.0, $N_{\rm dets}$ = 6.4e+05 (14 sites, 12 electrons), $N_{\rm plat}$ = 6.39e+03 ± 20 %

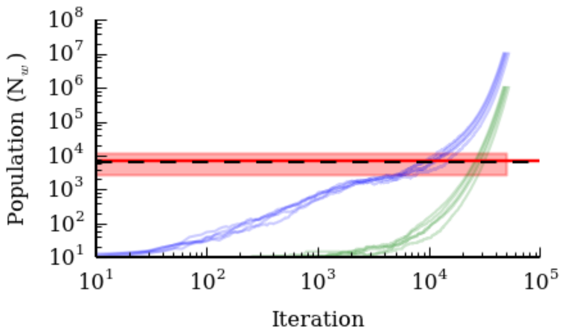


FIG. 201. $U$ = 1.0, $N_{\rm dets}$ = 8.4e+05 (14 sites, 14 electrons), $N_{\rm plat}$ = 7.03e+03 ± 62 % (manual correction: 2e+03)

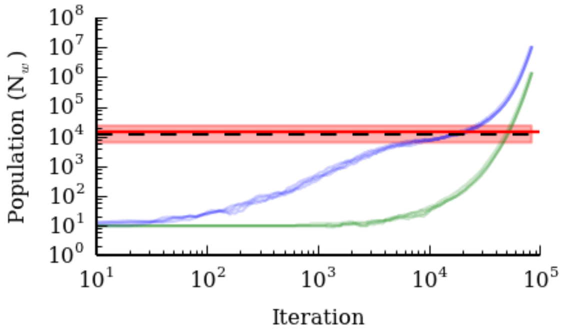


FIG. 202. $U$ = 1.0, $N_{\rm dets}$ = 1.2e+06 (20 sites, 32 electrons), $N_{\rm plat}$ = 1.48e+04 ± 58 % (manual correction: 8e+03)

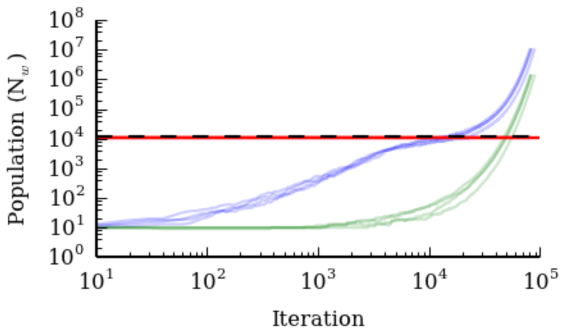


FIG. 203. $U$ = 1.0, $N_{\rm dets}$ = 1.2e+06 (20 sites, 8 electrons), $N_{\rm plat}$ = 1.12e+04 ± 6.1 %

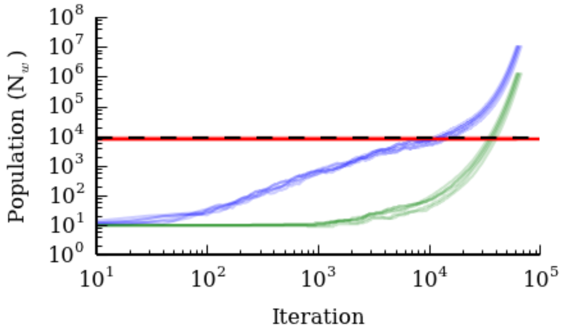


FIG. 204. $U$ = 1.0, $N_{\rm dets}$ = 1.2e+06 (16 sites, 10 electrons), $N_{\rm plat}$ = 8.27e+03 ± 9.5 %

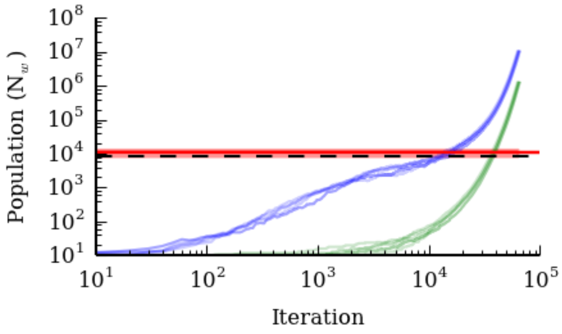


FIG. 205. $U$ = 1.0, $N_{\mathrm{dets}}$ = 1.2e+06 (16 sites, 22 electrons), $N_{\mathrm{plat}}$ = 1.05e+04 ± 24 %

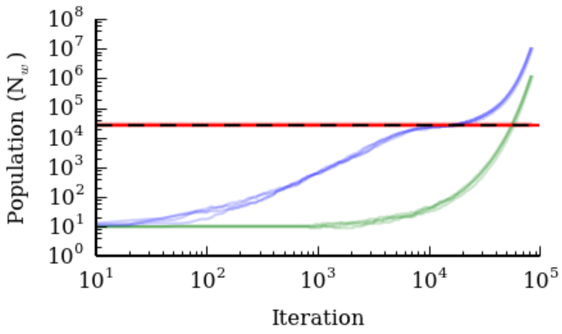


FIG. 206. $U$ = 1.0, $N_{\mathrm{dets}}$ = 2.4e+06 (22 sites, 8 electrons), $N_{\mathrm{plat}}$ = 2.77e+04 ± 8.2 %

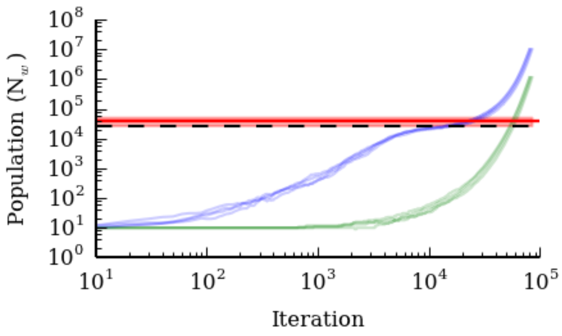


FIG. 207. $U$ = 1.0, $N_{\mathrm{dets}}$ = 2.4e+06 (22 sites, 36 electrons), $N_{\mathrm{plat}}$ = 3.8e+04 ± 31 % (manual correction: 2e+04)

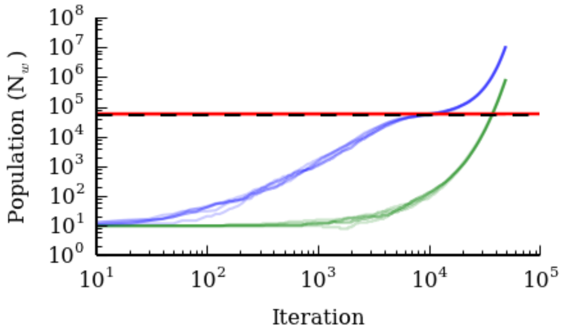


FIG. 208. $U$ = 1.0, $N_{\mathrm{dets}}$ = 4e+06 (16 sites, 12 electrons), $N_{\mathrm{plat}}$ = 5.7e+04 ± 1.6 %

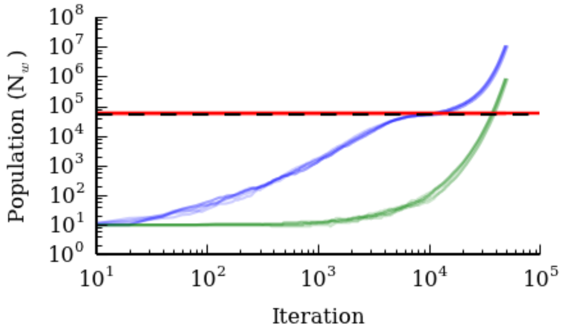


FIG. 209. $U$ = 1.0, $N_{\mathrm{dets}}$ = 4e+06 (16 sites, 20 electrons), $N_{\mathrm{plat}}$ = 5.64e+04 ± 7.1 %

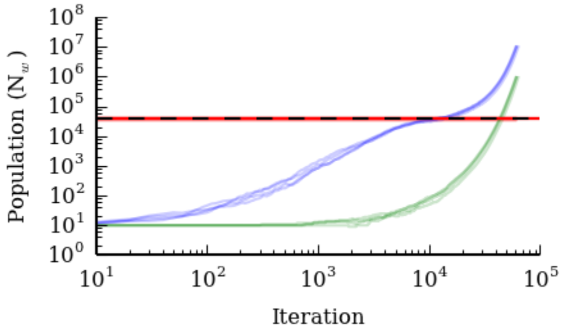


FIG. 210. $U$ = 1.0, $N_{\mathrm{dets}}$ = 4.1e+06 (18 sites, 10 electrons), $N_{\mathrm{plat}}$ = 3.75e+04 ± 10 %

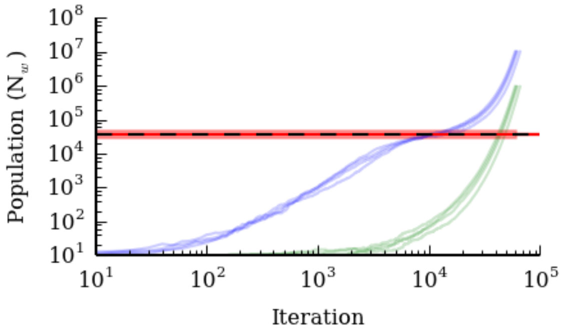


FIG. 211. $U$ = 1.0, $N_{\mathrm{dets}}$ = 4.1e+06 (18 sites, 26 electrons), $N_{\mathrm{plat}}$ = 3.78e+04 ± 25 %

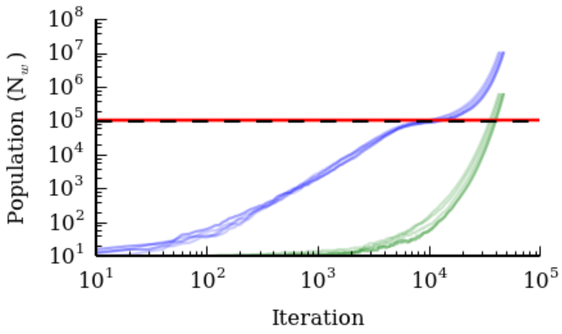


FIG. 212. $U$ = 1.0, $N_{\mathrm{dets}}$ = 8.2e+06 (16 sites, 18 electrons), $N_{\mathrm{plat}}$ = 1.03e+05 ± 0.00033 %

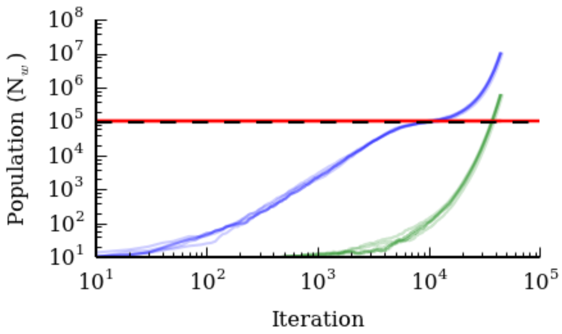


FIG. 213. $U$ = 1.0, $N_{\mathrm{dets}}$ = 8.2e+06 (16 sites, 14 electrons), $N_{\mathrm{plat}}$ = 1.05e+05 ± 3.8 %

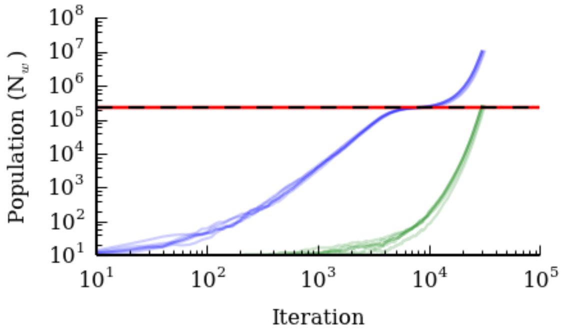


FIG. 214. $U$ = 1.0, $N_{\mathrm{dets}}$ = 1e+07 (16 sites, 16 electrons), $N_{\mathrm{plat}}$ = 2.26e+05 ± 0.23 %

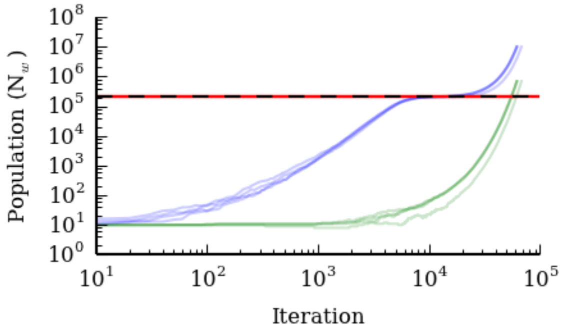


FIG. 215. $U$ = 1.0, $N_{\mathrm{dets}}$ = 1.2e+07 (20 sites, 30 electrons), $N_{\mathrm{plat}}$ = 2.11e+05 ± 0.93 %

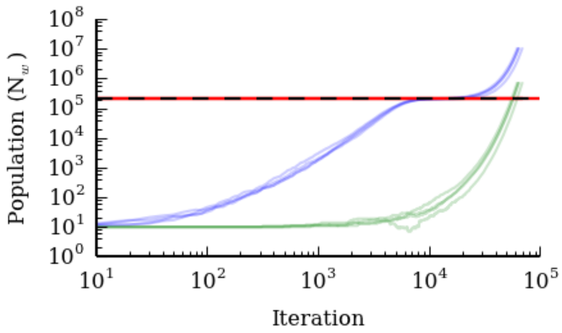


FIG. 216. $U$ = 1.0, $N_{\mathrm{dets}}$ = 1.2e+07 (20 sites, 10 electrons), $N_{\mathrm{plat}}$ = 2.12e+05 ± 4.3 %

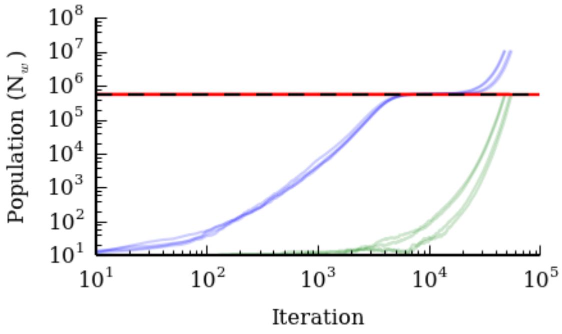


FIG. 217. $U$ = 1.0, $N_{\mathrm{dets}}$ = 1.9e+07 (18 sites, 24 electrons), $N_{\mathrm{plat}}$ = 5.67e+05 ± 0.48 %

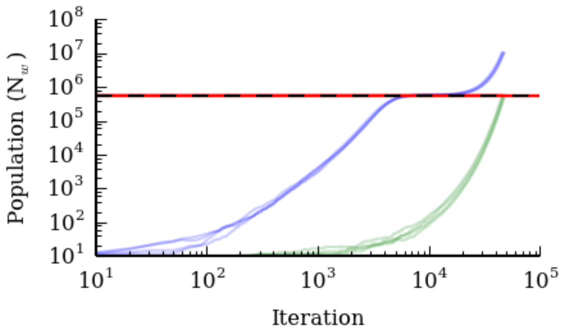


FIG. 218. $U$ = 1.0, $N_{\mathrm{dets}}$ = 1.9e+07 (18 sites, 12 electrons), $N_{\mathrm{plat}}$ = 5.68e+05 ± 0.45 %

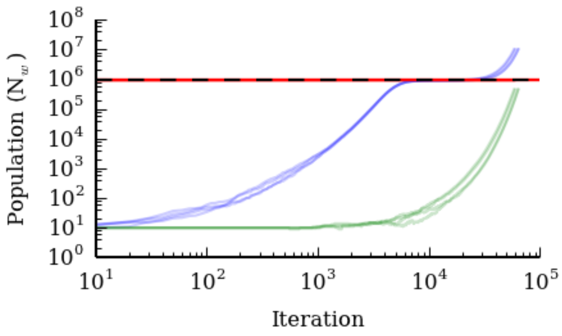


FIG. 219. $U$ = 1.0, $N_{\mathrm{dets}}$ = 3.2e+07 (22 sites, 34 electrons), $N_{\mathrm{plat}}$ = 9.11e+05 ± 0.13 %

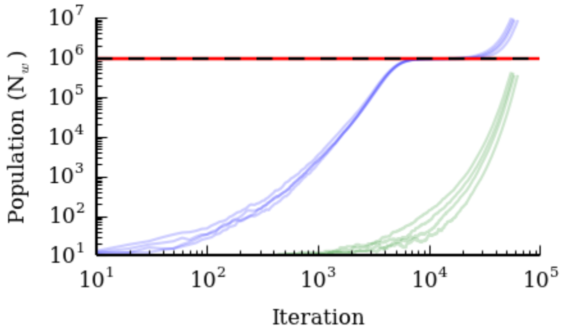


FIG. 220. $U$ = 1.0, $N_{\mathrm{dets}}$ = 3.2e+07 (22 sites, 10 electrons), $N_{\mathrm{plat}}$ = 9.18e+05 ± 3 %

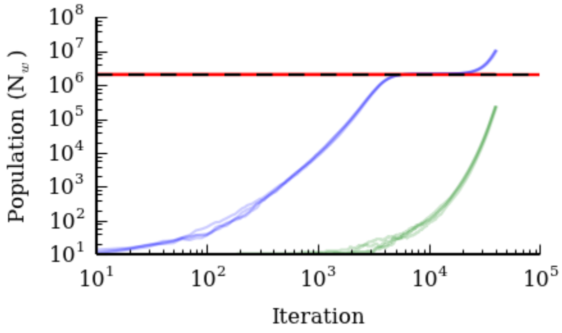


FIG. 221. $U$ = 1.0, $N_{\mathrm{dets}}$ = 5.6e+07 (18 sites, 22 electrons), $N_{\mathrm{plat}}$ = 2.09e+06 ± 0.16 %

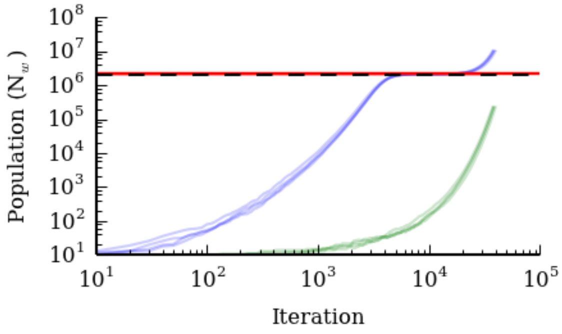


FIG. 222. $U$ = 1.0, $N_{\mathrm{dets}}$ = 5.6e+07 (18 sites, 14 electrons), $N_{\mathrm{plat}}$ = 2.11e+06 ± 0.076 %

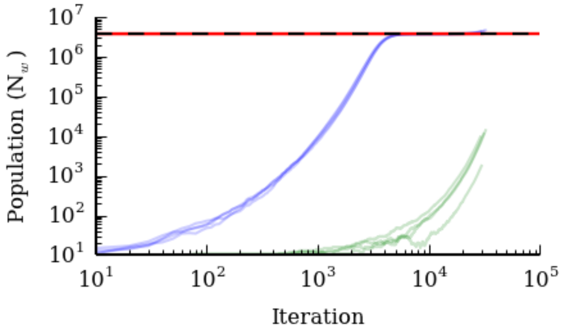


FIG. 223. $U$ = 1.0, $N_{\text{dets}}$ = 7.5e+07 (20 sites, 28 electrons), $N_{\text{plat}}$ = 3.77e+06 ± 0.11 %

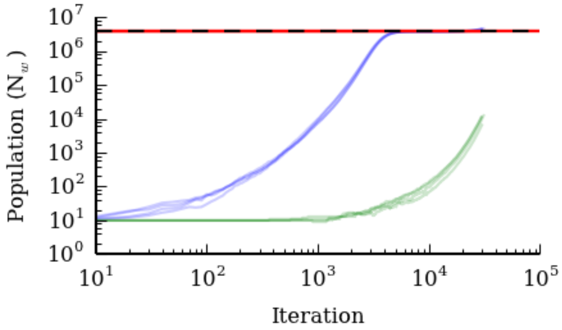


FIG. 224. $U$ = 1.0, $N_{\text{dets}}$ = 7.5e+07 (20 sites, 12 electrons), $N_{\text{plat}}$ = 3.77e+06 ± 0.048 %

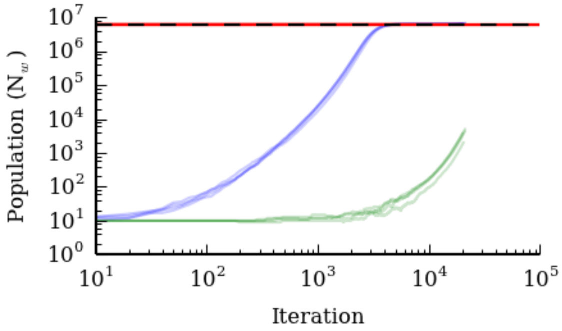


FIG. 225. $U$ = 1.0, $N_{\text{dets}}$ = 1.1e+08 (18 sites, 20 electrons), $N_{\text{plat}}$ = 6.2e+06 ± 0.048 %

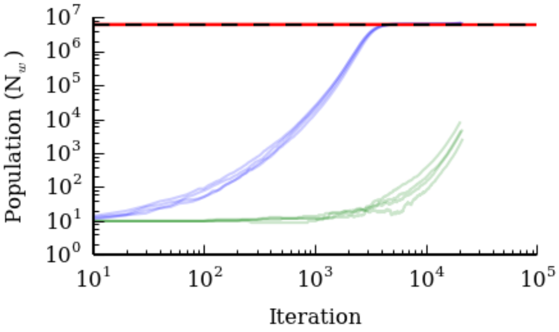


FIG. 226. $U$ = 1.0, $N_{\text{dets}}$ = 1.1e+08 (18 sites, 16 electrons), $N_{\text{plat}}$ = 6.2e+06 ± 0.27 %

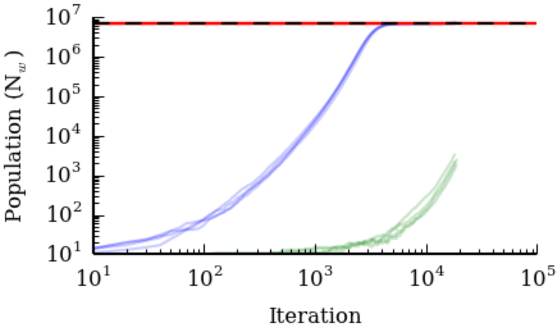


FIG. 227. $U$ = 1.0, $N_{\text{dets}}$ = 1.3e+08 (18 sites, 18 electrons), $N_{\text{plat}}$ = 6.85e+06 ± 0.51 %

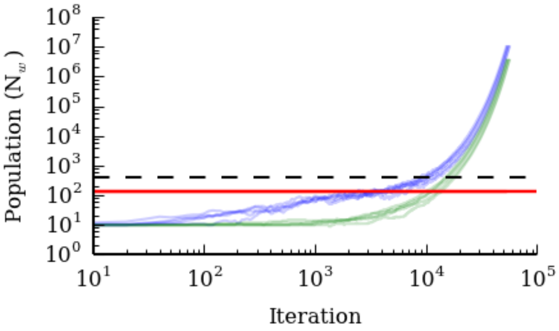


FIG. 228. $U$ = 2.0, $N_{\text{dets}}$ = 3.7e+02 (12 sites, 4 electrons), $N_{\text{plat}}$ = 133 ± 3.5 %

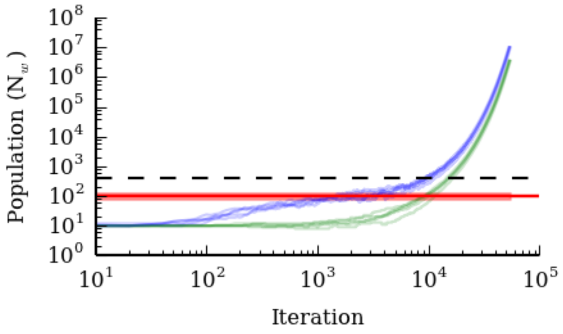


FIG. 229. $U = 2.0$, $N_{\rm dets} = 3.7\text{e}{+}02$ (12 sites, 20 electrons), $N_{\rm plat} = 99.3 \pm 24$ %

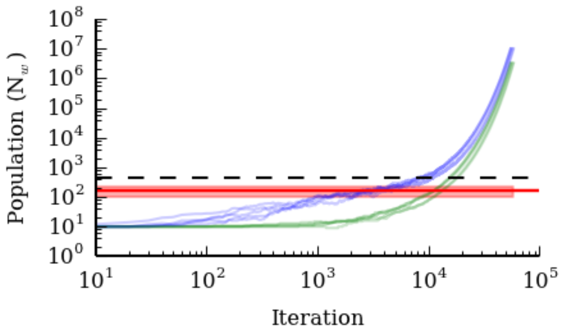


FIG. 230. $U = 2.0$, $N_{\rm dets} = 6\text{e}{+}02$ (14 sites, 4 electrons), $N_{\rm plat} = 163 \pm 38$ % (manual correction: 200)

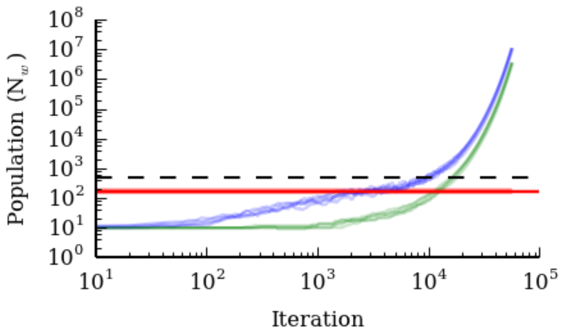


FIG. 231. $U = 2.0$, $N_{\rm dets} = 6\text{e}{+}02$ (14 sites, 24 electrons), $N_{\rm plat} = 174 \pm 14$ %

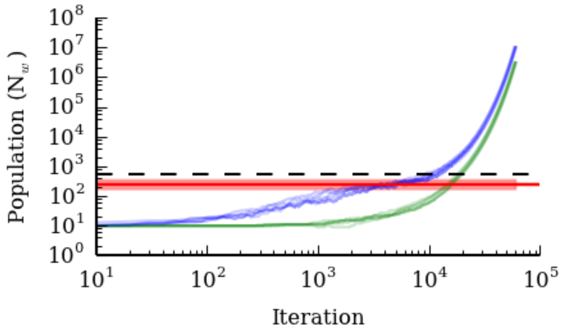


FIG. 232. $U = 2.0$, $N_{\rm dets} = 9\text{e}{+}02$ (16 sites, 28 electrons), $N_{\rm plat} = 257 \pm 33$ % (manual correction: 300)

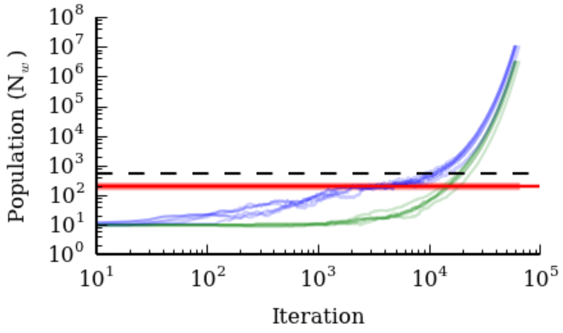


FIG. 233. $U = 2.0$, $N_{\rm dets} = 9\text{e}{+}02$ (16 sites, 4 electrons), $N_{\rm plat} = 204 \pm 21$ %

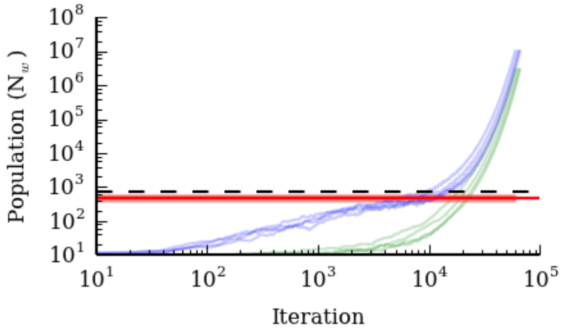


FIG. 234. $U = 2.0$, $N_{\rm dets} = 1.3\text{e}{+}03$ (18 sites, 32 electrons), $N_{\rm plat} = 473 \pm 20$ %

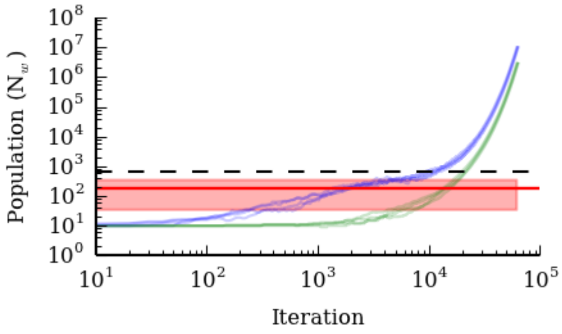


FIG. 235. $U = 2.0$, $N_{\mathrm{dets}} = 1.3\mathrm{e}{+}03$ (18 sites, 4 electrons), $N_{\mathrm{plat}} = 191 \pm 82$ % (manual correction: 400)

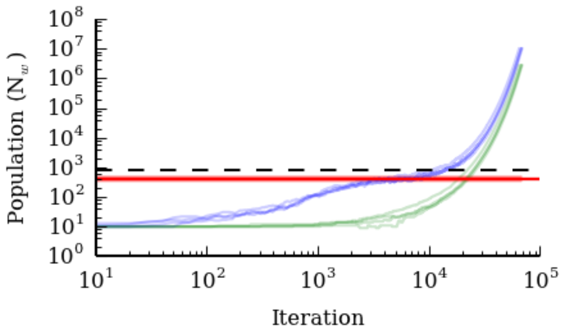


FIG. 236. $U = 2.0$, $N_{\mathrm{dets}} = 1.8\mathrm{e}{+}03$ (20 sites, 4 electrons), $N_{\mathrm{plat}} = 417 \pm 16$ %

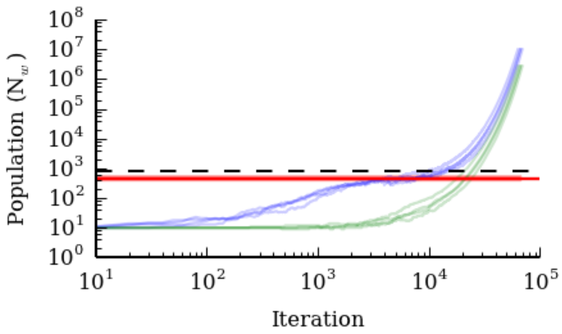


FIG. 237. $U = 2.0$, $N_{\mathrm{dets}} = 1.8\mathrm{e}{+}03$ (20 sites, 36 electrons), $N_{\mathrm{plat}} = 470 \pm 16$ %

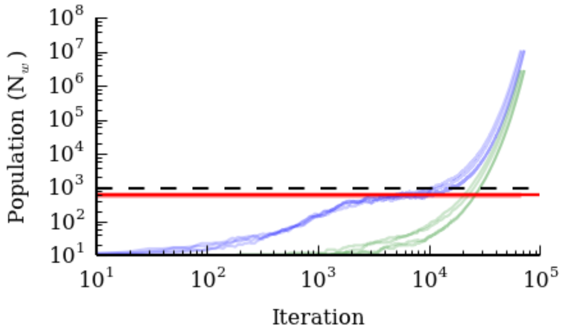


FIG. 238. $U = 2.0$, $N_{\mathrm{dets}} = 2.4\mathrm{e}{+}03$ (22 sites, 40 electrons), $N_{\mathrm{plat}} = 594 \pm 10$ %

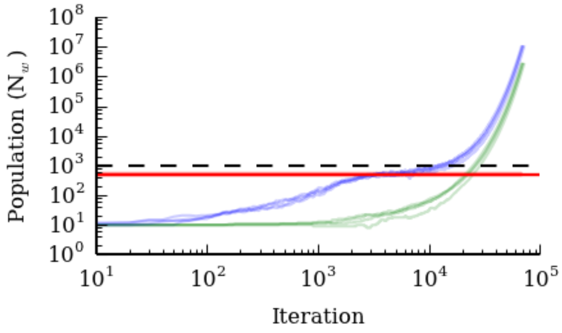


FIG. 239. $U = 2.0$, $N_{\mathrm{dets}} = 2.4\mathrm{e}{+}03$ (22 sites, 4 electrons), $N_{\mathrm{plat}} = 519 \pm 8.8$ %

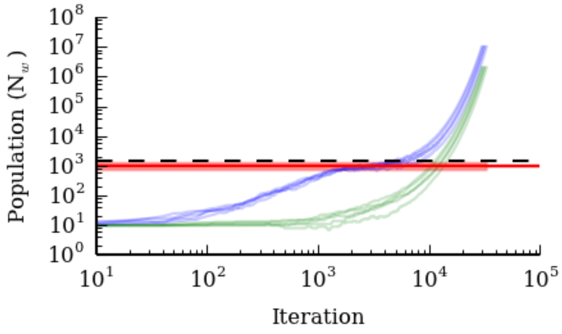


FIG. 240. $U = 2.0$, $N_{\mathrm{dets}} = 4\mathrm{e}{+}03$ (12 sites, 6 electrons), $N_{\mathrm{plat}} = 981 \pm 27$ %

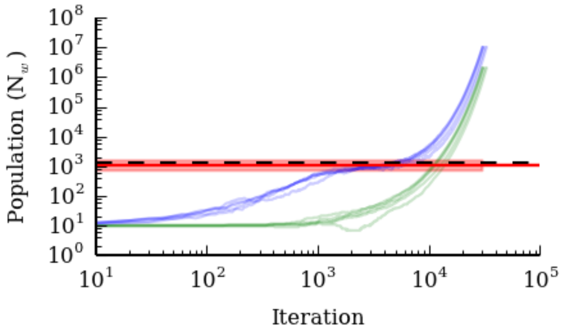


FIG. 241. $U = 2.0$, $N_{\rm dets} = $ 4e+03 (12 sites, 18 electrons), $N_{\rm plat} = $ 1.15e+03 ± 37 % (manual correction: 1e+03)

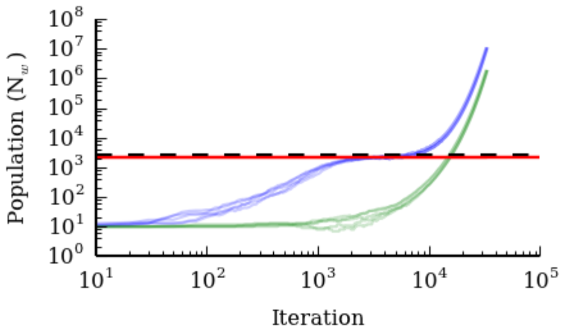


FIG. 242. $U = 2.0$, $N_{\rm dets} = $ 9.5e+03 (14 sites, 6 electrons), $N_{\rm plat} = $ 2.16e+03 ± 0.35 %

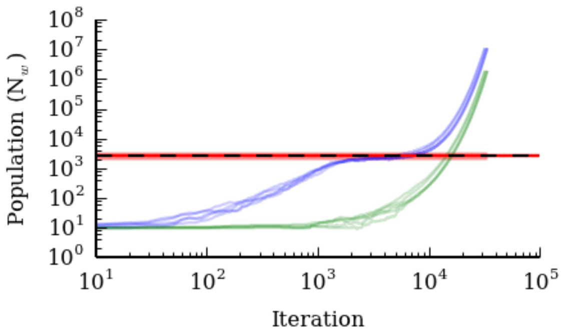


FIG. 243. $U = 2.0$, $N_{\rm dets} = $ 9.5e+03 (14 sites, 22 electrons), $N_{\rm plat} = $ 2.6e+03 ± 21 %

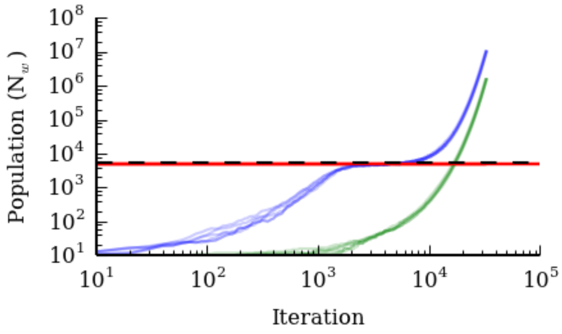


FIG. 244. $U = 2.0$, $N_{\rm dets} = $ 2e+04 (16 sites, 26 electrons), $N_{\rm plat} = $ 4.9e+03 ± 5.6 %

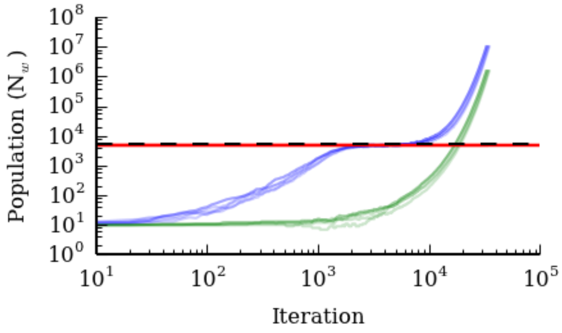


FIG. 245. $U = 2.0$, $N_{\rm dets} = $ 2e+04 (16 sites, 6 electrons), $N_{\rm plat} = $ 4.87e+03 ± 2.7 %

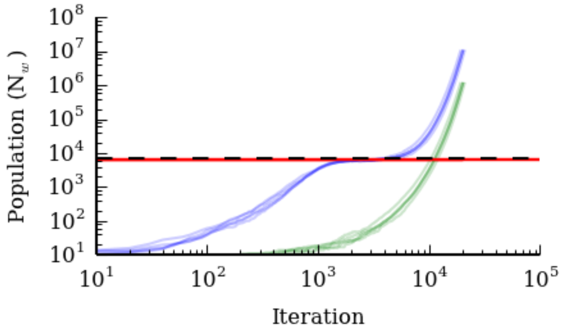


FIG. 246. $U = 2.0$, $N_{\rm dets} = $ 2e+04 (12 sites, 8 electrons), $N_{\rm plat} = $ 6.23e+03 ± 0.91 %

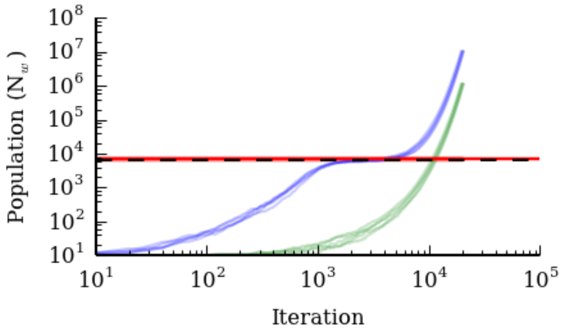


FIG. 247. $U$ = 2.0, $N_{\rm dets}$ = 2e+04 (12 sites, 16 electrons), $N_{\rm plat}$ = 6.93e+03 ± 11 %

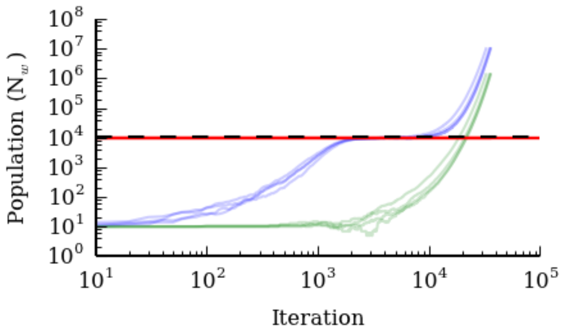


FIG. 248. $U$ = 2.0, $N_{\rm dets}$ = 3.7e+04 (18 sites, 30 electrons), $N_{\rm plat}$ = 9.85e+03 ± 3.8 %

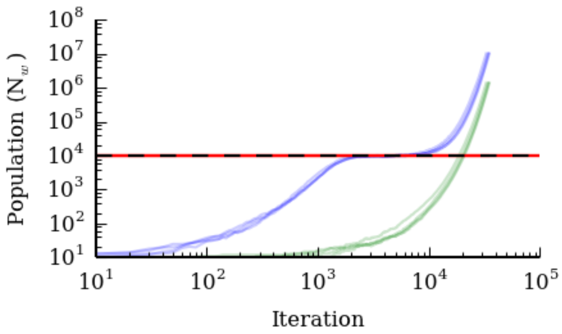


FIG. 249. $U$ = 2.0, $N_{\rm dets}$ = 3.7e+04 (18 sites, 6 electrons), $N_{\rm plat}$ = 9.94e+03 ± 1.6 %

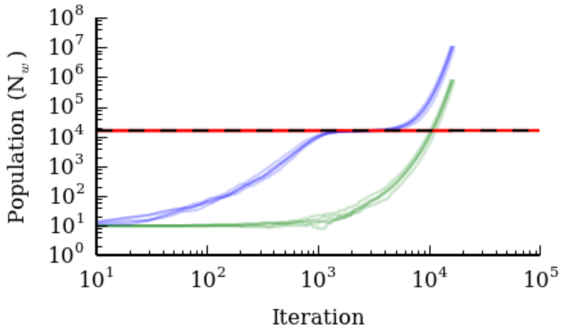


FIG. 250. $U$ = 2.0, $N_{\rm dets}$ = 5.2e+04 (12 sites, 10 electrons), $N_{\rm plat}$ = 1.55e+04 ± 1.5 %

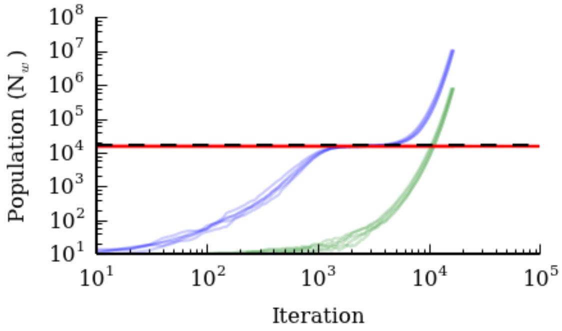


FIG. 251. $U$ = 2.0, $N_{\rm dets}$ = 5.2e+04 (12 sites, 14 electrons), $N_{\rm plat}$ = 1.55e+04 ± 4.7 %

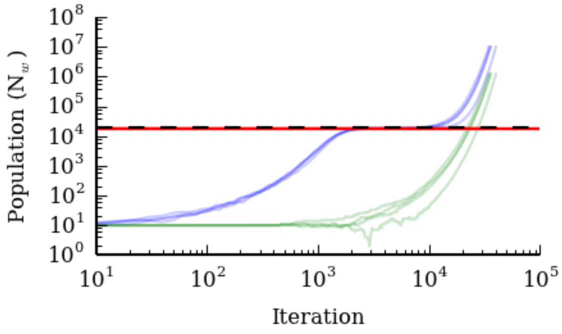


FIG. 252. $U$ = 2.0, $N_{\rm dets}$ = 6.5e+04 (20 sites, 34 electrons), $N_{\rm plat}$ = 1.82e+04 ± 0.26 %

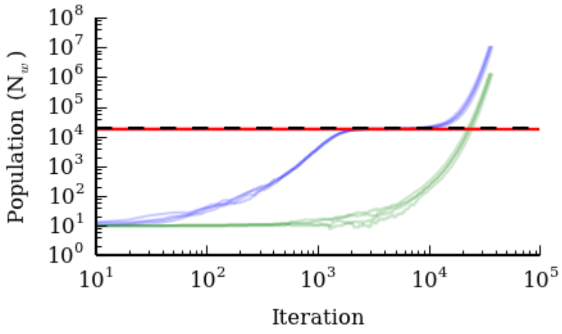


FIG. 253. $U$ = 2.0, $N_{\rm dets}$ = 6.5e+04 (20 sites, 6 electrons), $N_{\rm plat}$ = 1.81e+04 ± 0.077 %

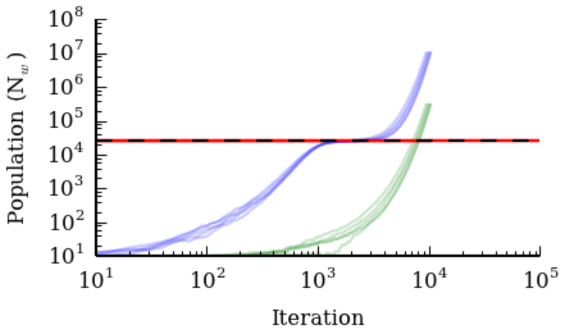


FIG. 254. $U$ = 2.0, $N_{\rm dets}$ = 7.1e+04 (12 sites, 12 electrons), $N_{\rm plat}$ = 2.51e+04 ± 1.3 %

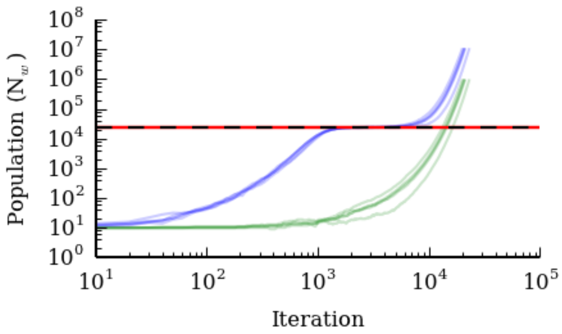


FIG. 255. $U$ = 2.0, $N_{\rm dets}$ = 7.2e+04 (14 sites, 8 electrons), $N_{\rm plat}$ = 2.39e+04 ± 0.48 %

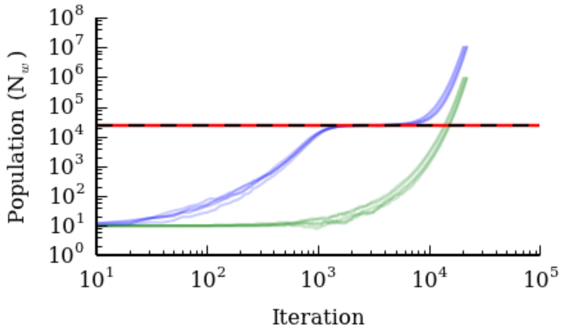


FIG. 256. $U$ = 2.0, $N_{\rm dets}$ = 7.2e+04 (14 sites, 20 electrons), $N_{\rm plat}$ = 2.37e+04 ± 0.087 %

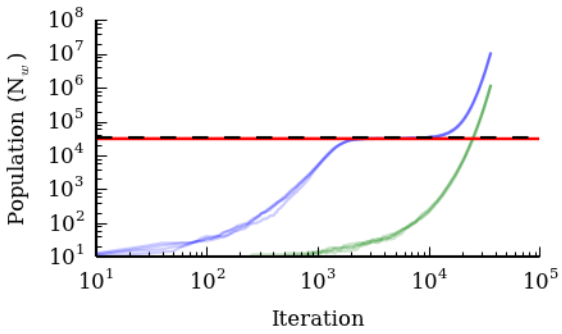


FIG. 257. $U$ = 2.0, $N_{\rm dets}$ = 1.1e+05 (22 sites, 38 electrons), $N_{\rm plat}$ = 3.16e+04 ± 1.3 %

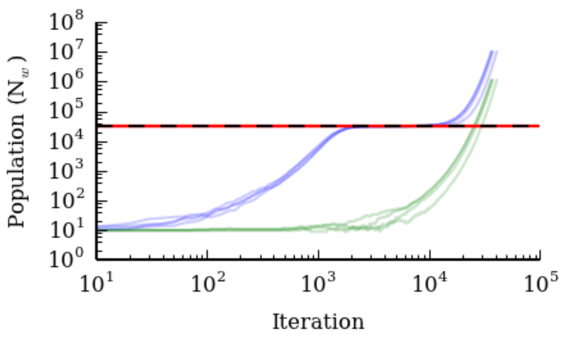


FIG. 258. $U$ = 2.0, $N_{\rm dets}$ = 1.1e+05 (22 sites, 6 electrons), $N_{\rm plat}$ = 3.18e+04 ± 0.41 %

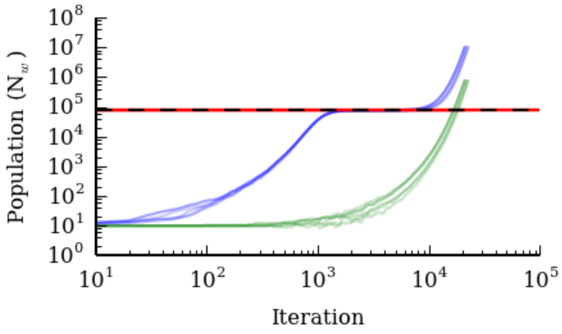


FIG. 259. $U$ = 2.0, $N_{\rm dets}$ = 2.1e+05 (16 sites, 8 electrons), $N_{\rm plat}$ = 7.6e+04 ± 0.093 %

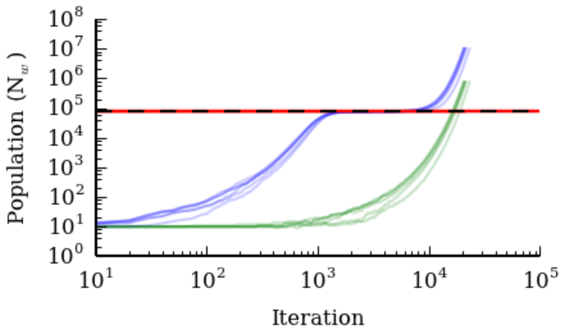


FIG. 260. $U$ = 2.0, $N_{\rm dets}$ = 2.1e+05 (16 sites, 24 electrons), $N_{\rm plat}$ = 7.61e+04 ± 0.38 %

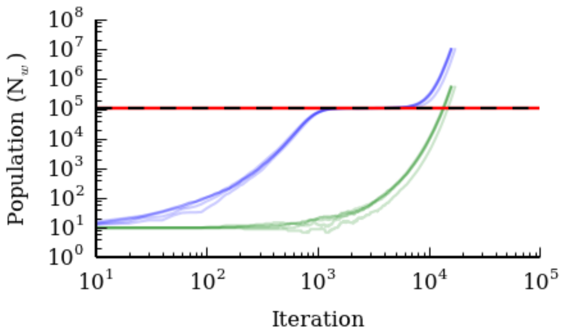


FIG. 261. $U$ = 2.0, $N_{\rm dets}$ = 2.9e+05 (14 sites, 18 electrons), $N_{\rm plat}$ = 1.06e+05 ± 0.18 %

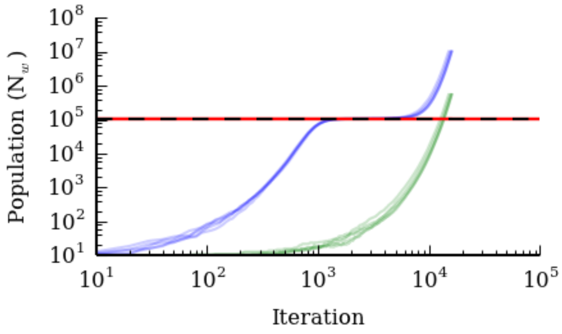


FIG. 262. $U$ = 2.0, $N_{\rm dets}$ = 2.9e+05 (14 sites, 10 electrons), $N_{\rm plat}$ = 1.06e+05 ± 0.12 %

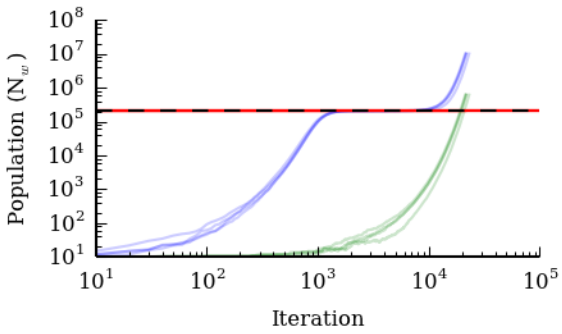


FIG. 263. $U$ = 2.0, $N_{\rm dets}$ = 5.2e+05 (18 sites, 8 electrons), $N_{\rm plat}$ = 2.06e+05 ± 0.059 %

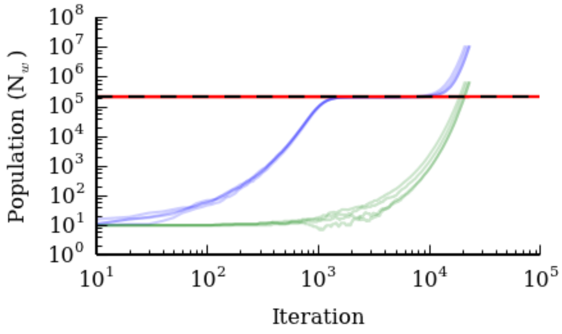


FIG. 264. $U$ = 2.0, $N_{\rm dets}$ = 5.2e+05 (18 sites, 28 electrons), $N_{\rm plat}$ = 2.06e+05 ± 0.35 %

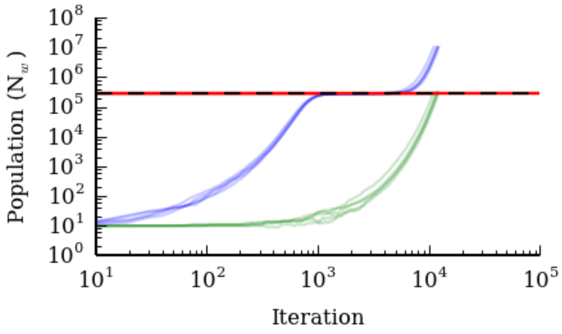


FIG. 265. $U$ = 2.0, $N_{\rm dets}$ = 6.4e+05 (14 sites, 16 electrons), $N_{\rm plat}$ = 2.77e+05 ± 0.81 %

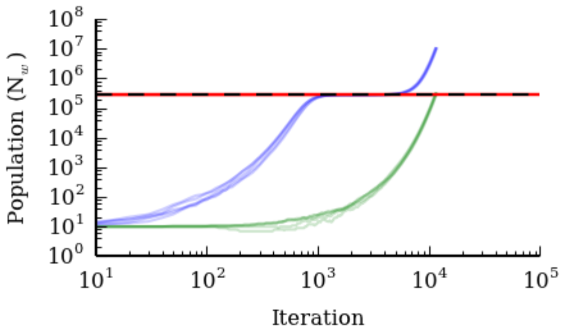


FIG. 266. $U$ = 2.0, $N_{\rm dets}$ = 6.4e+05 (14 sites, 12 electrons), $N_{\rm plat}$ = 2.79e+05 ± 0.51 %

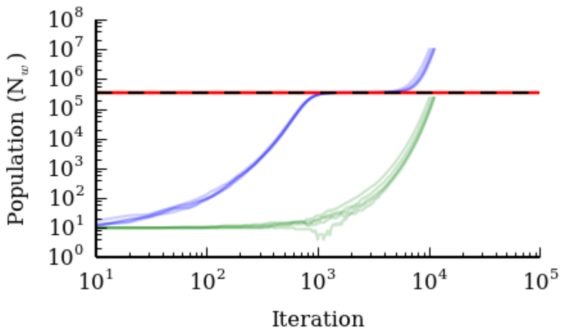


FIG. 267. $U$ = 2.0, $N_{\rm dets}$ = 8.4e+05 (14 sites, 14 electrons), $N_{\rm plat}$ = 3.5e+05 ± 0.13 %

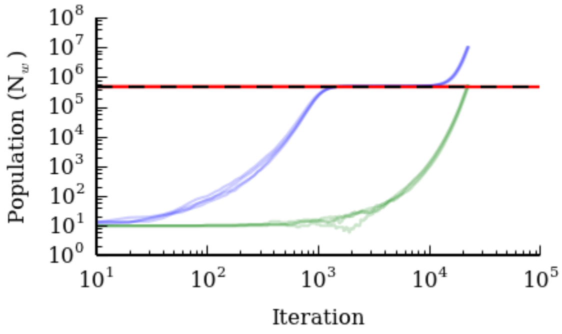


FIG. 268. $U$ = 2.0, $N_{\rm dets}$ = 1.2e+06 (20 sites, 32 electrons), $N_{\rm plat}$ = 4.94e+05 ± 0.02 %

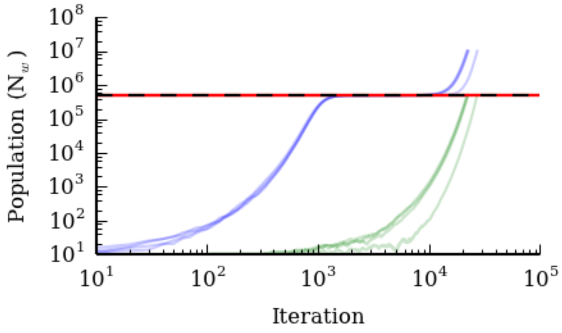


FIG. 269. $U$ = 2.0, $N_{\rm dets}$ = 1.2e+06 (20 sites, 8 electrons), $N_{\rm plat}$ = 4.94e+05 ± 0.24 %

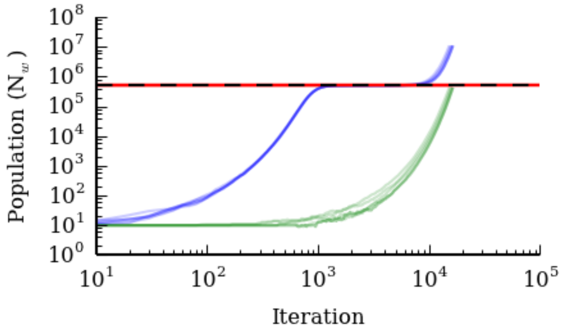


FIG. 270. $U$ = 2.0, $N_{\rm dets}$ = 1.2e+06 (16 sites, 10 electrons), $N_{\rm plat}$ = 5.08e+05 ± 0.11 %

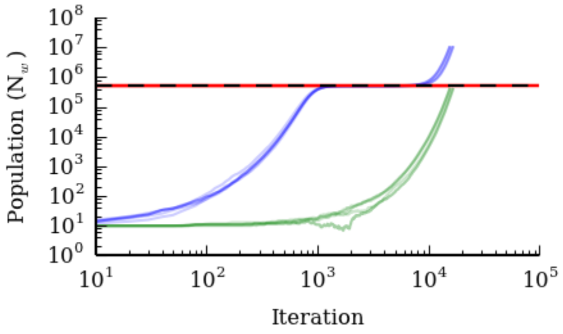


FIG. 271. $U$ = 2.0, $N_{\mathrm{dets}}$ = 1.2e+06 (16 sites, 22 electrons), $N_{\mathrm{plat}}$ = 5.06e+05 ± 0.36 %

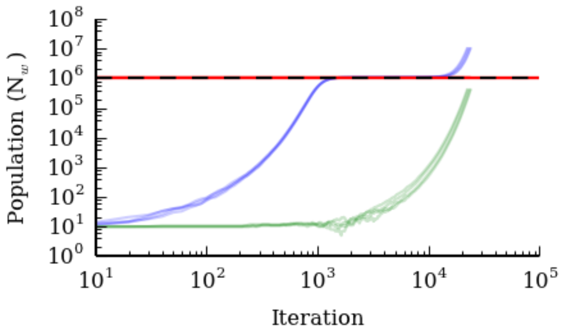


FIG. 272. $U$ = 2.0, $N_{\mathrm{dets}}$ = 2.4e+06 (22 sites, 8 electrons), $N_{\mathrm{plat}}$ = 1.07e+06 ± 0.051 %

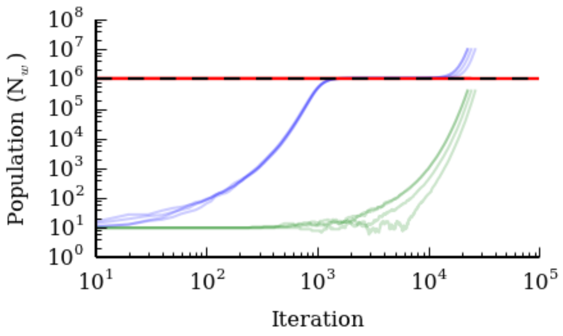


FIG. 273. $U$ = 2.0, $N_{\mathrm{dets}}$ = 2.4e+06 (22 sites, 36 electrons), $N_{\mathrm{plat}}$ = 1.07e+06 ± 0.073 %

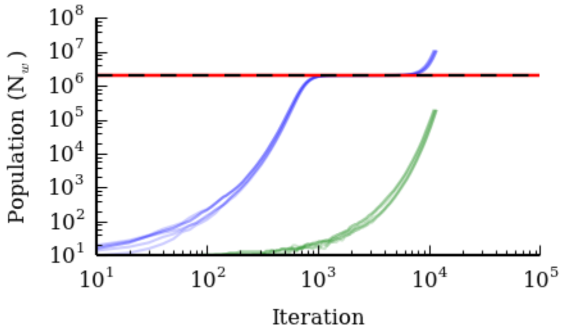


FIG. 274. $U$ = 2.0, $N_{\mathrm{dets}}$ = 4e+06 (16 sites, 12 electrons), $N_{\mathrm{plat}}$ = 2e+06 ± 0.35 %

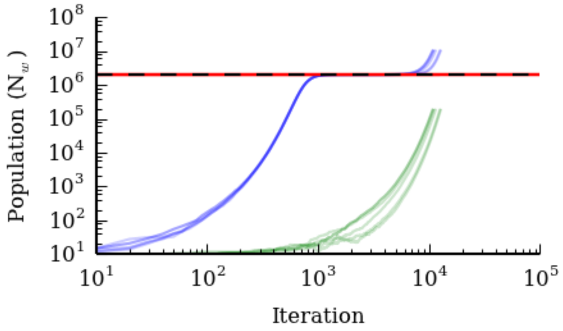


FIG. 275. $U$ = 2.0, $N_{\mathrm{dets}}$ = 4e+06 (16 sites, 20 electrons), $N_{\mathrm{plat}}$ = 2e+06 ± 0.21 %

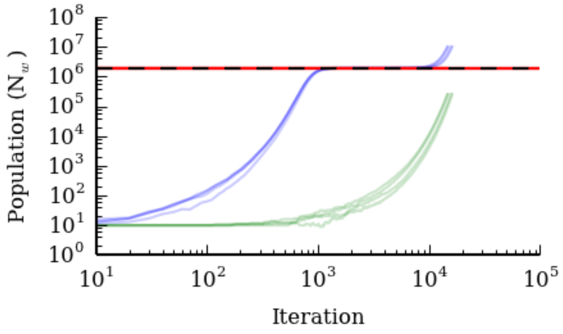


FIG. 276. $U$ = 2.0, $N_{\mathrm{dets}}$ = 4.1e+06 (18 sites, 10 electrons), $N_{\mathrm{plat}}$ = 1.93e+06 ± 0.12 %

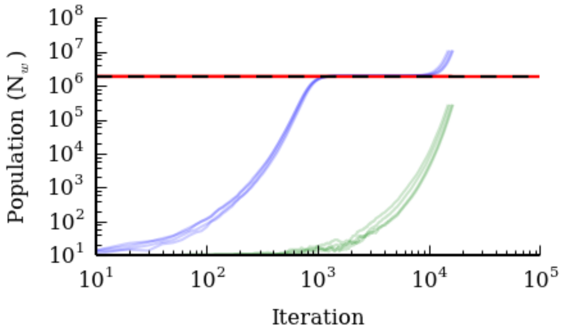


FIG. 277. $U$ = 2.0, $N_{\rm dets}$ = 4.1e+06 (18 sites, 26 electrons), $N_{\rm plat}$ = 1.92e+06 ± 0.36 %

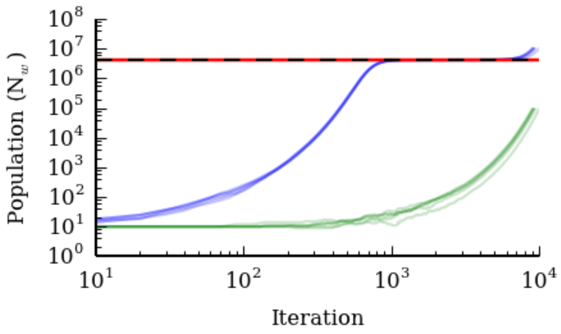


FIG. 278. $U$ = 2.0, $N_{\rm dets}$ = 8.2e+06 (16 sites, 18 electrons), $N_{\rm plat}$ = 4.16e+06 ± 1.7 %

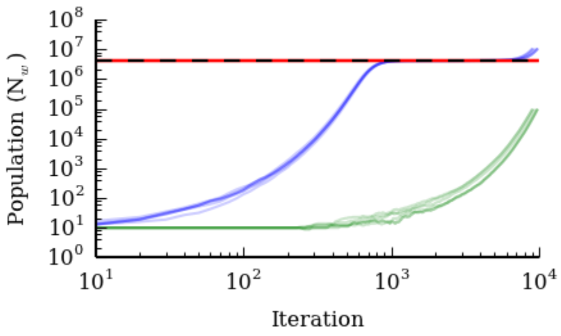


FIG. 279. $U$ = 2.0, $N_{\rm dets}$ = 8.2e+06 (16 sites, 14 electrons), $N_{\rm plat}$ = 4.17e+06 ± 0.6 %

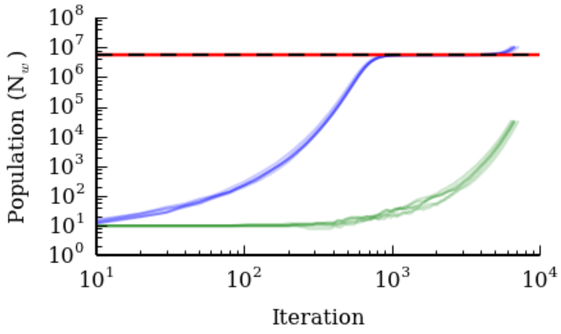


FIG. 280. $U$ = 2.0, $N_{\rm dets}$ = 1e+07 (16 sites, 16 electrons), $N_{\rm plat}$ = 5.57e+06 ± 0.33 %

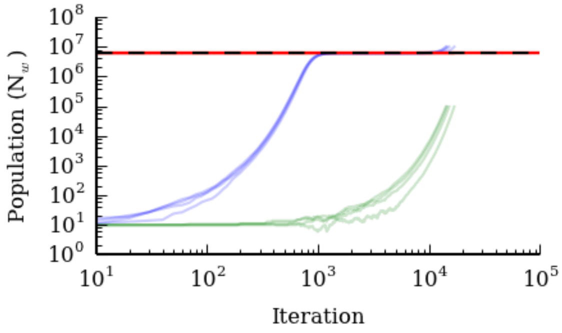


FIG. 281. $U$ = 2.0, $N_{\rm dets}$ = 1.2e+07 (20 sites, 30 electrons), $N_{\rm plat}$ = 6.12e+06 ± 0.29 %

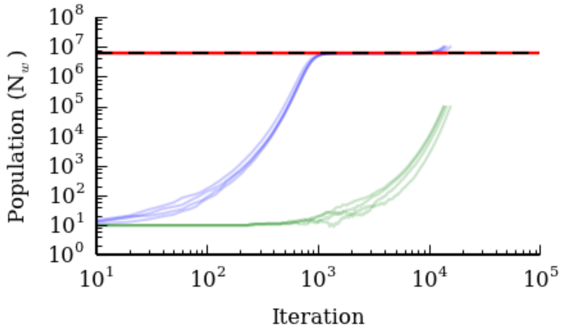


FIG. 282. $U$ = 2.0, $N_{\rm dets}$ = 1.2e+07 (20 sites, 10 electrons), $N_{\rm plat}$ = 6.12e+06 ± 0.18 %

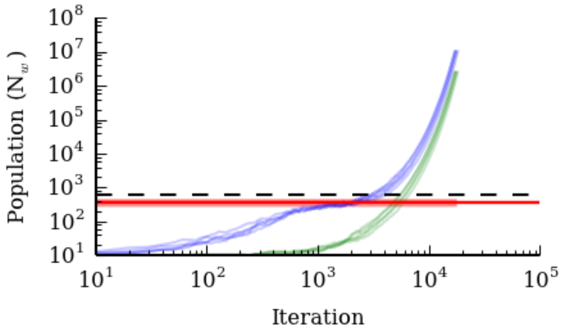


FIG. 283. $U$ = 4.0, $N_{\mathrm{dets}}$ = 3.7e+02 (12 sites, 4 electrons), $N_{\mathrm{plat}}$ = 361 ± 19 %

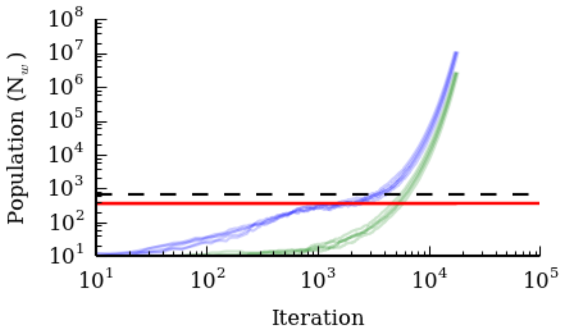


FIG. 284. $U$ = 4.0, $N_{\mathrm{dets}}$ = 3.7e+02 (12 sites, 20 electrons), $N_{\mathrm{plat}}$ = 355 ± 0 %

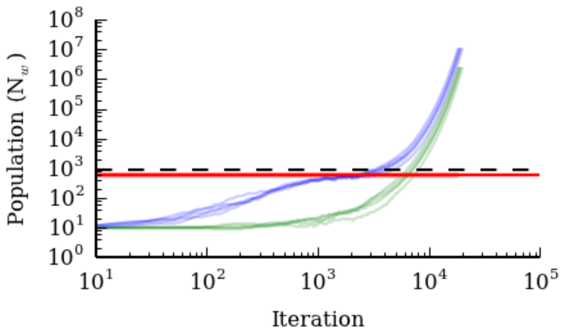


FIG. 285. $U$ = 4.0, $N_{\mathrm{dets}}$ = 6e+02 (14 sites, 4 electrons), $N_{\mathrm{plat}}$ = 596 ± 12 %

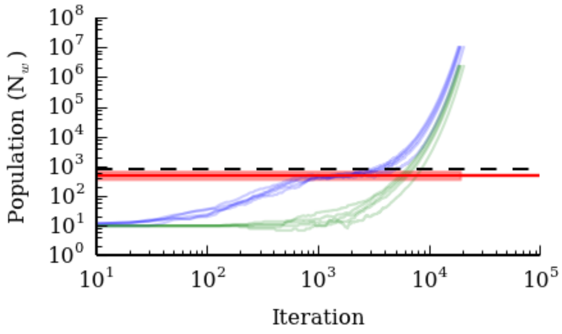


FIG. 286. $U$ = 4.0, $N_{\mathrm{dets}}$ = 6e+02 (14 sites, 24 electrons), $N_{\mathrm{plat}}$ = 506 ± 31 % (manual correction: 500)

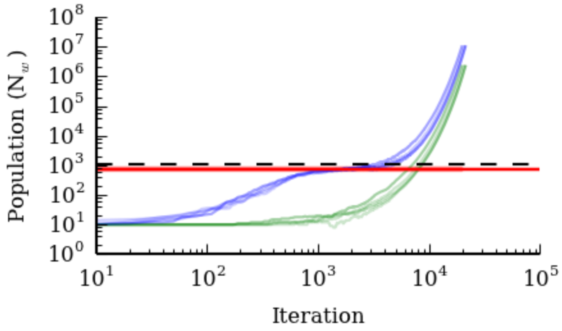


FIG. 287. $U$ = 4.0, $N_{\mathrm{dets}}$ = 9e+02 (16 sites, 28 electrons), $N_{\mathrm{plat}}$ = 755 ± 13 %

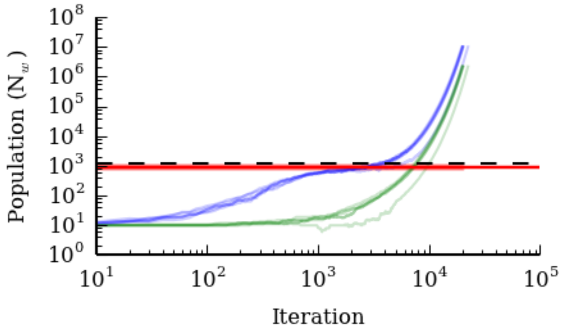


FIG. 288. $U$ = 4.0, $N_{\mathrm{dets}}$ = 9e+02 (16 sites, 4 electrons), $N_{\mathrm{plat}}$ = 905 ± 17 %

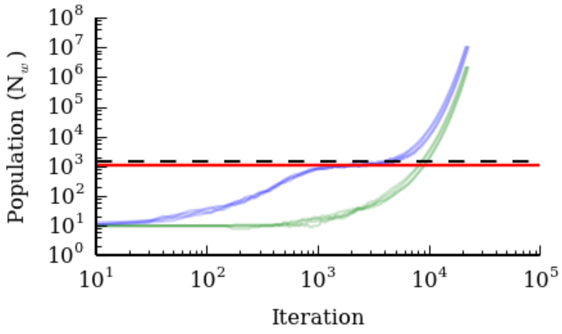


FIG. 289. $U$ = 4.0, $N_{\text{dets}}$ = 1.3e+03 (18 sites, 32 electrons), $N_{\text{plat}}$ = 1.09e+03 ± 1.3 %

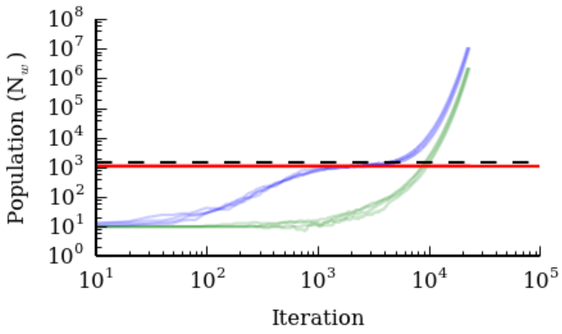


FIG. 290. $U$ = 4.0, $N_{\text{dets}}$ = 1.3e+03 (18 sites, 4 electrons), $N_{\text{plat}}$ = 1.14e+03 ± 4.9 %

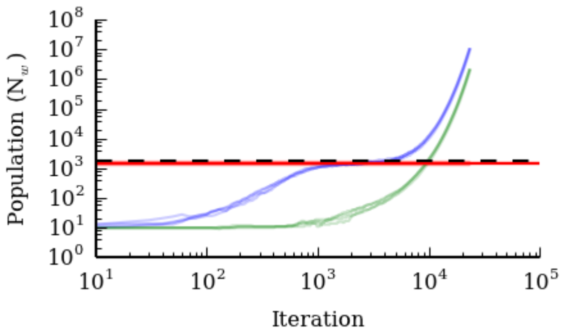


FIG. 291. $U$ = 4.0, $N_{\text{dets}}$ = 1.8e+03 (20 sites, 4 electrons), $N_{\text{plat}}$ = 1.48e+03 ± 12 %

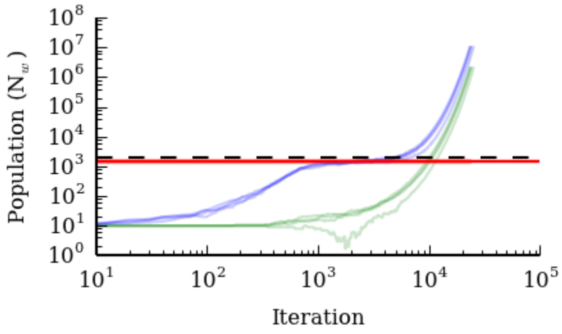


FIG. 292. $U$ = 4.0, $N_{\text{dets}}$ = 1.8e+03 (20 sites, 36 electrons), $N_{\text{plat}}$ = 1.46e+03 ± 10 %

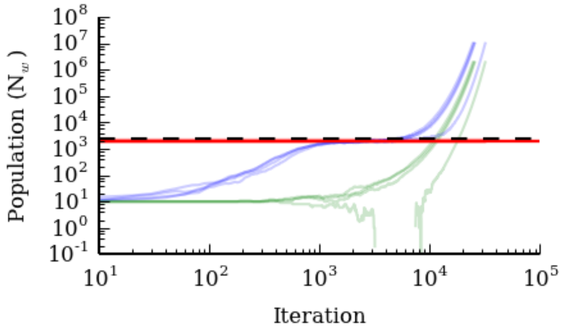


FIG. 293. $U$ = 4.0, $N_{\text{dets}}$ = 2.4e+03 (22 sites, 40 electrons), $N_{\text{plat}}$ = 2.03e+03 ± 11 %

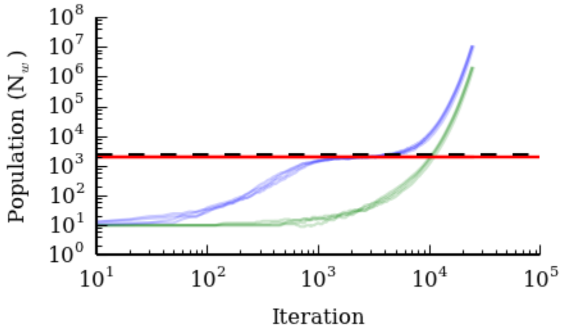


FIG. 294. $U$ = 4.0, $N_{\text{dets}}$ = 2.4e+03 (22 sites, 4 electrons), $N_{\text{plat}}$ = 1.99e+03 ± 3.7 %

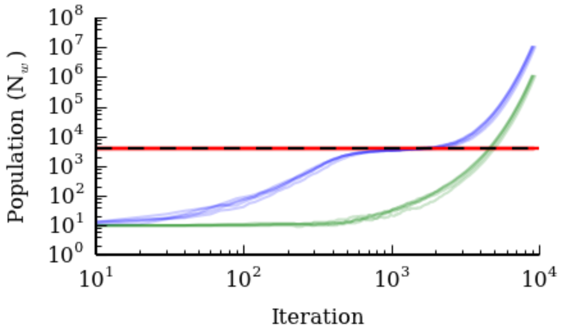


FIG. 295. $U = 4.0$, $N_{\rm dets} = 4e+03$ (12 sites, 6 electrons), $N_{\rm plat} = 3.86e+03 \pm 8.8$ %

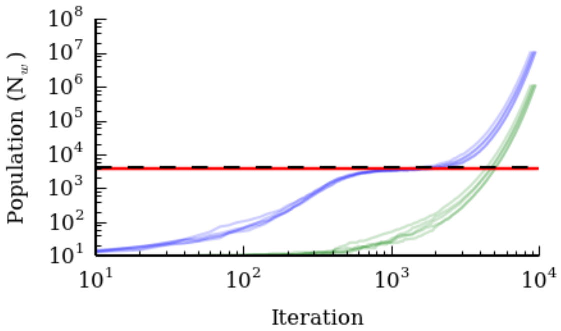


FIG. 296. $U = 4.0$, $N_{\rm dets} = 4e+03$ (12 sites, 18 electrons), $N_{\rm plat} = 3.8e+03 \pm 0.81$ %

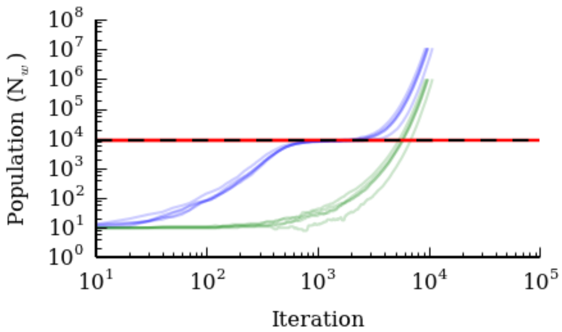


FIG. 297. $U = 4.0$, $N_{\rm dets} = 9.5e+03$ (14 sites, 6 electrons), $N_{\rm plat} = 8.68e+03 \pm 5.3$ %

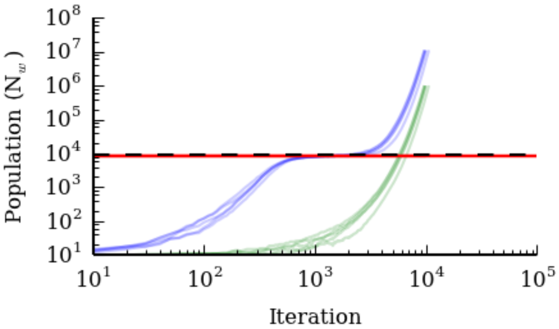


FIG. 298. $U = 4.0$, $N_{\rm dets} = 9.5e+03$ (14 sites, 22 electrons), $N_{\rm plat} = 8.43e+03 \pm 2.7$ %

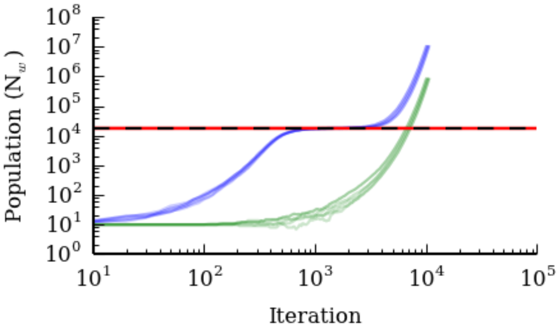


FIG. 299. $U = 4.0$, $N_{\rm dets} = 2e+04$ (16 sites, 26 electrons), $N_{\rm plat} = 1.8e+04 \pm 1.1$ %

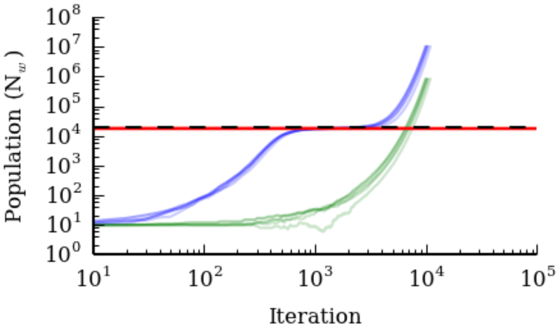


FIG. 300. $U = 4.0$, $N_{\rm dets} = 2e+04$ (16 sites, 6 electrons), $N_{\rm plat} = 1.81e+04 \pm 1.7$ %

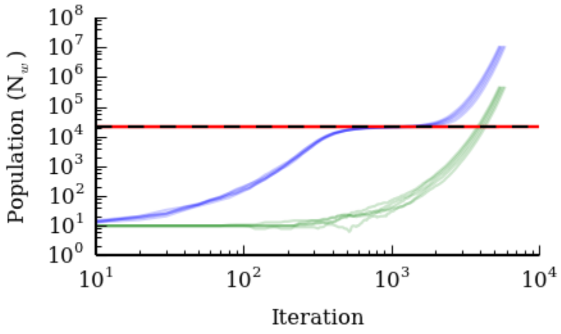


FIG. 301. $U = 4.0$, $N_{\rm dets} = 2e{+}04$ (12 sites, 8 electrons), $N_{\rm plat} = 2.13e{+}04 \pm 1.1$ %

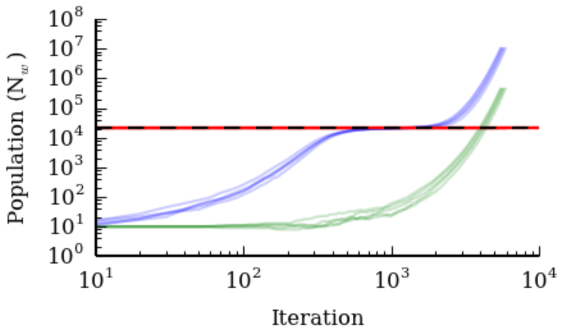


FIG. 302. $U = 4.0$, $N_{\rm dets} = 2e{+}04$ (12 sites, 16 electrons), $N_{\rm plat} = 2.1e{+}04 \pm 2.3$ %

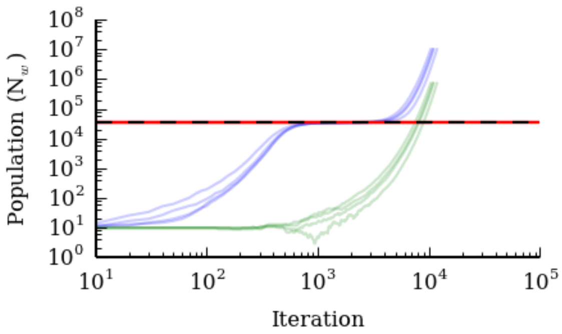


FIG. 303. $U = 4.0$, $N_{\rm dets} = 3.7e{+}04$ (18 sites, 30 electrons), $N_{\rm plat} = 3.48e{+}04 \pm 2.5$ %

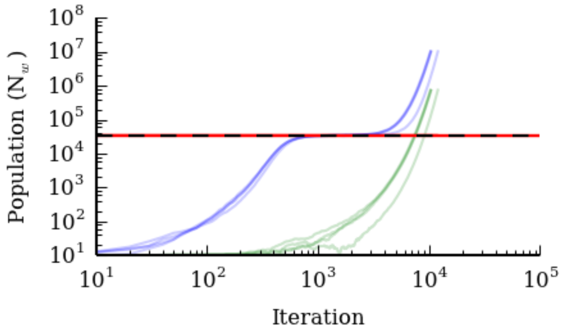


FIG. 304. $U = 4.0$, $N_{\rm dets} = 3.7e{+}04$ (18 sites, 6 electrons), $N_{\rm plat} = 3.47e{+}04 \pm 0.22$ %

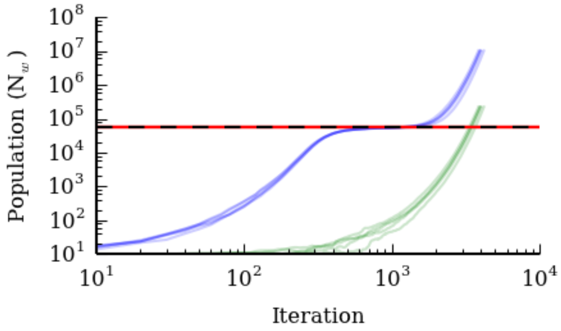


FIG. 305. $U = 4.0$, $N_{\rm dets} = 5.2e{+}04$ (12 sites, 10 electrons), $N_{\rm plat} = 5.56e{+}04 \pm 1.4$ %

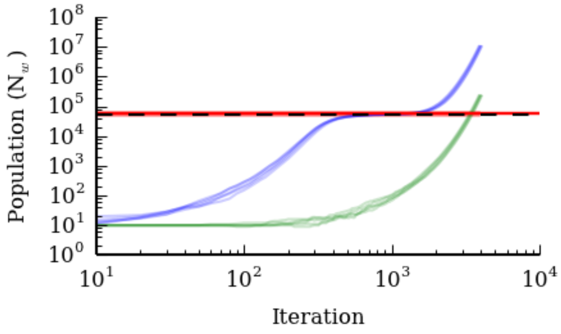


FIG. 306. $U = 4.0$, $N_{\rm dets} = 5.2e{+}04$ (12 sites, 14 electrons), $N_{\rm plat} = 5.62e{+}04 \pm 12$ %

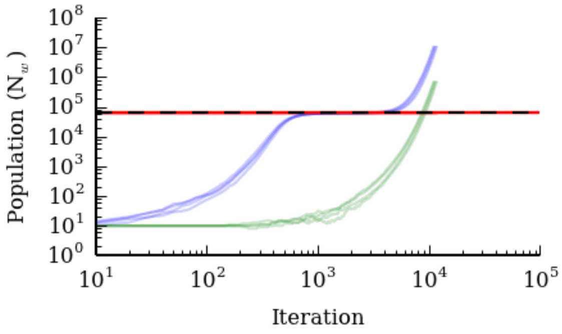


FIG. 307. $U$ = 4.0, $N_{\mathrm{dets}}$ = 6.5e+04 (20 sites, 34 electrons), $N_{\mathrm{plat}}$ = 6.18e+04 ± 0.91 %

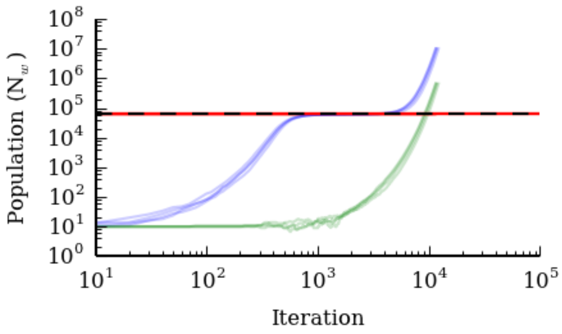


FIG. 308. $U$ = 4.0, $N_{\mathrm{dets}}$ = 6.5e+04 (20 sites, 6 electrons), $N_{\mathrm{plat}}$ = 6.16e+04 ± 0.46 %

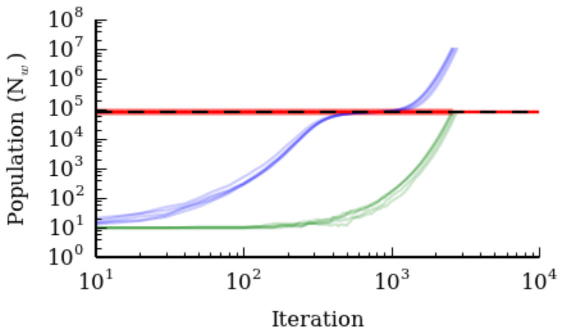


FIG. 309. $U$ = 4.0, $N_{\mathrm{dets}}$ = 7.1e+04 (12 sites, 12 electrons), $N_{\mathrm{plat}}$ = 8.06e+04 ± 22 %

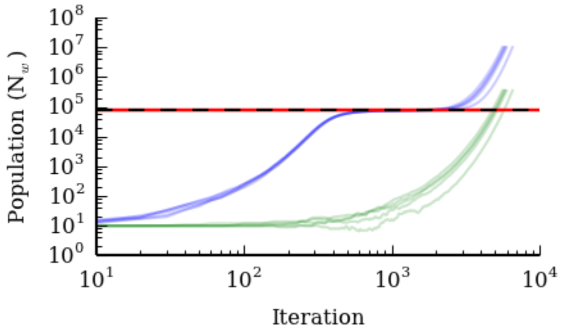


FIG. 310. $U$ = 4.0, $N_{\mathrm{dets}}$ = 7.2e+04 (14 sites, 8 electrons), $N_{\mathrm{plat}}$ = 7.78e+04 ± 2.6 %

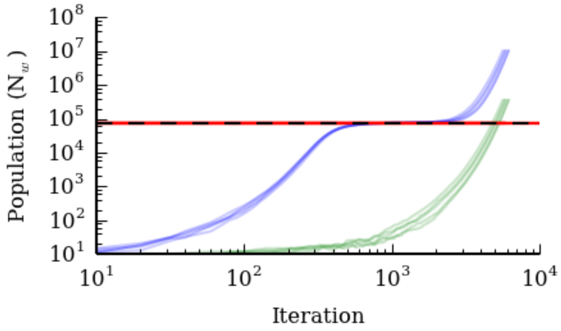


FIG. 311. $U$ = 4.0, $N_{\mathrm{dets}}$ = 7.2e+04 (14 sites, 20 electrons), $N_{\mathrm{plat}}$ = 7.59e+04 ± 4.8 %

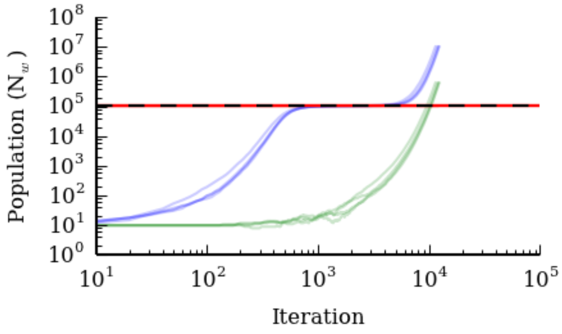


FIG. 312. $U$ = 4.0, $N_{\mathrm{dets}}$ = 1.1e+05 (22 sites, 38 electrons), $N_{\mathrm{plat}}$ = 1.04e+05 ± 0.65 %

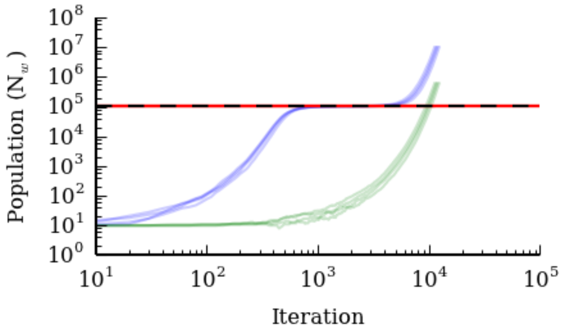


FIG. 313. $U$ = 4.0, $N_{\mathrm{dets}}$ = 1.1e+05 (22 sites, 6 electrons), $N_{\mathrm{plat}}$ = 1.05e+05 ± 1 %

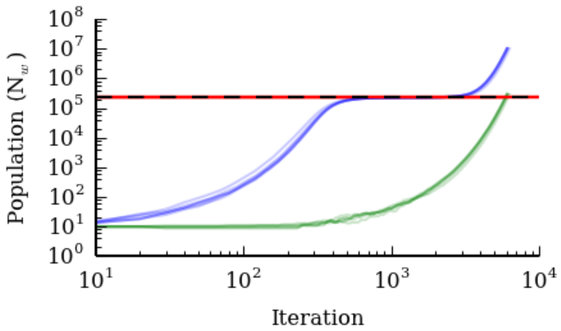


FIG. 314. $U$ = 4.0, $N_{\mathrm{dets}}$ = 2.1e+05 (16 sites, 8 electrons), $N_{\mathrm{plat}}$ = 2.28e+05 ± 1.2 %

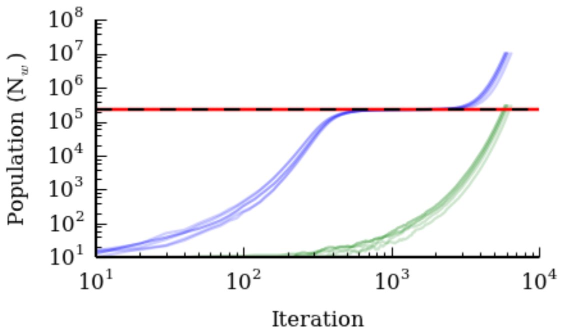


FIG. 315. $U$ = 4.0, $N_{\mathrm{dets}}$ = 2.1e+05 (16 sites, 24 electrons), $N_{\mathrm{plat}}$ = 2.27e+05 ± 0.29 %

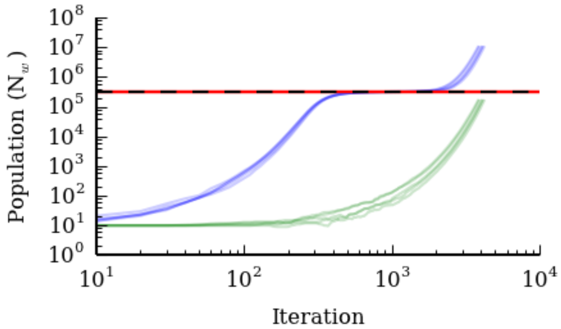


FIG. 316. $U$ = 4.0, $N_{\mathrm{dets}}$ = 2.9e+05 (14 sites, 18 electrons), $N_{\mathrm{plat}}$ = 3.17e+05 ± 2.9 %

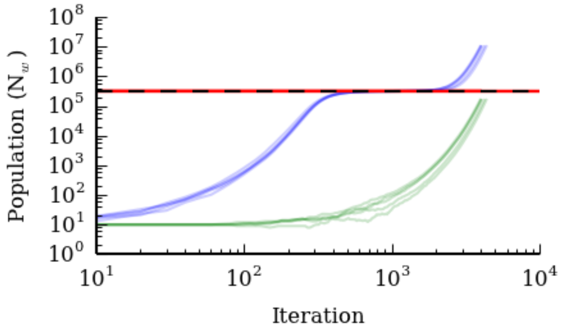


FIG. 317. $U$ = 4.0, $N_{\mathrm{dets}}$ = 2.9e+05 (14 sites, 10 electrons), $N_{\mathrm{plat}}$ = 3.33e+05 ± 0.23 %

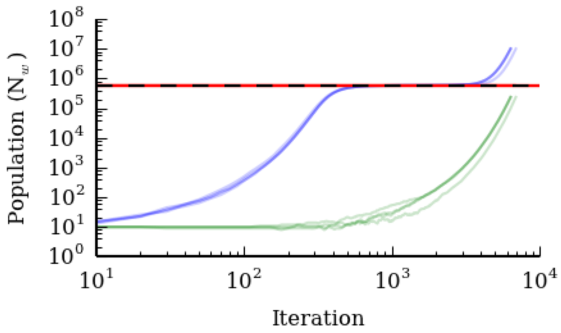


FIG. 318. $U$ = 4.0, $N_{\mathrm{dets}}$ = 5.2e+05 (18 sites, 8 electrons), $N_{\mathrm{plat}}$ = 5.85e+05 ± 0.046 %

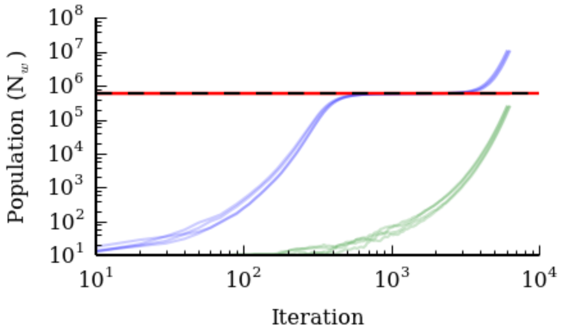


FIG. 319. $U$ = 4.0, $N_{\rm dets}$ = 5.2e+05 (18 sites, 28 electrons), $N_{\rm plat}$ = 5.8e+05 ± 1.3 %

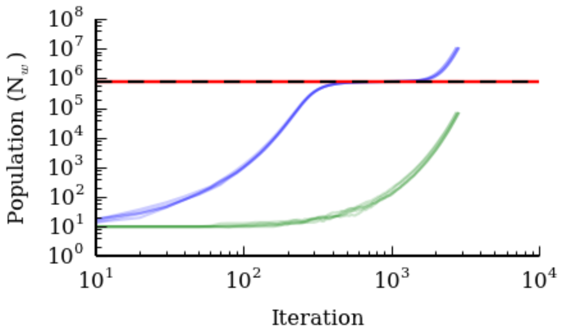


FIG. 320. $U$ = 4.0, $N_{\rm dets}$ = 6.4e+05 (14 sites, 16 electrons), $N_{\rm plat}$ = 7.88e+05 ± 2 %

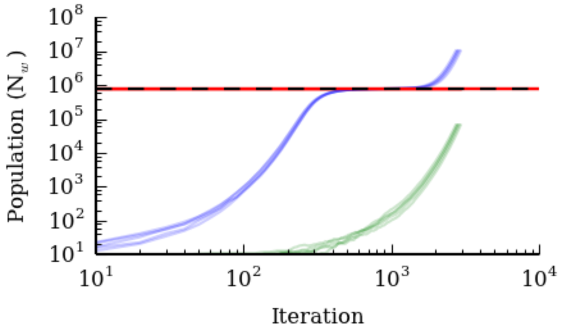


FIG. 321. $U$ = 4.0, $N_{\rm dets}$ = 6.4e+05 (14 sites, 12 electrons), $N_{\rm plat}$ = 7.42e+05 ± 2.8 %

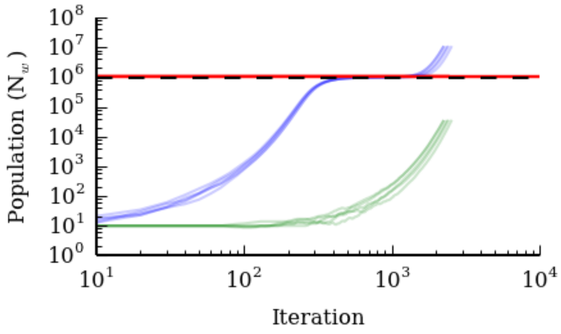


FIG. 322. $U$ = 4.0, $N_{\rm dets}$ = 8.4e+05 (14 sites, 14 electrons), $N_{\rm plat}$ = 1.09e+06 ± 5.9 %

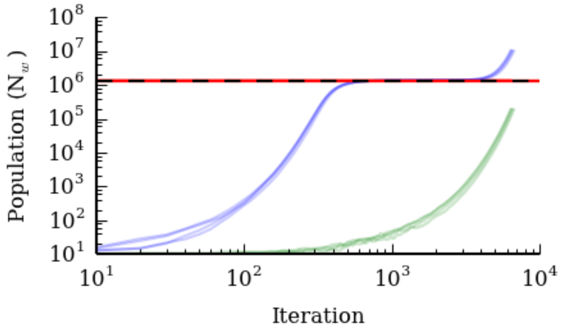


FIG. 323. $U$ = 4.0, $N_{\rm dets}$ = 1.2e+06 (20 sites, 32 electrons), $N_{\rm plat}$ = 1.36e+06 ± 1.4 %

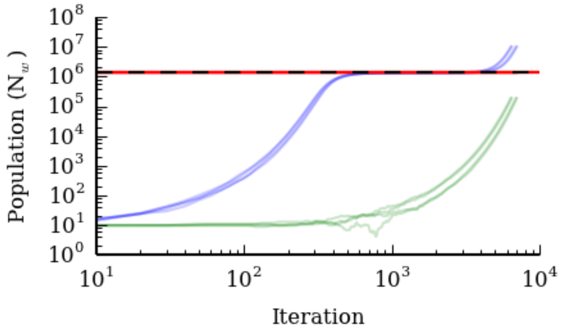


FIG. 324. $U$ = 4.0, $N_{\rm dets}$ = 1.2e+06 (20 sites, 8 electrons), $N_{\rm plat}$ = 1.36e+06 ± 3.3 %

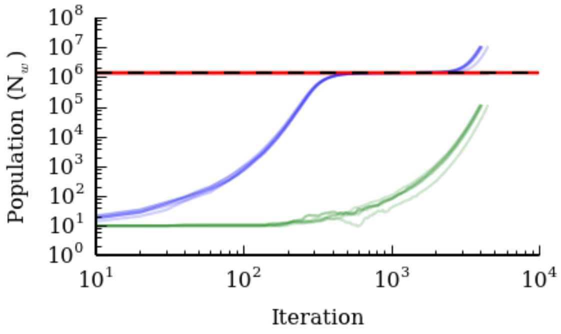


FIG. 325. $U$ = 4.0, $N_{\text{dets}}$ = 1.2e+06 (16 sites, 10 electrons), $N_{\text{plat}}$ = 1.38e+06 ± 5.8 %

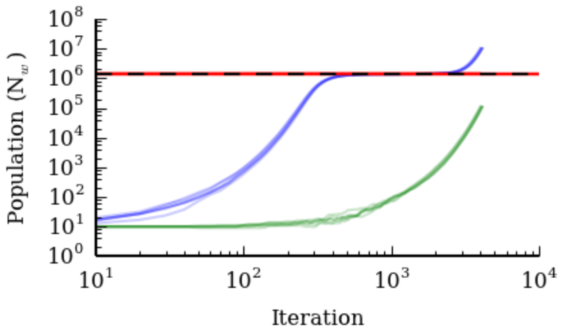


FIG. 326. $U$ = 4.0, $N_{\text{dets}}$ = 1.2e+06 (16 sites, 22 electrons), $N_{\text{plat}}$ = 1.47e+06 ± 0.85 %

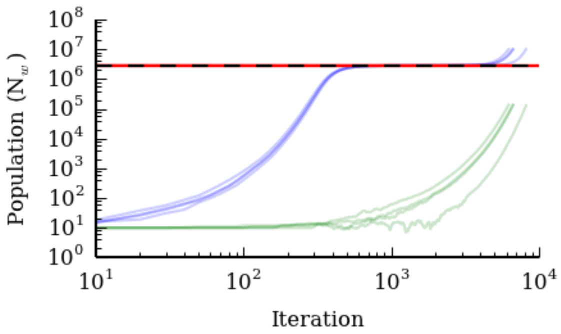


FIG. 327. $U$ = 4.0, $N_{\text{dets}}$ = 2.4e+06 (22 sites, 8 electrons), $N_{\text{plat}}$ = 2.89e+06 ± 0.95 %

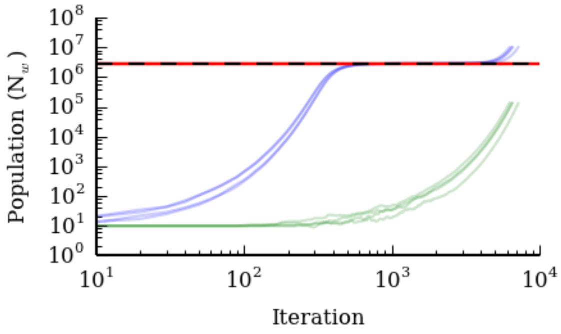


FIG. 328. $U$ = 4.0, $N_{\text{dets}}$ = 2.4e+06 (22 sites, 36 electrons), $N_{\text{plat}}$ = 2.86e+06 ± 2.4 %

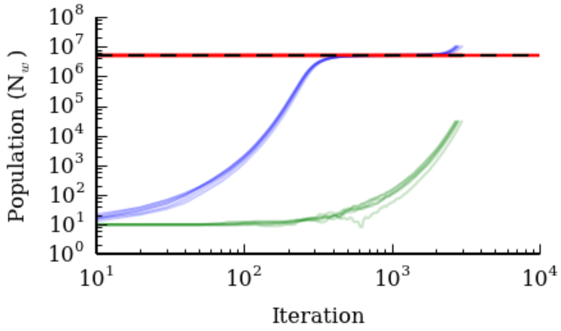


FIG. 329. $U$ = 4.0, $N_{\text{dets}}$ = 4e+06 (16 sites, 12 electrons), $N_{\text{plat}}$ = 5.15e+06 ± 6 %

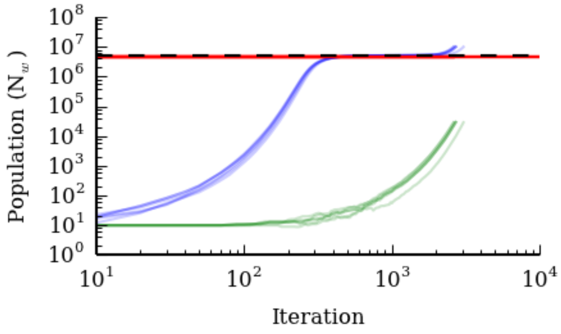


FIG. 330. $U$ = 4.0, $N_{\text{dets}}$ = 4e+06 (16 sites, 20 electrons), $N_{\text{plat}}$ = 4.67e+06 ± 7.1 %

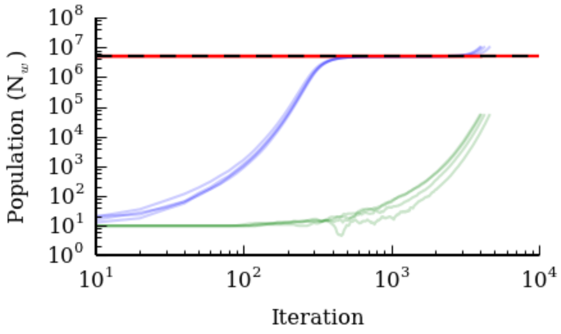


FIG. 331. $U$ = 4.0, $N_{\rm dets}$ = 4.1e+06 (18 sites, 10 electrons), $N_{\rm plat}$ = 5e+06 ± 5 %

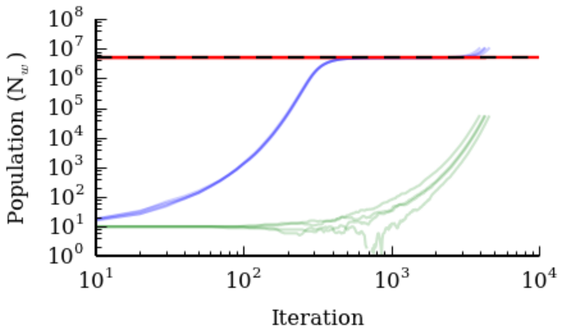


FIG. 332. $U$ = 4.0, $N_{\rm dets}$ = 4.1e+06 (18 sites, 26 electrons), $N_{\rm plat}$ = 4.88e+06 ± 0.3 %

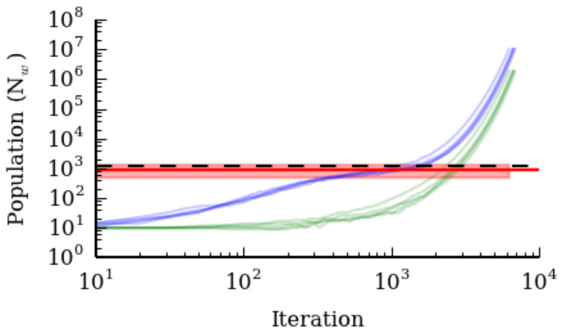


FIG. 333. $U$ = 8.0, $N_{\rm dets}$ = 3.7e+02 (12 sites, 4 electrons), $N_{\rm plat}$ = 895 ± 46 % (manual correction: 600)

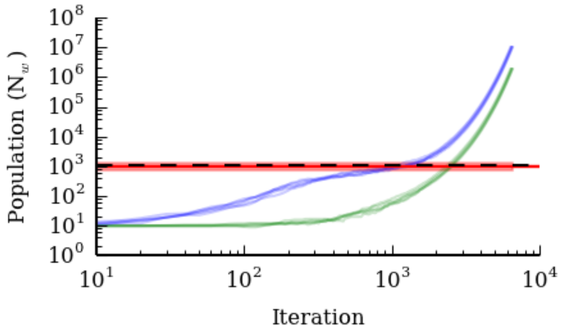


FIG. 334. $U$ = 8.0, $N_{\rm dets}$ = 3.7e+02 (12 sites, 20 electrons), $N_{\rm plat}$ = 1.01e+03 ± 28 %

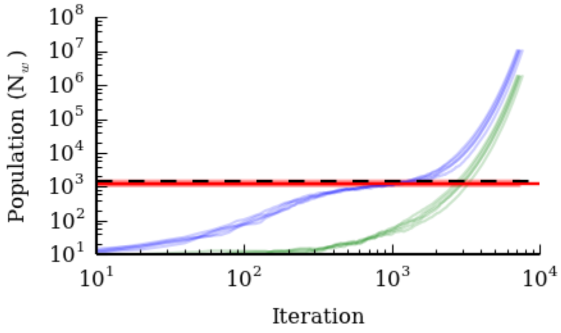


FIG. 335. $U$ = 8.0, $N_{\rm dets}$ = 6e+02 (14 sites, 4 electrons), $N_{\rm plat}$ = 1.29e+03 ± 19 %

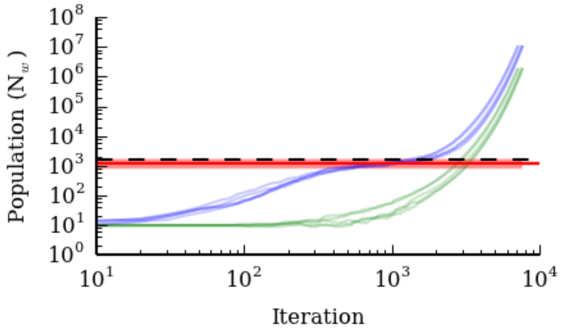


FIG. 336. $U$ = 8.0, $N_{\rm dets}$ = 6e+02 (14 sites, 24 electrons), $N_{\rm plat}$ = 1.22e+03 ± 29 %

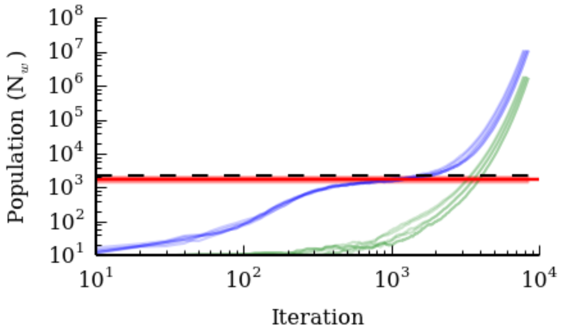


FIG. 337. $U$ = 8.0, $N_{\rm dets}$ = 9e+02 (16 sites, 28 electrons), $N_{\rm plat}$ = 1.74e+03 ± 18 %

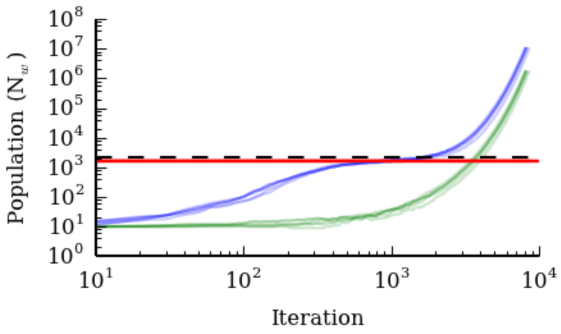


FIG. 338. $U$ = 8.0, $N_{\rm dets}$ = 9e+02 (16 sites, 4 electrons), $N_{\rm plat}$ = 1.7e+03 ± 6 %

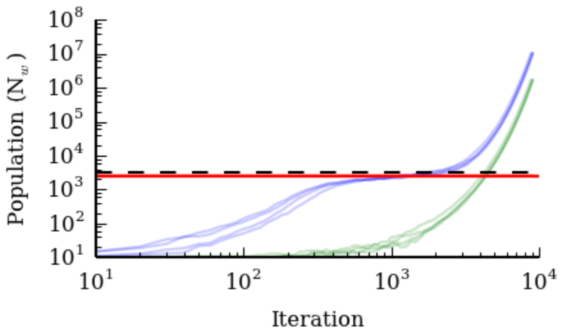


FIG. 339. $U$ = 8.0, $N_{\rm dets}$ = 1.3e+03 (18 sites, 32 electrons), $N_{\rm plat}$ = 2.58e+03 ± 3.7 %

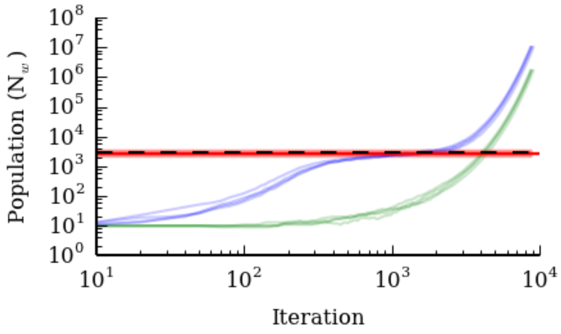


FIG. 340. $U$ = 8.0, $N_{\rm dets}$ = 1.3e+03 (18 sites, 4 electrons), $N_{\rm plat}$ = 2.77e+03 ± 23 %

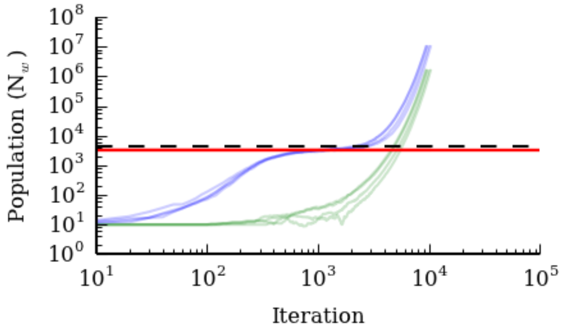


FIG. 341. $U$ = 8.0, $N_{\rm dets}$ = 1.8e+03 (20 sites, 4 electrons), $N_{\rm plat}$ = 3.33e+03 ± 2.4 %

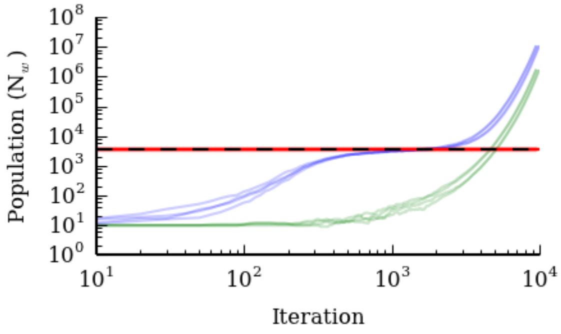


FIG. 342. $U$ = 8.0, $N_{\rm dets}$ = 1.8e+03 (20 sites, 36 electrons), $N_{\rm plat}$ = 3.56e+03 ± 10 %

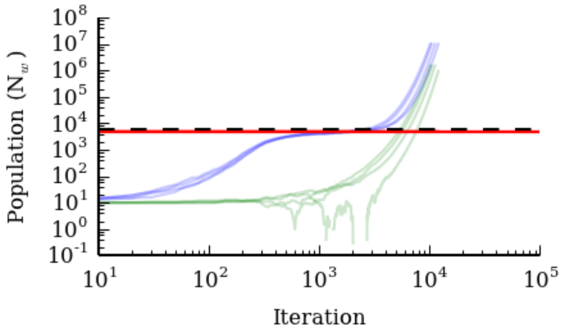


FIG. 343. $U$ = 8.0, $N_{\mathrm{dets}}$ = 2.4e+03 (22 sites, 40 electrons), $N_{\mathrm{plat}}$ = 5.05e+03 ± 4.1 %

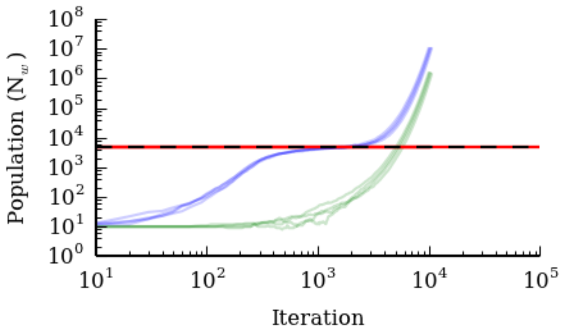


FIG. 344. $U$ = 8.0, $N_{\mathrm{dets}}$ = 2.4e+03 (22 sites, 4 electrons), $N_{\mathrm{plat}}$ = 4.8e+03 ± 6 %

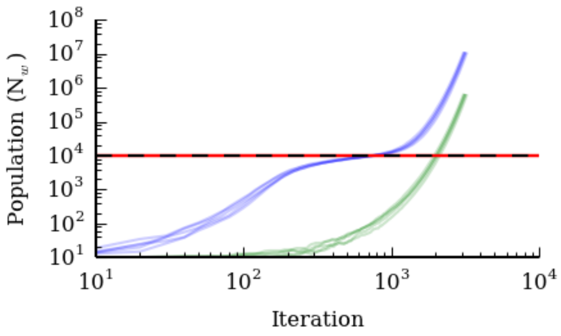


FIG. 345. $U$ = 8.0, $N_{\mathrm{dets}}$ = 4e+03 (12 sites, 6 electrons), $N_{\mathrm{plat}}$ = 9.69e+03 ± 1 %

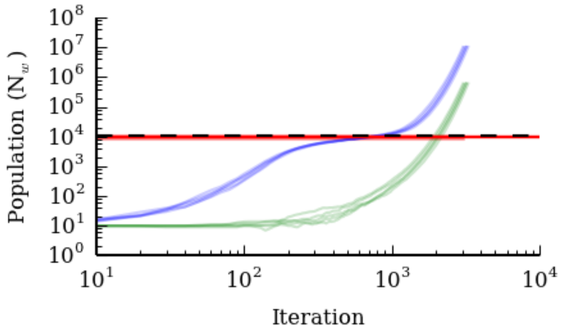


FIG. 346. $U$ = 8.0, $N_{\mathrm{dets}}$ = 4e+03 (12 sites, 18 electrons), $N_{\mathrm{plat}}$ = 9.67e+03 ± 14 %

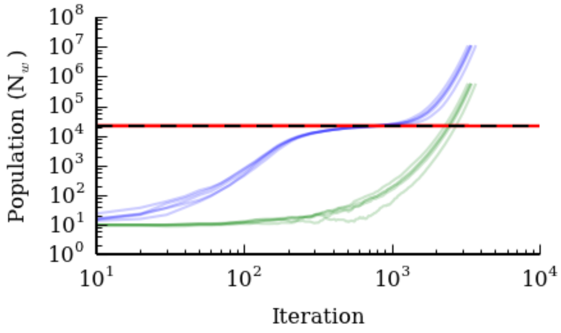


FIG. 347. $U$ = 8.0, $N_{\mathrm{dets}}$ = 9.5e+03 (14 sites, 6 electrons), $N_{\mathrm{plat}}$ = 2.24e+04 ± 6.4 %

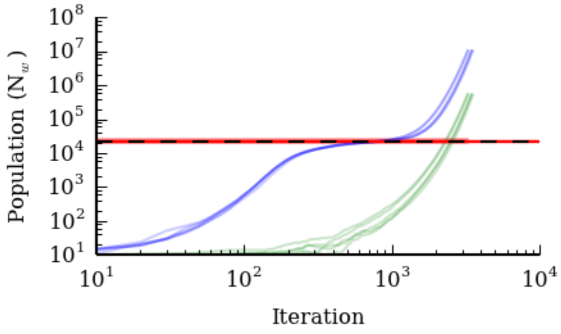


FIG. 348. $U$ = 8.0, $N_{\mathrm{dets}}$ = 9.5e+03 (14 sites, 22 electrons), $N_{\mathrm{plat}}$ = 2.26e+04 ± 15 %

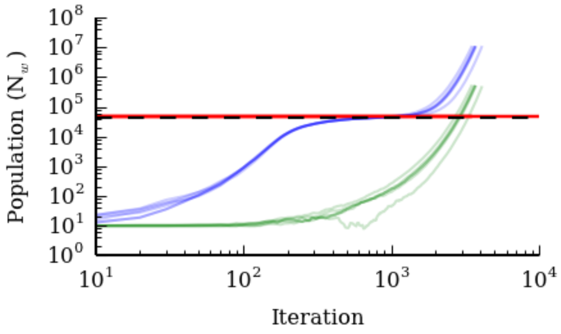


FIG. 349. $U$ = 8.0, $N_{\mathrm{dets}}$ = 2e+04 (16 sites, 26 electrons), $N_{\mathrm{plat}}$ = 4.77e+04 ± 6.4 %

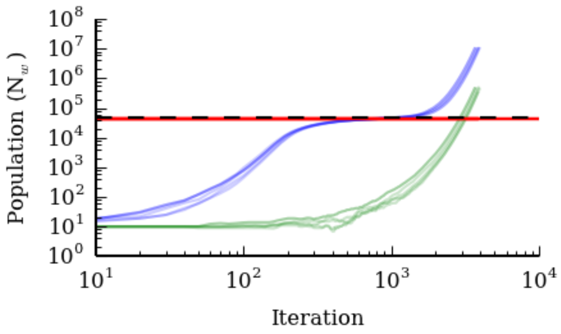


FIG. 350. $U$ = 8.0, $N_{\mathrm{dets}}$ = 2e+04 (16 sites, 6 electrons), $N_{\mathrm{plat}}$ = 4.52e+04 ± 9.8 %

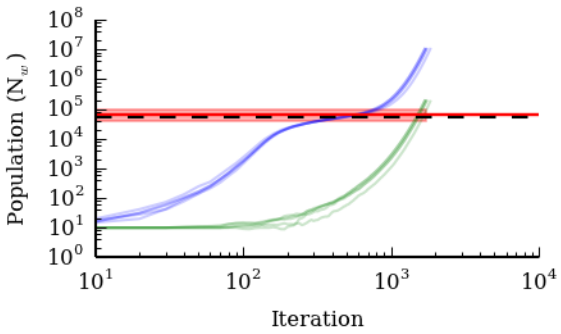


FIG. 351. $U$ = 8.0, $N_{\mathrm{dets}}$ = 2e+04 (12 sites, 8 electrons), $N_{\mathrm{plat}}$ = 6.64e+04 ± 43 % (manual correction: 6e+04)

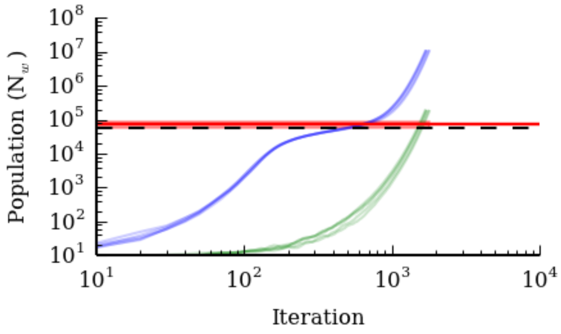


FIG. 352. $U$ = 8.0, $N_{\mathrm{dets}}$ = 2e+04 (12 sites, 16 electrons), $N_{\mathrm{plat}}$ = 7.41e+04 ± 23 %

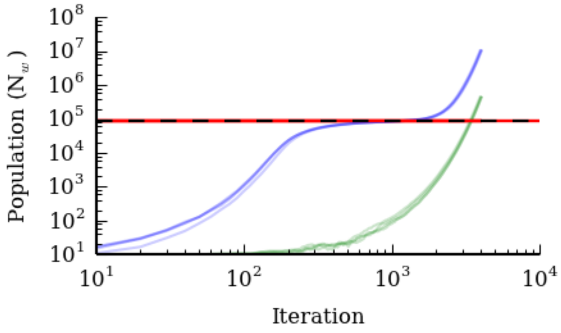


FIG. 353. $U$ = 8.0, $N_{\mathrm{dets}}$ = 3.7e+04 (18 sites, 30 electrons), $N_{\mathrm{plat}}$ = 8.79e+04 ± 5.6 %

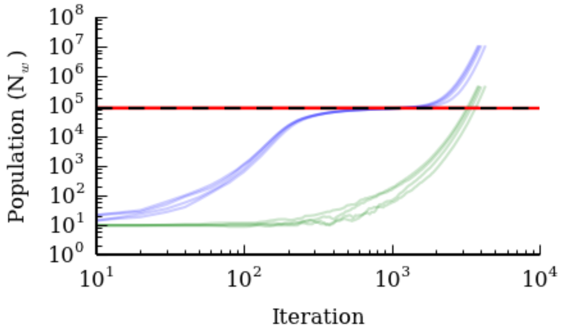


FIG. 354. $U$ = 8.0, $N_{\mathrm{dets}}$ = 3.7e+04 (18 sites, 6 electrons), $N_{\mathrm{plat}}$ = 8.97e+04 ± 2.7 %

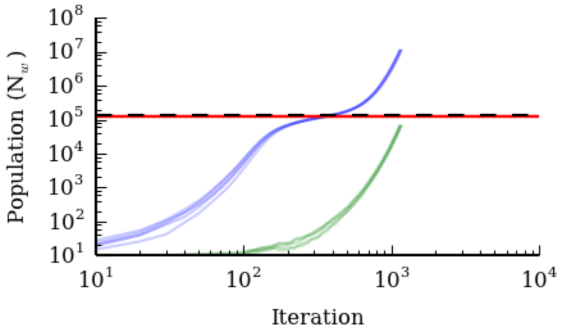


FIG. 355. $U$ = 8.0, $N_{\rm dets}$ = 5.2e+04 (12 sites, 10 electrons), $N_{\rm plat}$ = 1.25e+05 ± 0.6 %

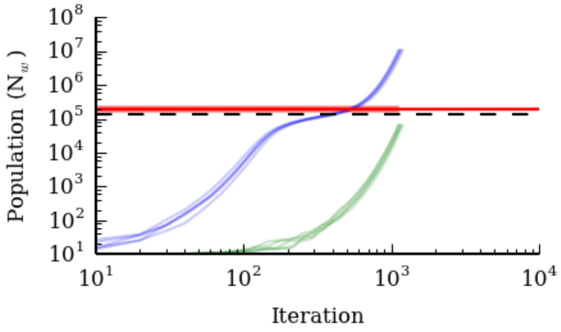


FIG. 356. $U$ = 8.0, $N_{\rm dets}$ = 5.2e+04 (12 sites, 14 electrons), $N_{\rm plat}$ = 1.96e+05 ± 20 %

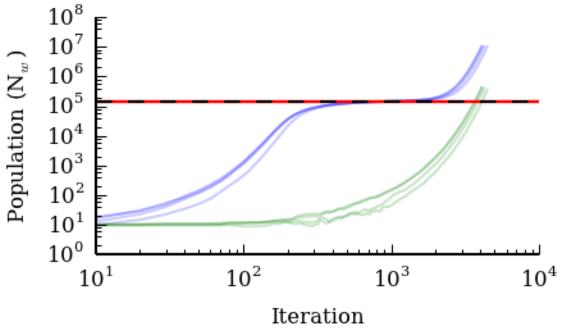


FIG. 357. $U$ = 8.0, $N_{\rm dets}$ = 6.5e+04 (20 sites, 34 electrons), $N_{\rm plat}$ = 1.42e+05 ± 3.6 %

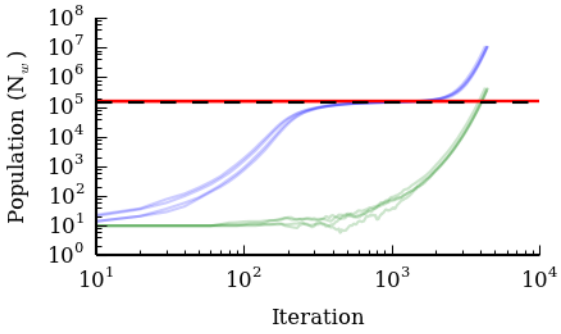


FIG. 358. $U$ = 8.0, $N_{\rm dets}$ = 6.5e+04 (20 sites, 6 electrons), $N_{\rm plat}$ = 1.52e+05 ± 3.8 %

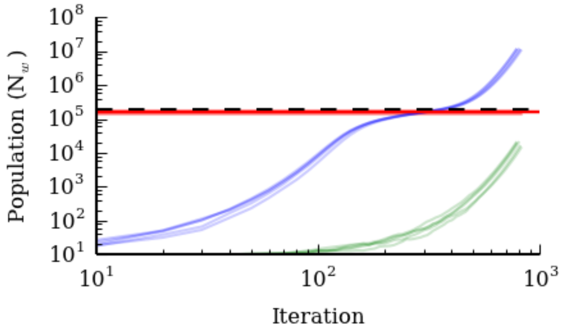


FIG. 359. $U$ = 8.0, $N_{\rm dets}$ = 7.1e+04 (12 sites, 12 electrons), $N_{\rm plat}$ = 1.55e+05 ± 10 %

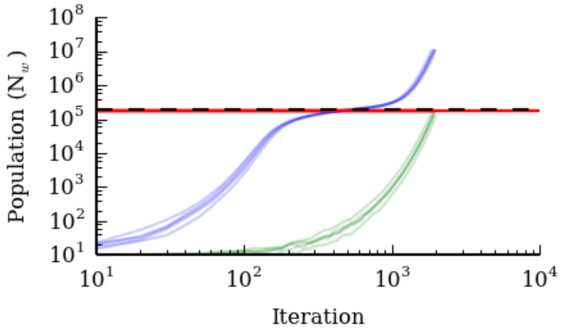


FIG. 360. $U$ = 8.0, $N_{\rm dets}$ = 7.2e+04 (14 sites, 8 electrons), $N_{\rm plat}$ = 1.77e+05 ± 11 %

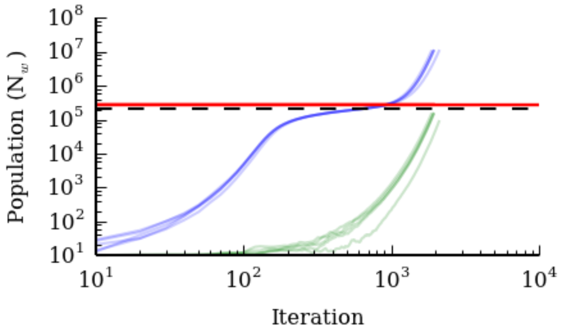


FIG. 361. $U$ = 8.0, $N_{\rm dets}$ = 7.2e+04 (14 sites, 20 electrons), $N_{\rm plat}$ = 2.81e+05 ± 5.6 %

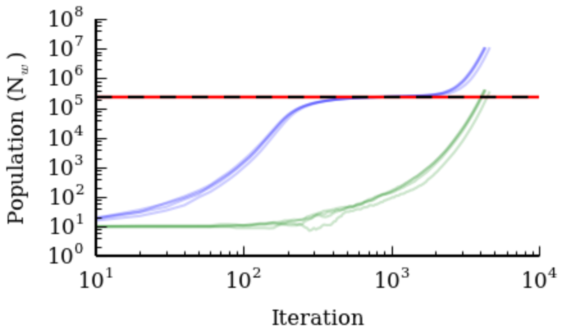


FIG. 362. $U$ = 8.0, $N_{\rm dets}$ = 1.1e+05 (22 sites, 38 electrons), $N_{\rm plat}$ = 2.4e+05 ± 0.37 %

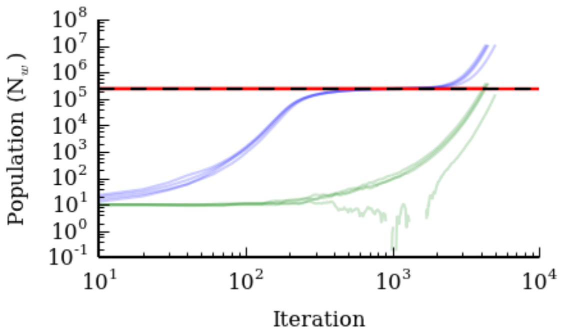


FIG. 363. $U$ = 8.0, $N_{\rm dets}$ = 1.1e+05 (22 sites, 6 electrons), $N_{\rm plat}$ = 2.51e+05 ± 2.2 %

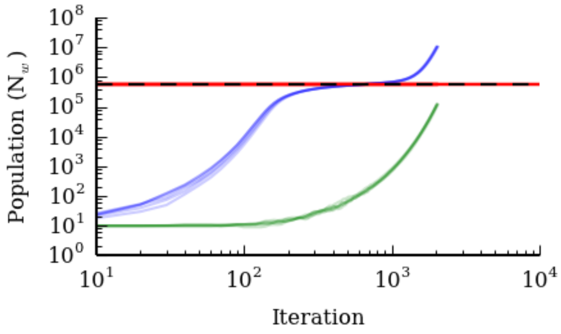


FIG. 364. $U$ = 8.0, $N_{\rm dets}$ = 2.1e+05 (16 sites, 8 electrons), $N_{\rm plat}$ = 5.67e+05 ± 11 %

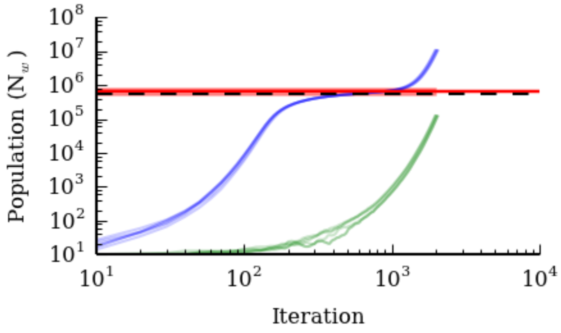


FIG. 365. $U$ = 8.0, $N_{\rm dets}$ = 2.1e+05 (16 sites, 24 electrons), $N_{\rm plat}$ = 6.3e+05 ± 19 %

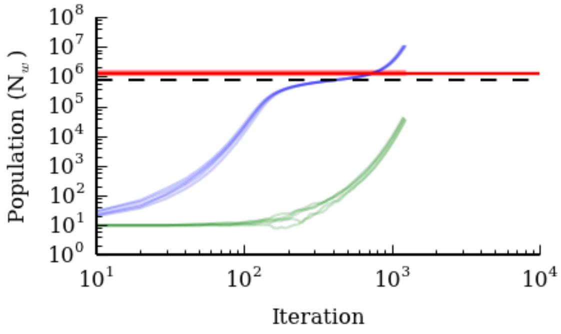


FIG. 366. $U$ = 8.0, $N_{\rm dets}$ = 2.9e+05 (14 sites, 18 electrons), $N_{\rm plat}$ = 1.33e+06 ± 13 %

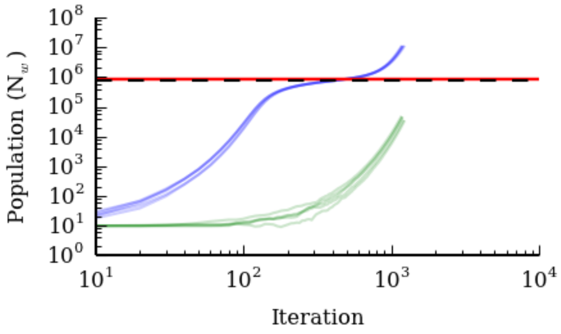


FIG. 367. $U$ = 8.0, $N_{\rm dets}$ = 2.9e+05 (14 sites, 10 electrons), $N_{\rm plat}$ = 8.91e+05 ± 0 %

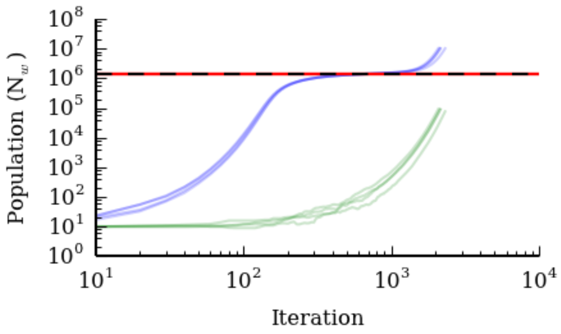


FIG. 368. $U$ = 8.0, $N_{\rm dets}$ = 5.2e+05 (18 sites, 8 electrons), $N_{\rm plat}$ = 1.41e+06 ± 0 %

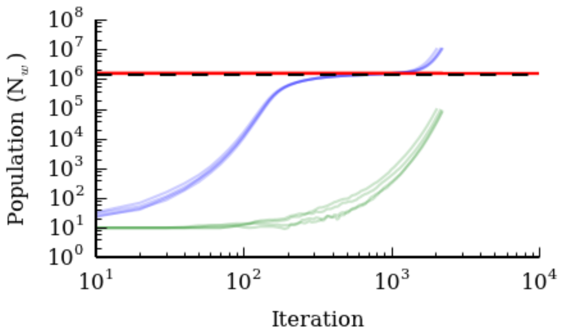


FIG. 369. $U$ = 8.0, $N_{\rm dets}$ = 5.2e+05 (18 sites, 28 electrons), $N_{\rm plat}$ = 1.62e+06 ± 2.6 %

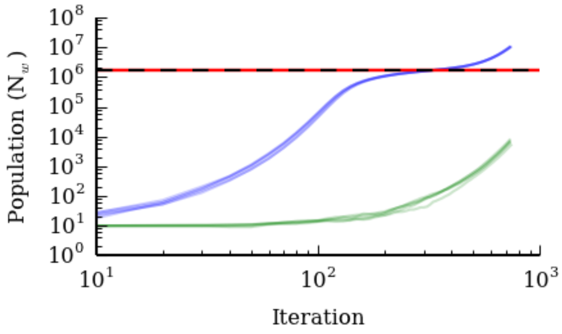


FIG. 370. $U$ = 8.0, $N_{\rm dets}$ = 6.4e+05 (14 sites, 16 electrons), $N_{\rm plat}$ = 1.78e+06 ± 0 %

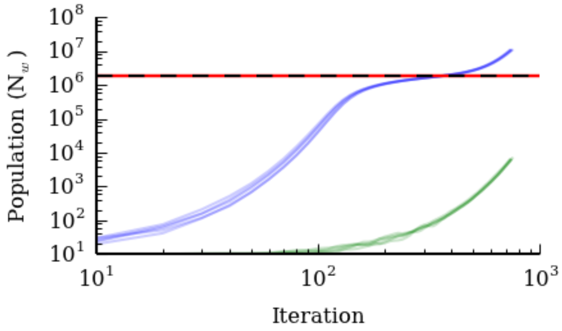


FIG. 371. $U$ = 8.0, $N_{\rm dets}$ = 6.4e+05 (14 sites, 12 electrons), $N_{\rm plat}$ = 1.78e+06 ± 0 %

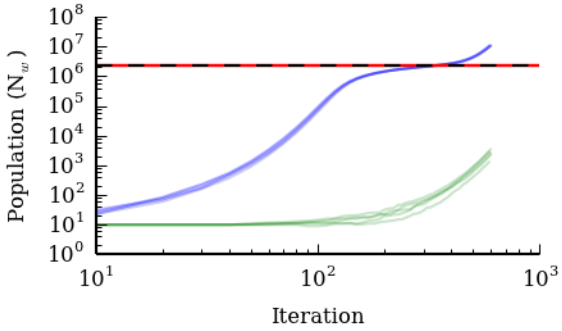


FIG. 372. $U$ = 8.0, $N_{\rm dets}$ = 8.4e+05 (14 sites, 14 electrons), $N_{\rm plat}$ = 2.24e+06 ± 0 %

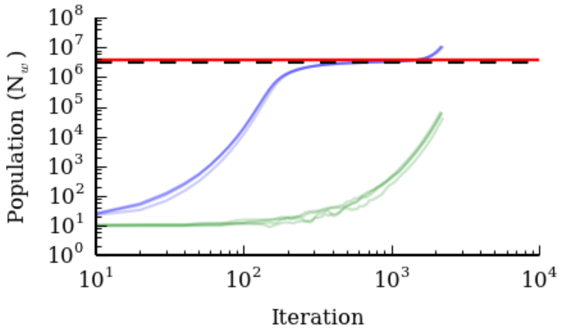


FIG. 373. $U$ = 8.0, $N_{\mathrm{dets}}$ = 1.2e+06 (20 sites, 32 electrons), $N_{\mathrm{plat}}$ = 3.86e+06 ± 0.016 %

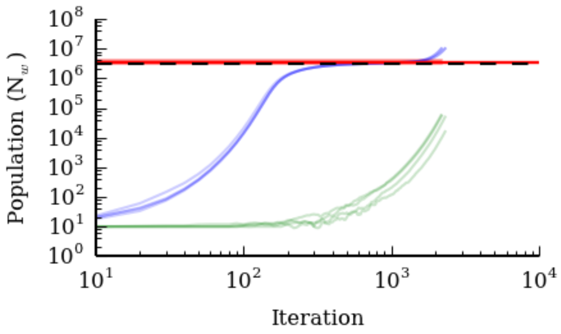


FIG. 374. $U$ = 8.0, $N_{\mathrm{dets}}$ = 1.2e+06 (20 sites, 8 electrons), $N_{\mathrm{plat}}$ = 3.61e+06 ± 12 %

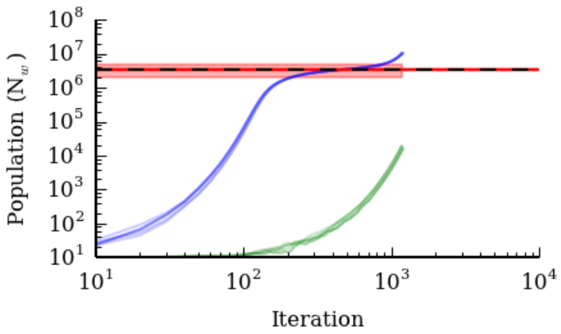


FIG. 375. $U$ = 8.0, $N_{\mathrm{dets}}$ = 1.2e+06 (16 sites, 10 electrons), $N_{\mathrm{plat}}$ = 3.51e+06 ± 42 % (manual correction: 4e+06)

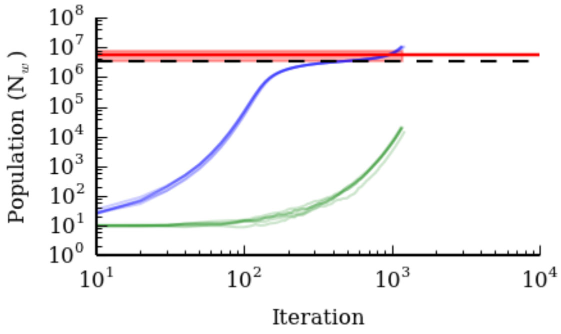


FIG. 376. $U$ = 8.0, $N_{\mathrm{dets}}$ = 1.2e+06 (16 sites, 22 electrons), $N_{\mathrm{plat}}$ = 5.46e+06 ± 35 %

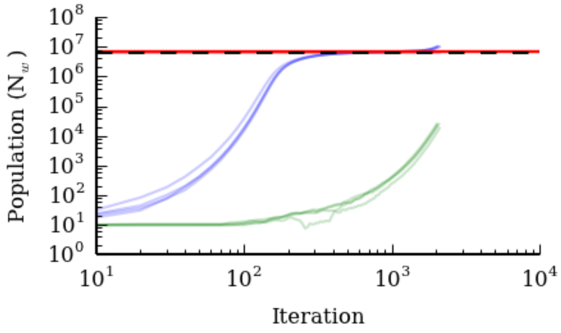


FIG. 377. $U$ = 8.0, $N_{\mathrm{dets}}$ = 2.4e+06 (22 sites, 8 electrons), $N_{\mathrm{plat}}$ = 6.76e+06 ± 6.5 %

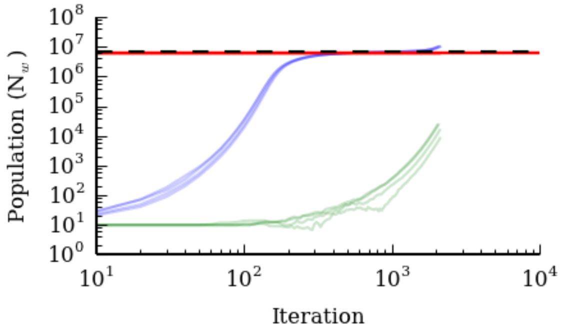


FIG. 378. $U$ = 8.0, $N_{\mathrm{dets}}$ = 2.4e+06 (22 sites, 36 electrons), $N_{\mathrm{plat}}$ = 5.95e+06 ± 8.9 %
